# Supplementary material for: Southern class I methanol masers at 36 and 44 GHz
Source: arXiv:1401.5179 ancillary file (2014-01-21)
Supplement: Supplementary file 2 [file fulltable3.pdf]

**Table 3.** Fit results for individual gaussian components. The uncertainties are given in parentheses and expressed in units of the least significant figure.

| Source name  | Location     | Frequency<br>(GHz) | LSR velocity<br>(km s <sup>-1</sup> ) | $\alpha_{2000}$<br>(h:m:s) | $\delta_{2000}$<br>( $^{\circ}$ :arcmin:arcsec) | Line FWHM<br>(km s <sup>-1</sup> ) | Flux density<br>(Jy) |          |
|--------------|--------------|--------------------|---------------------------------------|----------------------------|-------------------------------------------------|------------------------------------|----------------------|----------|
| G269.15-1.13 | A            | 36                 | +8.6 (2)                              | 09:03:33.4 (1)             | -48:28:01.9 (5)                                 | 1.4 (3)                            | 0.41 (2)             |          |
|              |              |                    | +8.77 (5)                             | 09:03:33.41 (5)            | -48:28:01.6 (3)                                 | 0.50 (9)                           | 0.47 (8)             |          |
|              |              |                    | +9.53 (3)                             | 09:03:33.46 (6)            | -48:28:02.8 (3)                                 | 0.8 (1)                            | 1.4 (1)              |          |
|              |              |                    | +10.4 (1)                             | 09:03:33.35 (6)            | -48:28:01.4 (3)                                 | 0.8 (2)                            | 0.47 (8)             |          |
|              |              | 44                 | +7.552 (5)                            | 09:03:33.46 (2)            | -48:28:01.45 (9)                                | 0.18 (1)                           | 1.49 (9)             |          |
|              |              |                    | +9.02 (8)                             | 09:03:33.30 (8)            | -48:28:02.6 (3)                                 | 2.2 (1)                            | 0.71 (6)             |          |
|              |              |                    | +9.336 (2)                            | 09:03:33.523 (8)           | -48:28:04.44 (4)                                | 0.465 (4)                          | 10.77 (8)            |          |
|              |              |                    | +9.99 (1)                             | 09:03:33.48 (3)            | -48:28:01.7 (2)                                 | 0.22 (3)                           | 0.76 (9)             |          |
|              | B            | 36                 | +10.66 (4)                            | 09:03:33.07 (8)            | -48:27:55.1 (4)                                 | 0.6 (2)                            | 0.6 (3)              |          |
|              |              |                    | +11.2 (3)                             | 09:03:33.0 (1)             | -48:27:55.7 (6)                                 | 1.2 (3)                            | 0.4 (1)              |          |
|              |              | 44                 | +9.70 (8)                             | 09:03:33.07 (5)            | -48:27:55.0 (3)                                 | 0.8 (1)                            | 1.0 (1)              |          |
|              |              |                    | +10.461 (6)                           | 09:03:33.020 (8)           | -48:27:54.97 (4)                                | 0.27 (2)                           | 2.5 (2)              |          |
|              |              |                    | +10.62 (2)                            | 09:03:33.05 (2)            | -48:27:54.8 (1)                                 | 0.88 (3)                           | 4.7 (2)              |          |
|              |              |                    | +12.01 (1)                            | 09:03:32.85 (3)            | -48:27:57.8 (2)                                 | 0.38 (3)                           | 1.16 (8)             |          |
|              |              | C                  | 44                                    | +9.272 (6)                 | 09:03:29.13 (3)                                 | -48:28:23.5 (2)                    | 0.27 (2)             | 11.5 (6) |
|              |              |                    |                                       | +10.6 (1)                  | 09:03:29.13 (9)                                 | -48:28:24.4 (5)                    | 1.7 (3)              | 1.6 (2)  |
|              | D            | 44                 | +13.27 (1)                            | 09:03:35.20 (4)            | -48:28:20.4 (2)                                 | 0.36 (3)                           | 0.94 (8)             |          |
|              | E            | 36                 | +11.00 (5)                            | 09:03:32.58 (6)            | -48:28:19.9 (3)                                 | 1.4 (1)                            | 0.42 (3)             |          |
|              | F            | 36                 | +10.15 (2)                            | 09:03:34.70 (9)            | -48:28:02.2 (4)                                 | 0.64 (5)                           | 0.49 (4)             |          |
|              | G270.26+0.84 | A                  | 36                                    | +9.751 (4)                 | 09:16:40.57 (1)                                 | -47:56:23.48 (6)                   | 0.209 (8)            | 5.1 (1)  |
| +9.98 (1)    |              |                    |                                       | 09:16:40.47 (6)            | -47:56:23.4 (3)                                 | 0.19 (3)                           | 1.3 (1)              |          |
| +10.6 (1)    |              |                    |                                       | 09:16:40.3 (1)             | -47:56:21.1 (7)                                 | 1.5 (2)                            | 0.31 (3)             |          |
| 44           |              |                    |                                       | +9.512 (2)                 | 09:16:40.560 (1)                                | -47:56:23.861 (8)                  | 0.243 (4)            | 42 (2)   |
|              |              |                    | +9.72 (2)                             | 09:16:40.57 (1)            | -47:56:23.78 (8)                                | 0.38 (2)                           | 15.9 (9)             |          |
|              |              |                    | +9.7 (2)                              | 09:16:40.49 (9)            | -47:56:23.2 (4)                                 | 2.9 (5)                            | 0.38 (8)             |          |
|              |              |                    | +11.58 (2)                            | 09:16:40.17 (3)            | -47:56:23.3 (2)                                 | 0.47 (8)                           | 1.0 (1)              |          |
| B            |              |                    | 36                                    | +8.90 (3)                  | 09:16:40.62 (6)                                 | -47:56:09.9 (3)                    | 0.52 (8)             | 0.64 (8) |
|              |              |                    |                                       | +9.47 (2)                  | 09:16:40.48 (5)                                 | -47:56:09.3 (3)                    | 0.28 (8)             | 0.6 (2)  |
|              |              |                    | 44                                    | +10.16 (3)                 | 09:16:40.60 (8)                                 | -47:56:09.5 (3)                    | 1.1 (1)              | 2.60 (5) |
|              |              |                    |                                       | +10.78 (3)                 | 09:16:40.68 (8)                                 | -47:56:10.1 (4)                    | 0.3 (1)              | 0.4 (1)  |
| C            |              |                    | 44                                    | +11.2 (1)                  | 09:16:40.64 (8)                                 | -47:56:09.2 (4)                    | 0.9 (1)              | 1.0 (1)  |
|              |              | +8.367 (3)         |                                       | 09:16:40.95 (1)            | -47:56:08.26 (8)                                | 0.280 (6)                          | 8.2 (2)              |          |
|              |              | +9.13 (8)          |                                       | 09:16:40.89 (8)            | -47:56:09.2 (4)                                 | 1.5 (1)                            | 1.80 (6)             |          |
|              |              | +9.84 (1)          |                                       | 09:16:40.82 (3)            | -47:56:09.7 (1)                                 | 0.37 (3)                           | 3.1 (2)              |          |
|              |              | D                  | 36                                    | +10.438 (4)                | 09:16:40.86 (2)                                 | -47:56:09.6 (1)                    | 0.55 (1)             | 9.7 (2)  |
|              |              |                    |                                       | +11.332 (7)                | 09:16:40.92 (4)                                 | -47:56:10.6 (2)                    | 0.38 (2)             | 3.3 (1)  |
|              |              |                    | 44                                    | +11.33 (1)                 | 09:16:41.54 (6)                                 | -47:56:15.5 (3)                    | 0.41 (3)             | 2.5 (2)  |
|              |              |                    |                                       | 36                         | +9.84 (5)                                       | 09:16:40.75 (8)                    | -47:56:11.0 (8)      | 0.6 (1)  |
|              |              | E                  | 36                                    |                            | +10.90 (4)                                      | 09:16:40.80 (9)                    | -47:56:13.9 (5)      | 1.2 (1)  |
|              |              |                    |                                       | +12.25 (5)                 | 09:16:40.55 (8)                                 | -47:56:15.7 (3)                    | 0.7 (2)              | 0.4 (1)  |
|              |              |                    | 44                                    | +13 (1)                    | 09:16:40.81 (8)                                 | -47:56:15.0 (4)                    | 4 (3)                | 0.20 (3) |
|              |              |                    |                                       | +17.2 (1)                  | 09:16:40.71 (8)                                 | -47:56:15.0 (3)                    | 1.7 (3)              | 0.32 (4) |
| F            |              | 36                 | +10.37 (9)                            | 09:16:41.06 (4)            | -47:56:14.2 (3)                                 | 0.5 (1)                            | 2.2 (4)              |          |
|              |              |                    | +10.81 (8)                            | 09:16:40.81 (5)            | -47:56:15.5 (2)                                 | 0.47 (8)                           | 2.1 (6)              |          |
|              |              |                    | +9.42 (4)                             | 09:16:39.88 (5)            | -47:56:19.1 (3)                                 | 0.7 (1)                            | 0.54 (6)             |          |
|              |              |                    | +10.37 (2)                            | 09:16:39.94 (5)            | -47:56:18.8 (3)                                 | 0.66 (8)                           | 1.06 (8)             |          |
|              |              | G                  | 36                                    | +11.28 (2)                 | 09:16:39.88 (4)                                 | -47:56:18.3 (2)                    | 0.82 (4)             | 1.81 (8) |
|              |              |                    |                                       | +11.7 (3)                  | 09:16:39.9 (2)                                  | -47:56:19 (1)                      | 3.7 (4)              | 0.29 (5) |
| G            |              | 36                 | +7.47 (3)                             | 09:16:41.5 (1)             | -47:56:07.6 (5)                                 | 0.57 (6)                           | 0.64 (6)             |          |
|              | +19.53 (3)   |                    | 09:16:41.32 (4)                       | -47:56:20.8 (2)            | 1.03 (8)                                        | 0.74 (5)                           |                      |          |

**Table 3** – *continued*

| Source name  | Location | Frequency<br>(GHz) | LSR<br>velocity<br>(km s <sup>-1</sup> ) | $\alpha_{2000}$<br>(h:m:s) | $\delta_{2000}$<br>(°:arcmin:arcsec) | Line<br>FWHM<br>(km s <sup>-1</sup> ) | Flux<br>density<br>(Jy) |
|--------------|----------|--------------------|------------------------------------------|----------------------------|--------------------------------------|---------------------------------------|-------------------------|
| G294.98-1.73 | A        | 36                 | -7.928 (6)                               | 11:39:14.61 (4)            | -63:29:04.5 (2)                      | 0.28 (1)                              | 2.10 (9)                |
|              |          |                    | -7.3 (2)                                 | 11:39:14.4 (3)             | -63:29:05 (1)                        | 2.8 (3)                               | 0.27 (3)                |
|              |          | 44                 | -8.48 (2)                                | 11:39:14.40 (6)            | -63:29:04.4 (3)                      | 0.30 (3)                              | 3.7 (5)                 |
|              |          |                    | -8.4 (3)                                 | 11:39:14.3 (1)             | -63:29:05.5 (5)                      | 1.2 (3)                               | 1.1 (5)                 |
|              |          |                    | -8.19 (1)                                | 11:39:14.70 (3)            | -63:29:04.1 (2)                      | 0.35 (4)                              | 6.0 (8)                 |
|              | B        | 44                 | -7.61 (5)                                | 11:39:14.66 (8)            | -63:29:04.3 (3)                      | 0.4 (1)                               | 0.8 (5)                 |
|              |          |                    | -6.8 (1)                                 | 11:39:14.76 (8)            | -63:29:03.7 (4)                      | 1.0 (2)                               | 0.48 (6)                |
|              |          |                    | -9.50 (2)                                | 11:39:14.35 (4)            | -63:29:15.0 (2)                      | 0.84 (5)                              | 1.24 (6)                |
|              |          |                    | -8.359 (9)                               | 11:39:14.46 (4)            | -63:29:16.2 (2)                      | 0.56 (2)                              | 2.32 (8)                |
|              |          |                    | -0.66 (3)                                | 11:39:13.6 (1)             | -63:29:07.5 (5)                      | 0.44 (8)                              | 0.60 (8)                |
|              | C        | 36                 | -0.2 (1)                                 | 11:39:13.4 (3)             | -63:29:09 (1)                        | 4.6 (3)                               | 0.48 (5)                |
|              |          |                    | +0.52 (2)                                | 11:39:13.64 (3)            | -63:29:08.7 (1)                      | 0.70 (8)                              | 0.83 (8)                |
| G300.97+1.15 | A        | 36                 | -42.25 (1)                               | 12:34:52.84 (4)            | -61:39:55.6 (2)                      | 0.85 (3)                              | 1.22 (8)                |
|              |          |                    | -42.21 (1)                               | 12:34:52.762 (6)           | -61:39:55.49 (3)                     | 0.230 (9)                             | 15 (2)                  |
|              |          |                    | -42.076 (8)                              | 12:34:52.769 (4)           | -61:39:55.45 (2)                     | 0.215 (6)                             | 16 (2)                  |
|              |          | 44                 | -42.62 (5)                               | 12:34:52.84 (1)            | -61:39:55.39 (6)                     | 0.51 (5)                              | 4.0 (4)                 |
|              |          |                    | -42.355 (1)                              | 12:34:52.813 (1)           | -61:39:55.349 (6)                    | 0.309 (3)                             | 41 (1)                  |
|              | B        | 36                 | -41.877 (5)                              | 12:34:52.59 (1)            | -61:39:56.36 (8)                     | 0.20 (1)                              | 1.82 (9)                |
|              |          |                    | -45.78 (2)                               | 12:34:53.26 (8)            | -61:39:47.6 (5)                      | 0.18 (4)                              | 0.29 (5)                |
|              |          |                    | -46.035 (2)                              | 12:34:53.185 (9)           | -61:39:47.29 (6)                     | 0.291 (5)                             | 4.84 (8)                |
|              |          |                    | -43.84 (1)                               | 12:34:50.62 (2)            | -61:39:50.6 (1)                      | 0.42 (3)                              | 0.96 (6)                |
|              |          |                    | -42.68 (4)                               | 12:34:51.71 (8)            | -61:39:58.2 (4)                      | 1.2 (1)                               | 0.37 (2)                |
|              | C        | 44                 | -41.832 (9)                              | 12:34:51.78 (3)            | -61:39:58.9 (2)                      | 0.19 (2)                              | 1.05 (6)                |
|              |          |                    | -41.61 (2)                               | 12:34:51.91 (8)            | -61:39:58.9 (3)                      | 0.18 (4)                              | 0.45 (6)                |
|              |          |                    | -40.98 (5)                               | 12:34:51.65 (5)            | -61:39:58.2 (3)                      | 0.6 (2)                               | 0.19 (3)                |
|              |          |                    | -40.427 (4)                              | 12:34:51.68 (1)            | -61:39:58.81 (6)                     | 0.246 (8)                             | 1.73 (5)                |
|              |          |                    | -43.77 (2)                               | 12:34:51.73 (3)            | -61:39:58.9 (2)                      | 0.59 (4)                              | 0.75 (4)                |
|              | D        | 36                 | -42.99 (1)                               | 12:34:51.68 (8)            | -61:39:58.7 (5)                      | 0.37 (3)                              | 0.84 (5)                |
|              |          |                    | -42.092 (4)                              | 12:34:51.788 (6)           | -61:39:59.02 (4)                     | 0.15 (1)                              | 3.1 (6)                 |
|              |          |                    | -41.94 (1)                               | 12:34:51.81 (2)            | -61:39:59.0 (1)                      | 0.29 (2)                              | 5.1 (2)                 |
|              |          |                    | -41.42 (2)                               | 12:34:51.71 (2)            | -61:39:58.8 (2)                      | 0.64 (4)                              | 1.51 (4)                |
|              |          |                    | -40.656 (3)                              | 12:34:51.72 (1)            | -61:39:58.86 (8)                     | 0.268 (5)                             | 3.58 (6)                |
|              | E        | 44                 | -43.53 (1)                               | 12:34:53.84 (4)            | -61:40:03.4 (3)                      | 0.25 (2)                              | 0.81 (8)                |
|              |          |                    | -46.8 (2)                                | 12:34:54.3 (2)             | -61:39:59 (1)                        | 3.3 (4)                               | 0.13 (1)                |
|              |          |                    | -42.95 (2)                               | 12:34:53.99 (3)            | -61:39:57.3 (2)                      | 0.41 (4)                              | 0.75 (4)                |
|              |          |                    | -42.46 (1)                               | 12:34:53.94 (2)            | -61:39:57.2 (1)                      | 0.41 (3)                              | 1.10 (4)                |
|              |          |                    | -41.71 (2)                               | 12:34:54.52 (6)            | -61:39:56.2 (3)                      | 0.56 (5)                              | 0.46 (3)                |
|              | F        | 36                 | -43.303 (6)                              | 12:34:53.96 (1)            | -61:39:57.03 (8)                     | 0.42 (1)                              | 4.5 (1)                 |
|              |          |                    | -42.781 (7)                              | 12:34:54.00 (2)            | -61:39:56.9 (1)                      | 0.66 (2)                              | 6.33 (5)                |
|              |          |                    | -41.993 (6)                              | 12:34:54.54 (2)            | -61:39:55.8 (1)                      | 0.21 (2)                              | 1.6 (2)                 |
|              |          |                    | -41.71 (6)                               | 12:34:54.63 (9)            | -61:39:55.3 (7)                      | 0.55 (9)                              | 0.81 (6)                |
|              |          |                    | -42.26 (8)                               | 12:34:50.1 (1)             | -61:40:00.1 (6)                      | 1.4 (1)                               | 0.22 (2)                |
|              | G        | 44                 | -41.92 (2)                               | 12:34:50.12 (8)            | -61:39:59.0 (4)                      | 0.19 (6)                              | 0.21 (5)                |
|              |          |                    | -42.13 (1)                               | 12:34:50.05 (6)            | -61:39:58.9 (4)                      | 0.24 (3)                              | 0.67 (8)                |
|              |          |                    | -41.6 (1)                                | 12:34:50.0 (1)             | -61:39:59.6 (7)                      | 2.0 (2)                               | 0.24 (3)                |
| G301.14-0.23 | A        | 36                 | -36.5 (1)                                | 12:35:35.6 (1)             | -63:02:26.7 (6)                      | 2.3 (1)                               | 0.59 (4)                |
|              |          |                    | -36.24 (1)                               | 12:35:35.57 (2)            | -63:02:24.9 (1)                      | 0.40 (2)                              | 2.0 (2)                 |
|              |          |                    | -35.58 (9)                               | 12:35:35.60 (2)            | -63:02:24.96 (8)                     | 0.8 (2)                               | 2.1 (2)                 |

Table 3 – continued

| Source name                 | Location     | Frequency   | LSR velocity          | $\alpha_{2000}$   | $\delta_{2000}$                | Line FWHM             | Flux density     |                  |
|-----------------------------|--------------|-------------|-----------------------|-------------------|--------------------------------|-----------------------|------------------|------------------|
|                             |              | (GHz)       | (km s <sup>-1</sup> ) | (h:m:s)           | ( <sup>o</sup> :arcmin:arcsec) | (km s <sup>-1</sup> ) | (Jy)             |                  |
| G301.14-0.23<br>(continued) | A            | 36          | -35.289 (8)           | 12:35:35.609 (3)  | -63:02:24.87 (2)               | 0.30 (2)              | 4.5 (6)          |                  |
|                             |              |             | -34.995 (9)           | 12:35:35.624 (7)  | -63:02:25.01 (4)               | 0.32 (2)              | 4.5 (5)          |                  |
|                             |              | 44          | -37.06 (4)            | 12:35:35.71 (3)   | -63:02:26.6 (2)                | 1.09 (6)              | 4.0 (1)          |                  |
|                             |              |             | -36.578 (3)           | 12:35:35.62 (1)   | -63:02:24.90 (8)               | 0.438 (5)             | 37.5 (7)         |                  |
|                             |              |             | -36.130 (3)           | 12:35:35.581 (2)  | -63:02:24.76 (2)               | 0.494 (7)             | 43.2 (2)         |                  |
|                             |              |             | -35.544 (1)           | 12:35:35.670 (1)  | -63:02:24.821 (8)              | 0.406 (3)             | 67.2 (2)         |                  |
|                             | B            | 36          | -35.176 (3)           | 12:35:35.675 (3)  | -63:02:24.90 (2)               | 0.351 (4)             | 26.7 (4)         |                  |
|                             |              |             | -38 (2)               | 12:35:35.07 (5)   | -63:02:31.8 (4)                | 3 (2)                 | -0.7 (9)         |                  |
|                             |              | 44          | -34.34 (8)            | 12:35:34.98 (5)   | -63:02:32.0 (2)                | 0.8 (2)               | 0.33 (8)         |                  |
|                             |              |             | -39.6 (2)             | 12:35:35.11 (2)   | -63:02:32.1 (1)                | 2.9 (4)               | -1.10 (8)        |                  |
|                             |              |             | -38.0 (1)             | 12:35:35.04 (6)   | -63:02:32.5 (4)                | 1.1 (6)               | -0.4 (2)         |                  |
|                             |              |             | -34.54 (8)            | 12:35:35.09 (2)   | -63:02:32.3 (2)                | 0.9 (2)               | 0.6 (1)          |                  |
|                             | G305.21+0.21 | A           | 36                    | -45.840 (8)       | 13:11:13.68 (3)                | -62:34:34.8 (2)       | 0.38 (2)         | 1.11 (5)         |
|                             |              |             | 44                    | -46.041 (2)       | 13:11:13.743 (6)               | -62:34:34.85 (4)      | 0.348 (5)        | 6.28 (8)         |
| -43.9 (1)                   |              |             |                       | 13:11:13.7 (1)    | -62:34:35.0 (9)                | 2.5 (4)               | 0.27 (4)         |                  |
| -43.776 (7)                 |              |             |                       | 13:11:13.65 (3)   | -62:34:34.9 (2)                | 0.18 (2)              | 1.4 (1)          |                  |
| B                           |              | 36          | -40.1 (1)             | 13:11:14.0 (1)    | -62:34:40.7 (7)                | 2.6 (2)               | 0.26 (2)         |                  |
|                             |              | 44          | -41.61 (2)            | 13:11:14.03 (4)   | -62:34:37.6 (3)                | 0.50 (6)              | 0.78 (8)         |                  |
| -40.6 (2)                   |              |             | 13:11:13.9 (2)        | -62:34:40.3 (9)   | 3.6 (5)                        | 0.21 (3)              |                  |                  |
| C                           |              | 44          | -45.755 (6)           | 13:11:15.04 (2)   | -62:34:45.7 (1)                | 0.26 (1)              | 3.0 (1)          |                  |
| D                           |              | 36          | -39.801 (4)           | 13:11:14.04 (1)   | -62:34:46.39 (8)               | 0.46 (1)              | 2.57 (5)         |                  |
|                             |              |             | -37.9 (3)             | 13:11:13.6 (1)    | -62:34:49.8 (8)                | 3.9 (6)               | 0.14 (2)         |                  |
|                             |              | 44          | -43.44 (8)            | 13:11:13.53 (8)   | -62:34:50.3 (4)                | 0.9 (2)               | 0.28 (4)         |                  |
|                             |              |             | -40.024 (2)           | 13:11:14.066 (7)  | -62:34:46.71 (4)               | 0.483 (4)             | 7.71 (6)         |                  |
|                             |              | -37.78 (4)  | 13:11:13.59 (3)       | -62:34:50.1 (2)   | 0.8 (1)                        | 0.51 (5)              |                  |                  |
|                             |              | -36.45 (4)  | 13:11:13.60 (4)       | -62:34:51.1 (2)   | 0.8 (1)                        | 0.47 (5)              |                  |                  |
|                             |              | E           | 44                    | -45.15 (3)        | 13:11:16.19 (8)                | -62:34:51.0 (5)       | 0.69 (6)         | 2.0 (1)          |
|                             |              |             |                       | F                 | 36                             | -42.267 (1)           | 13:11:10.822 (3) | -62:34:38.12 (2) |
|                             |              | 44          | -43.8 (2)             |                   | 13:11:10.88 (8)                | -62:34:39.0 (4)       | 0.5 (3)          | 0.24 (8)         |
|                             |              |             | -43.37 (2)            | 13:11:10.84 (2)   | -62:34:38.9 (1)                | 0.33 (4)              | 1.2 (2)          |                  |
|                             |              | -42.804 (2) | 13:11:10.898 (5)      | -62:34:38.40 (3)  | 0.234 (6)                      | 19 (1)                |                  |                  |
|                             |              | -42.547 (6) | 13:11:10.888 (1)      | -62:34:38.420 (5) | 0.41 (1)                       | 77 (3)                |                  |                  |
|                             |              | -42.26 (2)  | 13:11:10.901 (5)      | -62:34:38.39 (3)  | 0.42 (1)                       | 35 (3)                |                  |                  |
|                             |              | -41.60 (1)  | 13:11:11.03 (3)       | -62:34:37.8 (2)   | 0.23 (4)                       | 0.63 (8)              |                  |                  |
|                             |              | -41.14 (3)  | 13:11:10.90 (5)       | -62:34:38.1 (3)   | 0.29 (6)                       | 0.57 (8)              |                  |                  |
|                             |              | -40.72 (1)  | 13:11:10.94 (2)       | -62:34:38.2 (1)   | 0.40 (3)                       | 1.47 (6)              |                  |                  |
|                             |              | -39.81 (4)  | 13:11:10.57 (8)       | -62:34:42.5 (4)   | 0.39 (9)                       | 0.28 (6)              |                  |                  |
| G                           |              | 44          | -41.43 (2)            | 13:11:13.50 (4)   | -62:34:53.3 (2)                | 0.75 (4)              | 1.12 (5)         |                  |
|                             |              |             | -38.75 (1)            | 13:11:13.84 (2)   | -62:34:55.9 (1)                | 0.43 (3)              | 1.32 (8)         |                  |
| H                           |              | 36          | -40.63 (3)            | 13:11:05.95 (6)   | -62:34:50.0 (4)                | 1.00 (6)              | 0.53 (3)         |                  |
|                             |              | 44          | -40.97 (5)            | 13:11:05.92 (6)   | -62:34:50.7 (3)                | 1.14 (9)              | 0.60 (5)         |                  |
| -40.650 (5)                 |              |             | 13:11:06.04 (2)       | -62:34:50.2 (1)   | 0.25 (1)                       | 1.98 (9)              |                  |                  |
| I                           |              | 44          | -40.972 (1)           | 13:11:05.074 (6)  | -62:34:49.62 (4)               | 0.281 (2)             | 12.9 (1)         |                  |
| J                           |              | 44          | -41.18 (1)            | 13:11:08.71 (2)   | -62:34:45.4 (2)                | 0.45 (3)              | 0.61 (4)         |                  |
| K                           |              | 36          | -40.78 (3)            | 13:11:08.3 (1)    | -62:34:52.6 (7)                | 0.33 (8)              | 0.26 (5)         |                  |
|                             |              |             | -40.07 (4)            | 13:11:08.23 (6)   | -62:34:53.2 (4)                | 1.0 (1)               | 0.40 (2)         |                  |
|                             |              | 44          | -41.10 (3)            | 13:11:08.36 (3)   | -62:34:52.9 (2)                | 0.61 (8)              | 0.73 (4)         |                  |
|                             |              |             | -40.35 (2)            | 13:11:08.35 (3)   | -62:34:53.1 (2)                | 0.67 (4)              | 1.42 (4)         |                  |
|                             |              |             | -43.83 (6)            | 13:11:15.6 (1)    | -62:34:42.3 (6)                | 1.2 (1)               | 0.39 (4)         |                  |

**Table 3** – *continued*

| Source name  | Location | Frequency<br>(GHz) | LSR<br>velocity<br>(km s <sup>-1</sup> ) | $\alpha_{2000}$<br>(h:m:s) | $\delta_{2000}$<br>(°:arcmin:arcsec) | Line<br>FWHM<br>(km s <sup>-1</sup> ) | Flux<br>density<br>(Jy) |
|--------------|----------|--------------------|------------------------------------------|----------------------------|--------------------------------------|---------------------------------------|-------------------------|
| G305.25+0.25 | A        | 36                 | -37.334 (4)                              | 13:11:32.45 (2)            | -62:32:07.9 (1)                      | 0.26 (1)                              | 3.0 (1)                 |
|              |          |                    | -37.3 (2)                                | 13:11:32.39 (3)            | -62:32:08.7 (2)                      | 1.5 (2)                               | 2.1 (3)                 |
|              |          |                    | -36.822 (3)                              | 13:11:32.297 (4)           | -62:32:08.24 (2)                     | 0.54 (1)                              | 15.3 (6)                |
|              |          |                    | -36.265 (3)                              | 13:11:32.54 (1)            | -62:32:09.21 (8)                     | 0.30 (2)                              | 5.4 (8)                 |
|              |          |                    | -36.02 (3)                               | 13:11:32.54 (3)            | -62:32:09.0 (1)                      | 0.62 (4)                              | 7.2 (5)                 |
|              |          |                    | -35.0 (2)                                | 13:11:32.33 (6)            | -62:32:06.0 (5)                      | 1.7 (4)                               | 0.32 (4)                |
|              |          | 44                 | -38.68 (2)                               | 13:11:32.44 (3)            | -62:32:08.7 (2)                      | 0.34 (3)                              | 2.3 (1)                 |
|              |          |                    | -38.31 (1)                               | 13:11:32.462 (9)           | -62:32:08.72 (6)                     | 0.33 (5)                              | 2.4 (4)                 |
|              |          |                    | -37.5 (1)                                | 13:11:32.40 (1)            | -62:32:08.29 (8)                     | 0.9 (2)                               | 14 (2)                  |
|              |          |                    | -37.418 (1)                              | 13:11:32.60 (2)            | -62:32:07.8 (1)                      | 0.214 (4)                             | 17.5 (5)                |
|              |          |                    | -37.039 (5)                              | 13:11:32.42 (1)            | -62:32:08.33 (8)                     | 0.54 (2)                              | 44 (6)                  |
|              |          |                    | -36.456 (2)                              | 13:11:32.58 (3)            | -62:32:09.1 (2)                      | 0.32 (1)                              | 17 (1)                  |
|              |          |                    | -36.28 (1)                               | 13:11:32.62 (3)            | -62:32:09.3 (2)                      | 0.724 (9)                             | 47.9 (8)                |
|              |          |                    | -35.68 (8)                               | 13:11:32.40 (8)            | -62:32:06.8 (6)                      | 1.2 (1)                               | 1.20 (3)                |
|              |          |                    | -37.11 (3)                               | 13:11:32.53 (6)            | -62:32:07.1 (5)                      | 1.18 (8)                              | 0.43 (2)                |
| G305.37+0.21 | A        | 36                 | -40.21 (1)                               | 13:12:30.36 (4)            | -62:34:08.0 (3)                      | 0.50 (3)                              | 1.9 (1)                 |
|              |          | 44                 | -40.79 (6)                               | 13:12:30.51 (8)            | -62:34:07.8 (5)                      | 1.10 (9)                              | 2.5 (4)                 |
|              |          |                    | -40.511 (5)                              | 13:12:30.465 (6)           | -62:34:07.55 (4)                     | 0.40 (2)                              | 11.5 (4)                |
|              | B        | 36                 | -42.32 (4)                               | 13:12:29.0 (2)             | -62:34:01.2 (8)                      | 0.65 (8)                              | 0.66 (8)                |
|              |          | 44                 | -42.50 (3)                               | 13:12:28.92 (4)            | -62:34:00.9 (3)                      | 0.56 (6)                              | 2.3 (2)                 |
|              | C        | 44                 | -38.48 (6)                               | 13:12:31.72 (6)            | -62:34:08.0 (4)                      | 2.1 (2)                               | 1.57 (9)                |
|              |          |                    | -36.77 (1)                               | 13:12:31.63 (2)            | -62:34:08.1 (1)                      | 0.48 (3)                              | 4.5 (2)                 |
|              |          |                    | -36.32 (2)                               | 13:12:31.54 (3)            | -62:34:07.4 (2)                      | 0.21 (5)                              | 1.5 (3)                 |
|              | CD       | 36                 | -37.55 (9)                               | 13:12:31.50 (9)            | -62:34:06.5 (6)                      | 3.4 (2)                               | 0.59 (4)                |
|              |          |                    | -37.20 (1)                               | 13:12:31.51 (4)            | -62:34:02.2 (3)                      | 0.50 (3)                              | 1.96 (8)                |
|              | D        | 44                 | -37.372 (3)                              | 13:12:31.51 (1)            | -62:34:01.69 (8)                     | 0.596 (7)                             | 11.3 (1)                |
|              | E        | 36                 | -36.57 (1)                               | 13:12:36.17 (3)            | -62:33:27.1 (2)                      | 0.27 (4)                              | 0.68 (8)                |
|              |          |                    | -36.27 (3)                               | 13:12:36.0 (1)             | -62:33:27.7 (6)                      | 1.59 (8)                              | 0.71 (6)                |
|              |          |                    | -36.18 (1)                               | 13:12:36.1 (1)             | -62:33:27.3 (7)                      | 0.29 (4)                              | 0.70 (8)                |
|              |          | 44                 | -36.82 (1)                               | 13:12:36.21 (2)            | -62:33:26.7 (1)                      | 0.31 (3)                              | 1.6 (1)                 |
|              |          |                    | -36.45 (1)                               | 13:12:36.12 (5)            | -62:33:27.3 (3)                      | 0.31 (3)                              | 1.8 (2)                 |
|              |          |                    | -36.28 (6)                               | 13:12:36.12 (9)            | -62:33:26.8 (5)                      | 1.7 (2)                               | 0.6 (2)                 |
|              |          |                    | -35.925 (7)                              | 13:12:36.46 (3)            | -62:33:25.2 (2)                      | 0.32 (2)                              | 1.8 (1)                 |
|              |          |                    | -35.1 (1)                                | 13:12:35.9 (1)             | -62:33:35.2 (7)                      | 2.3 (3)                               | 0.37 (4)                |
|              |          |                    | -35.047 (7)                              | 13:12:36.08 (9)            | -62:33:36.3 (6)                      | 0.27 (2)                              | 1.32 (8)                |
|              |          |                    | -33.80 (5)                               | 13:12:35.74 (4)            | -62:33:32.4 (3)                      | 0.57 (8)                              | 2.6 (2)                 |
|              |          |                    | -33.469 (2)                              | 13:12:35.554 (3)           | -62:33:32.04 (2)                     | 0.342 (3)                             | 23.9 (5)                |
|              |          | 44                 | -32.36 (6)                               | 13:12:35.9 (1)             | -62:33:33.7 (7)                      | 0.4 (1)                               | 0.5 (1)                 |
|              |          |                    | -31.85 (5)                               | 13:12:35.92 (6)            | -62:33:33.9 (4)                      | 0.63 (9)                              | 0.94 (6)                |
|              |          |                    | -36.45 (2)                               | 13:12:36.05 (6)            | -62:33:35.4 (4)                      | 0.76 (6)                              | 1.03 (8)                |
|              |          |                    | -35.314 (3)                              | 13:12:36.04 (4)            | -62:33:35.9 (3)                      | 0.459 (8)                             | 6.35 (9)                |
|              |          |                    | -34.38 (1)                               | 13:12:35.83 (6)            | -62:33:33.7 (4)                      | 0.51 (2)                              | 5.0 (1)                 |
|              |          |                    | -33.746 (1)                              | 13:12:35.609 (5)           | -62:33:31.82 (3)                     | 0.283 (3)                             | 35.0 (6)                |
|              |          |                    | -33.649 (5)                              | 13:12:35.715 (6)           | -62:33:31.68 (4)                     | 0.646 (8)                             | 25.8 (6)                |
|              |          |                    | -32.4 (3)                                | 13:12:35.903 (8)           | -62:33:32.99 (5)                     | 0.8 (3)                               | 3 (1)                   |
|              |          |                    | -31.94 (4)                               | 13:12:35.91 (2)            | -62:33:33.1 (1)                      | 0.57 (8)                              | 4 (3)                   |
|              | G        | 36                 | -34.99 (5)                               | 13:12:36.7 (2)             | -62:33:36 (1)                        | 0.27 (8)                              | 0.9 (2)                 |
|              |          |                    | -34.718 (6)                              | 13:12:36.819 (4)           | -62:33:37.47 (3)                     | 0.289 (8)                             | 8.2 (2)                 |

Table 3 – continued

| Source name                 | Location | Frequency<br>(GHz) | LSR<br>velocity<br>(km s <sup>-1</sup> ) | $\alpha_{2000}$<br>(h:m:s) | $\delta_{2000}$<br>(°:arcmin:arcsec) | Line<br>FWHM<br>(km s <sup>-1</sup> ) | Flux<br>density<br>(Jy) |
|-----------------------------|----------|--------------------|------------------------------------------|----------------------------|--------------------------------------|---------------------------------------|-------------------------|
| G305.37+0.21<br>(continued) | G        | 36                 | -33.66 (1)                               | 13:12:37.013 (7)           | -62:33:35.43 (5)                     | 0.59 (2)                              | 5.2 (3)                 |
|                             |          |                    | -33.608 (4)                              | 13:12:37.011 (4)           | -62:33:35.24 (3)                     | 0.20 (1)                              | 4.3 (3)                 |
|                             |          |                    | -33.107 (2)                              | 13:12:36.968 (2)           | -62:33:35.68 (1)                     | 0.212 (9)                             | 16 (2)                  |
|                             |          |                    | -32.995 (8)                              | 13:12:37.01 (2)            | -62:33:34.8 (2)                      | 0.336 (6)                             | 35 (2)                  |
|                             |          |                    | -32.49 (3)                               | 13:12:37.10 (8)            | -62:33:34.1 (7)                      | 0.38 (6)                              | 0.66 (6)                |
|                             |          |                    | -35.6 (1)                                | 13:12:36.85 (9)            | -62:33:37.5 (6)                      | 0.4 (3)                               | 0.6 (3)                 |
|                             |          |                    | -34.99 (2)                               | 13:12:36.87 (2)            | -62:33:37.4 (1)                      | 0.53 (5)                              | 12 (3)                  |
|                             |          |                    | -34.930 (3)                              | 13:12:36.850 (7)           | -62:33:37.33 (4)                     | 0.26 (1)                              | 22 (3)                  |
|                             |          |                    | -34.05 (2)                               | 13:12:37.082 (6)           | -62:33:35.56 (4)                     | 0.42 (3)                              | 18.7 (8)                |
|                             |          | 44                 | -33.808 (3)                              | 13:12:37.023 (2)           | -62:33:35.26 (2)                     | 0.259 (7)                             | 30 (2)                  |
|                             |          |                    | -33.262 (2)                              | 13:12:36.999 (2)           | -62:33:35.49 (2)                     | 0.404 (4)                             | 100 (4)                 |
|                             |          |                    | -33.0 (2)                                | 13:12:37.20 (2)            | -62:33:34.7 (1)                      | 0.7 (1)                               | 6 (2)                   |
|                             |          |                    | -31.57 (8)                               | 13:12:36.96 (6)            | -62:33:35.0 (5)                      | 0.6 (2)                               | 0.6 (1)                 |
|                             |          |                    | -32.61 (1)                               | 13:12:36.9 (1)             | -62:33:30.7 (8)                      | 0.56 (3)                              | 1.87 (5)                |
|                             |          |                    | -32.847 (5)                              | 13:12:36.95 (8)            | -62:33:30.0 (4)                      | 0.518 (9)                             | 9.0 (3)                 |
|                             |          |                    |                                          |                            |                                      |                                       |                         |
|                             |          |                    |                                          |                            |                                      |                                       |                         |
|                             |          |                    |                                          |                            |                                      |                                       |                         |
| G309.38-0.13                | A        | 36                 | -51.057 (5)                              | 13:47:24.86 (6)            | -62:18:06.3 (3)                      | 0.26 (1)                              | 1.32 (5)                |
|                             |          | 44                 | -51.294 (2)                              | 13:47:25.00 (1)            | -62:18:06.16 (8)                     | 0.391 (4)                             | 8.06 (6)                |
|                             | BE       | 36                 | -49.51 (4)                               | 13:47:24.6 (2)             | -62:18:07.8 (6)                      | 0.4 (1)                               | 0.28 (6)                |
|                             |          |                    | -82.89 (4)                               | 13:47:24.07 (4)            | -62:18:10.1 (2)                      | 1.72 (8)                              | 3.2 (1)                 |
|                             |          |                    | -82.860 (4)                              | 13:47:24.090 (4)           | -62:18:10.10 (2)                     | 0.36 (1)                              | 5.2 (1)                 |
|                             |          |                    | -81.27 (2)                               | 13:47:24.084 (4)           | -62:18:10.15 (2)                     | 1.26 (8)                              | 5.6 (5)                 |
|                             |          |                    | -79.6 (1)                                | 13:47:24.06 (2)            | -62:18:10.2 (1)                      | 2 (1)                                 | 1.44 (5)                |
|                             |          |                    | -78.60 (3)                               | 13:47:24.07 (1)            | -62:18:10.17 (8)                     | 0.5 (1)                               | 0.8 (3)                 |
|                             |          |                    | -77.62 (6)                               | 13:47:24.04 (2)            | -62:18:10.0 (1)                      | 0.9 (1)                               | 1.3 (3)                 |
|                             |          |                    | -72.6 (2)                                | 13:47:24.11 (6)            | -62:18:09.8 (4)                      | 4.8 (5)                               | 0.28 (3)                |
|                             |          |                    | -65.59 (5)                               | 13:47:24.06 (5)            | -62:18:08.6 (3)                      | 0.5 (1)                               | 0.36 (8)                |
|                             |          |                    | -50.489 (8)                              | 13:47:24.10 (3)            | -62:18:09.5 (2)                      | 0.38 (1)                              | 12.2 (4)                |
|                             |          |                    | -50.44 (3)                               | 13:47:24.1 (1)             | -62:18:09.4 (6)                      | 2.0 (1)                               | 1.7 (1)                 |
|                             |          |                    | -50.123 (9)                              | 13:47:24.114 (6)           | -62:18:09.08 (4)                     | 0.43 (1)                              | 12.7 (3)                |
|                             |          |                    | -48.98 (1)                               | 13:47:24.203 (9)           | -62:18:08.62 (5)                     | 0.28 (4)                              | 1.0 (1)                 |
|                             |          |                    | -82.91 (5)                               | 13:47:24.04 (8)            | -62:18:10.4 (5)                      | 0.5 (1)                               | 0.6 (1)                 |
|                             |          |                    | -81.5 (3)                                | 13:47:24.2 (1)             | -62:18:11.2 (6)                      | 3.2 (8)                               | 0.22 (8)                |
|                             |          |                    | -81.28 (9)                               | 13:47:24.02 (6)            | -62:18:10.1 (4)                      | 0.6 (3)                               | 0.3 (1)                 |
|                             |          |                    | -52.1 (2)                                | 13:47:24.14 (6)            | -62:18:09.5 (4)                      | 1.0 (3)                               | 1.0 (1)                 |
|                             |          |                    | -51.583 (7)                              | 13:47:24.14 (2)            | -62:18:09.4 (1)                      | 0.35 (3)                              | 4.0 (4)                 |
|                             |          |                    | -50.852 (1)                              | 13:47:24.126 (2)           | -62:18:09.31 (1)                     | 0.1875 (7)                            | 83.4 (3)                |
|                             |          |                    | -50.70 (2)                               | 13:47:24.142 (5)           | -62:18:09.15 (3)                     | 0.62 (5)                              | 29 (10)                 |
|                             |          |                    | -50.3 (3)                                | 13:47:24.13 (1)            | -62:18:09.11 (8)                     | 0.8 (3)                               | 11 (8)                  |
|                             |          |                    | -49.23 (1)                               | 13:47:24.211 (7)           | -62:18:08.70 (5)                     | 0.53 (2)                              | 4.7 (1)                 |
|                             | C        | 36                 | -48.83 (2)                               | 13:47:24.07 (9)            | -62:18:02.0 (5)                      | 0.33 (4)                              | 0.49 (5)                |
|                             |          |                    | -47.8 (2)                                | 13:47:24.0 (1)             | -62:18:01.6 (8)                      | 2.6 (4)                               | 0.15 (2)                |
|                             |          | 44                 | -48.98 (1)                               | 13:47:24.10 (1)            | -62:18:01.14 (8)                     | 0.53 (3)                              | 1.91 (8)                |
|                             |          |                    | -47.8 (1)                                | 13:47:24.05 (8)            | -62:18:02.1 (5)                      | 1.6 (3)                               | 0.43 (4)                |
|                             | D        | 44                 | -49.55 (2)                               | 13:47:22.92 (2)            | -62:17:51.8 (1)                      | 0.59 (5)                              | 1.27 (8)                |
|                             | F        | 36                 | -53.78 (5)                               | 13:47:20.90 (5)            | -62:18:05.1 (3)                      | 0.3 (1)                               | 0.27 (8)                |
|                             |          |                    | -51.2 (2)                                | 13:47:20.8 (1)             | -62:18:04.7 (7)                      | 4.5 (3)                               | 0.7 (1)                 |
|                             |          |                    | -51.09 (1)                               | 13:47:20.68 (5)            | -62:18:04.6 (3)                      | 1.34 (4)                              | 3.0 (1)                 |
|                             |          |                    | -49.67 (1)                               | 13:47:20.81 (5)            | -62:18:03.8 (3)                      | 0.49 (4)                              | 1.29 (9)                |

**Table 3** – *continued*

| Source name                        | Location     | Frequency<br>(GHz) | LSR velocity<br>(km s <sup>-1</sup> ) | $\alpha_{2000}$<br>(h:m:s) | $\delta_{2000}$<br>( $^{\circ}$ :arcmin:arcsec) | Line FWHM<br>(km s <sup>-1</sup> ) | Flux density<br>(Jy) |          |          |
|------------------------------------|--------------|--------------------|---------------------------------------|----------------------------|-------------------------------------------------|------------------------------------|----------------------|----------|----------|
| G309.38-0.13<br><i>(continued)</i> | F            | 36                 | -48.65 (5)                            | 13:47:20.71 (4)            | -62:18:07.4 (2)                                 | 0.7 (2)                            | 0.38 (8)             |          |          |
|                                    |              | 44                 | -51.68 (8)                            | 13:47:20.60 (6)            | -62:18:05.4 (4)                                 | 1.9 (2)                            | 0.83 (8)             |          |          |
|                                    | G            |                    | -49.43 (8)                            | 13:47:20.43 (8)            | -62:18:05.0 (5)                                 | 1.1 (2)                            | 0.62 (8)             |          |          |
|                                    |              | 36                 | -60.57 (3)                            | 13:47:19.35 (2)            | -62:18:10.7 (1)                                 | 1.93 (8)                           | 1.86 (5)             |          |          |
|                                    |              |                    | -57.7 (2)                             | 13:47:19.3 (1)             | -62:18:09.4 (9)                                 | 1.8 (6)                            | 0.30 (5)             |          |          |
|                                    |              |                    | -55.24 (5)                            | 13:47:19.28 (3)            | -62:18:10.9 (2)                                 | 2.1 (1)                            | 1.49 (5)             |          |          |
|                                    | H            | 36                 | -52.08 (3)                            | 13:47:21.3 (1)             | -62:17:57.6 (5)                                 | 1.99 (8)                           | 1.11 (3)             |          |          |
|                                    |              |                    | -50.449 (4)                           | 13:47:21.48 (4)            | -62:17:56.4 (2)                                 | 0.28 (1)                           | 3.10 (9)             |          |          |
|                                    | I            | 44                 | -87.76 (4)                            | 13:47:25.05 (6)            | -62:18:10.3 (3)                                 | 0.30 (9)                           | 0.23 (6)             |          |          |
|                                    |              |                    | -53.25 (3)                            | 13:47:25.25 (8)            | -62:18:10.1 (4)                                 | 0.78 (8)                           | 0.46 (4)             |          |          |
| G316.76-0.01                       | J            | 44                 | -50.42 (1)                            | 13:47:21.90 (2)            | -62:18:03.3 (1)                                 | 0.41 (3)                           | 1.7 (1)              |          |          |
|                                    | A            | 44                 | -40.71 (1)                            | 14:44:57.72 (4)            | -59:48:00.1 (2)                                 | 0.82 (3)                           | 1.30 (4)             |          |          |
|                                    |              | B                  | 44                                    | -40.580 (7)                | 14:44:56.59 (2)                                 | -59:48:04.3 (2)                    | 0.17 (2)             | 0.96 (8) |          |
|                                    |              |                    | -39.84 (5)                            | 14:44:56.7 (1)             | -59:48:02 (2)                                   | 1.34 (8)                           | 0.8 (1)              |          |          |
|                                    |              |                    | -39.663 (6)                           | 14:44:56.77 (6)            | -59:48:02.9 (5)                                 | 0.47 (2)                           | 2.3 (1)              |          |          |
|                                    |              |                    | -39.22 (1)                            | 14:44:56.6 (1)             | -59:48:03.5 (7)                                 | 0.22 (3)                           | 0.74 (8)             |          |          |
|                                    |              |                    | -36.714 (7)                           | 14:44:56.49 (3)            | -59:48:03.8 (2)                                 | 0.60 (2)                           | 1.56 (4)             |          |          |
|                                    |              | C                  | 36                                    | -39.269 (1)                | 14:44:56.910 (5)                                | -59:47:59.30 (3)                   | 0.265 (2)            | 9.04 (5) |          |
|                                    |              |                    |                                       | -38.673 (4)                | 14:44:56.92 (2)                                 | -59:47:58.3 (1)                    | 0.392 (8)            | 2.41 (4) |          |
|                                    |              |                    |                                       | -37.736 (5)                | 14:44:56.669 (6)                                | -59:47:54.76 (4)                   | 0.47 (1)             | 1.90 (4) |          |
|                                    |              |                    | 44                                    | -39.467 (1)                | 14:44:56.92 (1)                                 | -59:47:59.04 (8)                   | 0.300 (1)            | 29.3 (1) |          |
|                                    |              |                    | -38.928 (3)                           | 14:44:56.929 (5)           | -59:47:58.20 (3)                                | 0.530 (7)                          | 10.41 (8)            |          |          |
|                                    |              |                    | -38.00 (1)                            | 14:44:56.66 (1)            | -59:47:54.97 (9)                                | 0.44 (3)                           | 7 (2)                |          |          |
|                                    |              |                    | -37.68 (8)                            | 14:44:56.72 (1)            | -59:47:55.00 (8)                                | 0.68 (8)                           | 6 (1)                |          |          |
|                                    |              | D                  | 36                                    | -41.8 (4)                  | 14:44:56.5 (1)                                  | -59:48:11.2 (7)                    | 2.0 (6)              | 0.17 (2) |          |
|                                    |              |                    |                                       | -40.41 (9)                 | 14:44:56.45 (4)                                 | -59:48:11.8 (2)                    | 1.1 (2)              | 0.27 (8) |          |
|                                    |              | E                  | 36                                    | -39.69 (1)                 | 14:44:53.40 (4)                                 | -59:48:10.7 (2)                    | 0.62 (3)             | 0.79 (3) |          |
|                                    |              | F                  | 36                                    | -39.3 (1)                  | 14:44:58.7 (2)                                  | -59:47:52.1 (8)                    | 2.0 (2)              | 0.20 (2) |          |
|                                    |              | G318.05+0.09       | A                                     | 44                         | -50.90 (2)                                      | 14:53:44.06 (5)                    | -59:08:49.0 (3)      | 0.34 (3) | 0.88 (8) |
|                                    | B            |                    | 36                                    | -49.95 (9)                 | 14:53:40.79 (9)                                 | -59:09:02.2 (6)                    | 2.4 (2)              | 0.22 (2) |          |
| 44                                 |              |                    | -50.605 (8)                           | 14:53:40.74 (1)            | -59:09:02.67 (8)                                | 0.49 (2)                           | 2.27 (8)             |          |          |
|                                    |              |                    | -49.765 (5)                           | 14:53:40.64 (1)            | -59:09:03.73 (8)                                | 0.47 (1)                           | 3.69 (8)             |          |          |
| C                                  | 36           |                    | -48.92 (6)                            | 14:53:44.22 (3)            | -59:08:54.2 (2)                                 | 1.4 (1)                            | 0.30 (3)             |          |          |
|                                    | 44           |                    | -49.80 (2)                            | 14:53:44.088 (8)           | -59:08:54.01 (4)                                | 0.56 (3)                           | 8.0 (3)              |          |          |
|                                    |              |                    | -49.124 (8)                           | 14:53:44.098 (3)           | -59:08:54.02 (2)                                | 0.66 (2)                           | 17.1 (2)             |          |          |
|                                    |              |                    | -48.10 (3)                            | 14:53:44.00 (2)            | -59:08:54.21 (9)                                | 0.49 (5)                           | 1.8 (2)              |          |          |
| D                                  | 36           |                    | -49.64 (9)                            | 14:53:45.6 (1)             | -59:09:06.4 (6)                                 | 2.3 (2)                            | 0.29 (4)             |          |          |
|                                    |              |                    | -49.62 (2)                            | 14:53:45.71 (3)            | -59:09:06.4 (2)                                 | 0.25 (5)                           | 0.68 (8)             |          |          |
|                                    |              |                    | -49.30 (6)                            | 14:53:45.70 (5)            | -59:09:06.2 (3)                                 | 0.3 (1)                            | 0.28 (8)             |          |          |
|                                    | E            |                    | 36                                    | -49.44 (3)                 | 14:53:44.67 (4)                                 | -59:09:00.9 (3)                    | 0.38 (6)             | 0.45 (5) |          |
|                                    |              |                    | -48.9 (1)                             | 14:53:44.8 (1)             | -59:08:59.3 (9)                                 | 0.5 (3)                            | 0.14 (4)             |          |          |
|                                    | F            |                    | 36                                    | -50.5 (5)                  | 14:53:45.5 (1)                                  | -59:08:58.4 (8)                    | 1.8 (8)              | 0.20 (5) |          |
|                                    | G            |                    | 44                                    | -52.83 (5)                 | 14:53:42.99 (6)                                 | -59:08:52.7 (3)                    | 1.1 (1)              | 0.44 (4) |          |
|                                    | G318.95-0.20 |                    | A                                     | 36                         | -36.69 (2)                                      | 15:00:55.31 (4)                    | -58:59:00.3 (3)      | 0.43 (8) | 0.51 (8) |
|                                    |              |                    |                                       | -35.998 (2)                | 15:00:55.326 (9)                                | -58:58:56.41 (6)                   | 0.303 (6)            | 4.8 (1)  |          |
|                                    |              |                    |                                       | -36.0 (2)                  | 15:00:55.2 (1)                                  | -58:59:01.8 (7)                    | 2.5 (6)              | 0.2 (1)  |          |
|                                    |              | -35.47 (4)         | 15:00:54.97 (6)                       | -58:58:59.5 (4)            | 0.9 (1)                                         | 1.0 (1)                            |                      |          |          |
|                                    | 44           | -37.29 (1)         | 15:00:55.42 (5)                       | -58:58:55.6 (3)            | 0.20 (3)                                        | 0.8 (1)                            |                      |          |          |

Table 3 – continued

| Source name                 | Location | Frequency<br>(GHz) | LSR<br>velocity<br>(km s <sup>-1</sup> ) | $\alpha_{2000}$<br>(h:m:s) | $\delta_{2000}$<br>(°:arcmin:arcsec) | Line<br>FWHM<br>(km s <sup>-1</sup> ) | Flux<br>density<br>(Jy) |
|-----------------------------|----------|--------------------|------------------------------------------|----------------------------|--------------------------------------|---------------------------------------|-------------------------|
| G318.95-0.20<br>(continued) | A        | 44                 | -36.240 (1)                              | 15:00:55.371 (4)           | -58:58:56.39 (3)                     | 0.298 (2)                             | 28.1 (2)                |
|                             |          |                    | -35.775 (9)                              | 15:00:55.10 (2)            | -58:58:57.6 (1)                      | 0.84 (2)                              | 5.70 (6)                |
|                             |          |                    | -33.94 (2)                               | 15:00:55.38 (3)            | -58:58:57.6 (2)                      | 0.65 (3)                              | 2.69 (8)                |
|                             |          |                    | -33.605 (7)                              | 15:00:55.39 (2)            | -58:58:58.0 (1)                      | 0.23 (3)                              | 1.7 (2)                 |
|                             | B        | 36                 | -35.806 (2)                              | 15:00:54.31 (1)            | -58:58:51.99 (9)                     | 0.279 (5)                             | 2.63 (4)                |
|                             |          |                    | -30.01 (1)                               | 15:00:54.81 (2)            | -58:58:49.4 (1)                      | 0.78 (4)                              | 0.63 (3)                |
|                             |          | 44                 | -36.310 (7)                              | 15:00:54.33 (8)            | -58:58:51.9 (5)                      | 0.18 (1)                              | 1.8 (1)                 |
|                             |          |                    | -36.018 (4)                              | 15:00:54.336 (7)           | -58:58:52.13 (5)                     | 0.32 (2)                              | 4.42 (6)                |
|                             | C        | 36                 | -35.679 (8)                              | 15:00:54.36 (2)            | -58:58:51.6 (1)                      | 0.26 (1)                              | 2.8 (1)                 |
|                             |          |                    | -33.21 (1)                               | 15:00:54.61 (3)            | -58:58:52.9 (2)                      | 0.24 (3)                              | 0.57 (8)                |
|                             |          |                    | -34.91 (2)                               | 15:00:57.1 (1)             | -58:59:00.7 (7)                      | 1.02 (8)                              | 0.77 (8)                |
|                             |          |                    | -34.892 (6)                              | 15:00:56.788 (6)           | -58:59:01.77 (4)                     | 0.26 (2)                              | 1.23 (8)                |
|                             |          | 44                 | -33.74 (2)                               | 15:00:57.37 (8)            | -58:59:03.9 (5)                      | 0.51 (5)                              | 0.51 (4)                |
|                             |          |                    | -30.43 (6)                               | 15:00:57.7 (1)             | -58:59:03.7 (7)                      | 4.2 (2)                               | 0.48 (1)                |
|                             |          |                    | -35.2 (3)                                | 15:00:56.77 (8)            | -58:59:01.3 (5)                      | 1.0 (4)                               | 0.7 (2)                 |
|                             |          |                    | -34.69 (2)                               | 15:00:56.80 (2)            | -58:59:01.7 (1)                      | 0.49 (8)                              | 1.6 (5)                 |
|                             | D        | 44                 | -33.78 (2)                               | 15:00:57.21 (4)            | -58:59:03.3 (2)                      | 0.39 (4)                              | 1.05 (8)                |
|                             |          |                    | -32.72 (3)                               | 15:00:55.1 (1)             | -58:58:48.9 (7)                      | 0.43 (6)                              | 0.45 (6)                |
|                             | E        | 36                 | -33.64 (2)                               | 15:00:53.36 (4)            | -58:58:45.4 (3)                      | 1.27 (5)                              | 1.16 (2)                |
|                             |          |                    | -32.18 (4)                               | 15:00:53.59 (3)            | -58:58:45.9 (2)                      | 1.03 (9)                              | 0.48 (3)                |
|                             | F        | 36                 | -28.31 (4)                               | 15:00:54.5 (1)             | -58:58:44.7 (7)                      | 1.1 (1)                               | 0.31 (2)                |
| G320.29-0.31                | A        | 36                 | -67.14 (2)                               | 15:10:19.02 (3)            | -58:25:16.2 (2)                      | 0.62 (5)                              | 1.27 (8)                |
|                             |          |                    | -66.52 (1)                               | 15:10:19.08 (6)            | -58:25:16.7 (4)                      | 0.38 (2)                              | 4.0 (1)                 |
|                             |          |                    | -66.188 (8)                              | 15:10:18.97 (4)            | -58:25:16.5 (3)                      | 0.30 (1)                              | 4.3 (2)                 |
|                             |          |                    | -65.660 (6)                              | 15:10:19.07 (4)            | -58:25:15.9 (3)                      | 0.45 (3)                              | 2.1 (1)                 |
|                             |          |                    | -64.739 (6)                              | 15:10:18.97 (3)            | -58:25:18.2 (2)                      | 0.34 (2)                              | 1.68 (8)                |
|                             |          |                    | -63.76 (1)                               | 15:10:18.95 (3)            | -58:25:17.3 (2)                      | 0.44 (4)                              | 0.74 (5)                |
|                             |          |                    | -60.63 (9)                               | 15:10:19.2 (1)             | -58:25:18.4 (9)                      | 0.7 (2)                               | 0.15 (4)                |
|                             |          | 44                 | -67.24 (4)                               | 15:10:19.09 (1)            | -58:25:15.49 (9)                     | 1.10 (5)                              | 9.3 (4)                 |
|                             |          |                    | -66.610 (9)                              | 15:10:19.16 (2)            | -58:25:16.4 (1)                      | 0.57 (2)                              | 34 (1)                  |
|                             |          |                    | -66.407 (1)                              | 15:10:19.081 (4)           | -58:25:16.14 (2)                     | 0.208 (3)                             | 47.3 (9)                |
|                             |          |                    | -65.92 (2)                               | 15:10:19.00 (8)            | -58:25:16.0 (4)                      | 0.60 (6)                              | 9.6 (8)                 |
|                             |          |                    | -64.96 (1)                               | 15:10:19.02 (2)            | -58:25:17.8 (1)                      | 0.38 (3)                              | 3.5 (3)                 |
|                             |          |                    | -63.94 (1)                               | 15:10:19.05 (1)            | -58:25:17.28 (8)                     | 0.27 (3)                              | 2.4 (2)                 |
|                             |          |                    | -62.36 (2)                               | 15:10:19.00 (3)            | -58:25:16.0 (2)                      | 0.55 (5)                              | 1.5 (1)                 |
|                             |          |                    | -60.44 (5)                               | 15:10:19.22 (4)            | -58:25:15.0 (2)                      | 0.7 (1)                               | 0.7 (1)                 |
| G322.16+0.64                | A        | 44                 | -58.799 (8)                              | 15:18:33.74 (3)            | -56:38:26.2 (2)                      | 0.22 (3)                              | 15 (3)                  |
|                             |          |                    | -58.51 (4)                               | 15:18:33.75 (4)            | -56:38:26.3 (2)                      | 0.50 (6)                              | 16.7 (9)                |
|                             |          |                    | -55.13 (5)                               | 15:18:33.3 (1)             | -56:38:25 (1)                        | 1.0 (1)                               | 4.7 (5)                 |
|                             |          |                    | -53.35 (1)                               | 15:18:33.46 (3)            | -56:38:22.2 (2)                      | 0.81 (3)                              | 14.4 (5)                |
|                             | B        | 36                 | -57.08 (4)                               | 15:18:33.68 (8)            | -56:38:36.3 (5)                      | 1.0 (1)                               | 1.2 (1)                 |
|                             |          | 44                 | -57.50 (1)                               | 15:18:33.60 (2)            | -56:38:37.2 (1)                      | 0.34 (3)                              | 13.7 (7)                |
|                             | C        | 44                 | -56.91 (2)                               | 15:18:33.61 (3)            | -56:38:36.4 (3)                      | 0.45 (6)                              | 6.8 (7)                 |
|                             |          |                    | -57.8 (1)                                | 15:18:33.6 (2)             | -56:38:34 (1)                        | 1.6 (3)                               | 2.8 (3)                 |
|                             | D        | 36                 | -56.28 (2)                               | 15:18:33.68 (8)            | -56:38:33.1 (5)                      | 0.47 (5)                              | 7.0 (7)                 |
|                             |          |                    | -55.12 (8)                               | 15:18:34.7 (1)             | -56:38:19.6 (9)                      | 2.0 (2)                               | 0.80 (6)                |
|                             |          |                    | -53.858 (7)                              | 15:18:35.01 (2)            | -56:38:20.7 (1)                      | 0.30 (2)                              | 3.0 (1)                 |
|                             |          |                    | -55.393 (8)                              | 15:18:34.71 (3)            | -56:38:19.1 (2)                      | 0.47 (2)                              | 12.2 (4)                |

**Table 3** – *continued*

| Source name                 | Location | Frequency<br>(GHz) | LSR<br>velocity<br>(km s <sup>-1</sup> ) | $\alpha_{2000}$<br>(h:m:s) | $\delta_{2000}$<br>(°:arcmin:arcsec) | Line<br>FWHM<br>(km s <sup>-1</sup> ) | Flux<br>density<br>(Jy) |
|-----------------------------|----------|--------------------|------------------------------------------|----------------------------|--------------------------------------|---------------------------------------|-------------------------|
| G322.16+0.64<br>(continued) | D        | 44                 | -54.43 (8)                               | 15:18:34.99 (5)            | -56:38:21.2 (3)                      | 0.82 (9)                              | 7.8 (8)                 |
|                             |          |                    | -54.064 (7)                              | 15:18:35.00 (2)            | -56:38:21.4 (1)                      | 0.39 (3)                              | 17 (2)                  |
|                             | E        | 36                 | -55.60 (4)                               | 15:18:40.67 (6)            | -56:38:41.0 (4)                      | 0.7 (1)                               | 0.34 (4)                |
|                             |          |                    | -54.3 (1)                                | 15:18:40.69 (8)            | -56:38:38.6 (8)                      | 5.1 (4)                               | 0.36 (8)                |
|                             |          |                    | -53.9 (3)                                | 15:18:40.6 (1)             | -56:38:43.4 (8)                      | 1.9 (4)                               | 1.3 (4)                 |
|                             |          |                    | -53.12 (2)                               | 15:18:40.26 (8)            | -56:38:49.7 (5)                      | 1.19 (8)                              | 3.4 (7)                 |
|                             |          |                    | -52.11 (2)                               | 15:18:40.26 (8)            | -56:38:48.9 (6)                      | 0.92 (4)                              | 0.60 (2)                |
|                             |          |                    | -52.305 (6)                              | 15:18:39.74 (1)            | -56:38:46.4 (1)                      | 0.38 (1)                              | 1.97 (6)                |
|                             | F        | 36                 | -59.32 (2)                               | 15:18:34.70 (3)            | -56:38:36.9 (2)                      | 0.69 (5)                              | 1.51 (8)                |
|                             |          |                    | -58.18 (6)                               | 15:18:34.76 (5)            | -56:38:38.4 (3)                      | 0.9 (1)                               | 0.64 (8)                |
|                             | G        | 36                 | -55.04 (2)                               | 15:18:38.34 (5)            | -56:37:55.1 (4)                      | 0.98 (6)                              | 1.68 (9)                |
|                             | H        | 36                 | -54.04 (1)                               | 15:18:38.45 (5)            | -56:38:00.4 (4)                      | 0.30 (3)                              | 1.4 (1)                 |
|                             |          |                    | -53.8 (1)                                | 15:18:38.40 (8)            | -56:37:58.8 (6)                      | 3.3 (3)                               | 0.44 (5)                |
| G323.74-0.26                | A        | 44                 | -52.99 (2)                               | 15:31:44.98 (4)            | -56:30:44.7 (3)                      | 0.24 (5)                              | 0.8 (1)                 |
|                             |          |                    | -52.607 (5)                              | 15:31:44.99 (1)            | -56:30:45.00 (6)                     | 0.31 (1)                              | 3.40 (9)                |
|                             |          |                    | -50.985 (3)                              | 15:31:45.11 (1)            | -56:30:47.16 (8)                     | 0.406 (6)                             | 5.88 (8)                |
|                             | B        | 36                 | -49.95 (2)                               | 15:31:46.02 (6)            | -56:30:58.7 (4)                      | 0.88 (4)                              | 0.98 (5)                |
|                             |          |                    | -49.834 (6)                              | 15:31:46.10 (2)            | -56:30:57.8 (1)                      | 0.17 (2)                              | 0.95 (8)                |
|                             |          |                    | -48.56 (8)                               | 15:31:46.0 (1)             | -56:30:56.5 (7)                      | 1.2 (2)                               | 0.29 (2)                |
|                             |          | 44                 | -50.444 (7)                              | 15:31:46.17 (2)            | -56:30:58.0 (2)                      | 0.30 (2)                              | 2.49 (8)                |
|                             |          |                    | -50.039 (3)                              | 15:31:46.129 (7)           | -56:30:57.70 (4)                     | 0.315 (8)                             | 7.19 (8)                |
|                             |          |                    | -49.64 (1)                               | 15:31:46.03 (3)            | -56:30:57.7 (2)                      | 0.24 (3)                              | 0.99 (9)                |
|                             | C        | 44                 | -49.64 (1)                               | 15:31:45.76 (3)            | -56:30:50.7 (2)                      | 0.38 (3)                              | 1.13 (8)                |
|                             | D        | 36                 | -47.571 (9)                              | 15:31:46.15 (2)            | -56:30:44.7 (1)                      | 0.19 (2)                              | 0.68 (6)                |
|                             |          |                    | -47.835 (9)                              | 15:31:46.15 (2)            | -56:30:44.6 (1)                      | 0.30 (2)                              | 1.47 (9)                |
| G324.72+0.34                | A        | 36                 | -55.77 (2)                               | 15:34:55.78 (8)            | -55:27:47.2 (5)                      | 0.31 (6)                              | 0.42 (8)                |
|                             |          |                    | -53.61 (4)                               | 15:34:55.85 (8)            | -55:27:45.8 (6)                      | 1.1 (1)                               | 0.46 (4)                |
|                             |          |                    | -56.09 (2)                               | 15:34:55.74 (4)            | -55:27:46.3 (3)                      | 0.46 (4)                              | 1.19 (9)                |
|                             |          |                    | -54.24 (2)                               | 15:34:56.20 (2)            | -55:27:45.0 (2)                      | 0.48 (6)                              | 1.08 (9)                |
|                             |          |                    | -53.64 (4)                               | 15:34:55.83 (3)            | -55:27:46.2 (2)                      | 0.40 (9)                              | 0.63 (9)                |
|                             | B        | 36                 | -53.097 (2)                              | 15:35:01.27 (2)            | -55:27:07.2 (1)                      | 0.267 (7)                             | 13.5 (6)                |
|                             |          |                    | -52.958 (8)                              | 15:35:01.137 (9)           | -55:27:07.62 (5)                     | 0.509 (7)                             | 10.9 (5)                |
|                             |          |                    | -52.067 (2)                              | 15:35:00.791 (6)           | -55:27:07.92 (4)                     | 0.373 (3)                             | 13.0 (1)                |
|                             |          |                    | -47.0 (1)                                | 15:35:01.7 (1)             | -55:27:08.3 (7)                      | 3.4 (3)                               | 0.47 (3)                |
|                             |          |                    | -53.37 (4)                               | 15:35:01.32 (3)            | -55:27:07.7 (2)                      | 0.28 (4)                              | 4 (1)                   |
|                             |          | 44                 | -53.13 (4)                               | 15:35:01.26 (3)            | -55:27:07.0 (2)                      | 0.31 (4)                              | 5.7 (9)                 |
|                             |          |                    | -52.36 (2)                               | 15:35:00.68 (5)            | -55:27:07.6 (3)                      | 0.44 (3)                              | 4.0 (9)                 |
|                             |          |                    | -52.255 (7)                              | 15:35:00.78 (3)            | -55:27:08.1 (2)                      | 0.25 (2)                              | 5 (1)                   |
|                             |          |                    | -52.96 (2)                               | 15:34:54.10 (3)            | -55:27:27.1 (2)                      | 1.14 (4)                              | 1.93 (6)                |
|                             |          |                    | -51.759 (1)                              | 15:34:54.503 (3)           | -55:27:29.64 (2)                     | 0.275 (1)                             | 33.0 (1)                |
|                             | C        | 44                 | -52.266 (6)                              | 15:34:54.56 (4)            | -55:27:29.1 (3)                      | 0.20 (1)                              | 4.2 (1)                 |
|                             |          |                    | -51.982 (1)                              | 15:34:54.513 (2)           | -55:27:29.64 (2)                     | 0.236 (2)                             | 57.5 (1)                |
|                             |          |                    | -51.73 (1)                               | 15:34:54.54 (6)            | -55:27:29.1 (5)                      | 0.18 (3)                              | 2.0 (2)                 |
|                             |          |                    | -51.726 (6)                              | 15:34:58.681 (6)           | -55:27:14.17 (4)                     | 0.40 (1)                              | 2.55 (5)                |
|                             |          |                    | -51.118 (6)                              | 15:34:58.45 (3)            | -55:27:14.3 (2)                      | 0.30 (3)                              | 2.0 (4)                 |
|                             | D        | 36                 | -50.83 (8)                               | 15:34:58.4 (1)             | -55:27:14.5 (7)                      | 0.66 (9)                              | 1.3 (1)                 |
|                             |          |                    | -51.965 (3)                              | 15:34:58.58 (1)            | -55:27:14.34 (8)                     | 0.456 (7)                             | 6.88 (8)                |
|                             |          |                    | -51.321 (3)                              | 15:34:58.503 (4)           | -55:27:14.00 (3)                     | 0.29 (2)                              | 5.9 (7)                 |



Table 3 – continued

| Source name                 | Location | Frequency<br>(GHz) | LSR<br>velocity<br>(km s <sup>-1</sup> ) | $\alpha_{2000}$<br>(h:m:s) | $\delta_{2000}$<br>(°:arcmin:arcsec) | Line<br>FWHM<br>(km s <sup>-1</sup> ) | Flux<br>density<br>(Jy) |
|-----------------------------|----------|--------------------|------------------------------------------|----------------------------|--------------------------------------|---------------------------------------|-------------------------|
| G324.72+0.34<br>(continued) | E        | 36                 | -53.341 (9)                              | 15:34:58.11 (4)            | -55:27:33.5 (3)                      | 0.28 (2)                              | 0.81 (6)                |
|                             |          |                    | -48.77 (2)                               | 15:34:58.13 (1)            | -55:27:31.2 (1)                      | 0.47 (3)                              | 1.36 (5)                |
|                             |          |                    | -48.21 (1)                               | 15:34:58.13 (1)            | -55:27:31.04 (8)                     | 0.47 (3)                              | 1.38 (5)                |
|                             | F        | 36                 | -52.29 (1)                               | 15:34:56.75 (3)            | -55:27:16.6 (2)                      | 0.41 (3)                              | 0.96 (5)                |
|                             |          |                    | -50.56 (9)                               | 15:34:57.0 (1)             | -55:27:20.6 (8)                      | 3.6 (2)                               | 0.41 (2)                |
| G326.48+0.70                | A        | 36                 | -49.65 (3)                               | 15:43:16.476 (6)           | -54:07:13.35 (4)                     | 0.37 (5)                              | 3.8 (6)                 |
|                             |          |                    | -49.20 (8)                               | 15:43:16.47 (2)            | -54:07:13.6 (1)                      | 0.5 (1)                               | 2.1 (3)                 |
|                             |          |                    | -46.1 (2)                                | 15:43:16.51 (9)            | -54:07:12.9 (6)                      | 9.3 (3)                               | 2.7 (2)                 |
|                             |          |                    | -45.550 (3)                              | 15:43:16.442 (2)           | -54:07:13.59 (1)                     | 0.566 (8)                             | 23.0 (3)                |
|                             |          |                    | -44.313 (3)                              | 15:43:16.468 (2)           | -54:07:13.70 (1)                     | 0.444 (9)                             | 17.3 (3)                |
|                             |          |                    | -42.58 (2)                               | 15:43:16.443 (4)           | -54:07:14.01 (3)                     | 0.59 (3)                              | 10.6 (2)                |
|                             |          |                    | -42.16 (1)                               | 15:43:16.421 (7)           | -54:07:14.44 (4)                     | 0.29 (3)                              | 5.9 (7)                 |
|                             |          |                    | -41.62 (2)                               | 15:43:16.409 (8)           | -54:07:13.99 (5)                     | 0.44 (4)                              | 6.2 (4)                 |
|                             |          |                    | -40.97 (2)                               | 15:43:16.32 (6)            | -54:07:15.6 (4)                      | 0.74 (4)                              | 2.0 (1)                 |
|                             |          |                    | -39.95 (2)                               | 15:43:16.48 (3)            | -54:07:12.7 (2)                      | 0.50 (6)                              | 2.1 (2)                 |
|                             |          |                    | -37.62 (3)                               | 15:43:17.06 (5)            | -54:07:14.8 (3)                      | 1.50 (8)                              | 0.92 (4)                |
|                             |          | 44                 | -49.20 (3)                               | 15:43:16.43 (1)            | -54:07:13.22 (9)                     | 0.48 (8)                              | 2.3 (3)                 |
|                             |          |                    | -46.39 (3)                               | 15:43:16.434 (5)           | -54:07:13.29 (3)                     | 0.46 (6)                              | 6.1 (4)                 |
|                             |          |                    | -45.92 (2)                               | 15:43:16.429 (5)           | -54:07:13.30 (3)                     | 0.40 (4)                              | 9.2 (5)                 |
|                             |          |                    | -44.54 (8)                               | 15:43:16.45 (1)            | -54:07:13.00 (8)                     | 4.9 (1)                               | 7.1 (2)                 |
|                             |          |                    | -44.518 (2)                              | 15:43:16.427 (1)           | -54:07:13.650 (4)                    | 0.445 (6)                             | 44.2 (4)                |
|                             |          |                    | -43.97 (2)                               | 15:43:16.419 (6)           | -54:07:13.71 (4)                     | 0.34 (4)                              | 5.3 (4)                 |
|                             |          |                    | -42.27 (2)                               | 15:43:16.379 (2)           | -54:07:14.21 (1)                     | 0.8 (1)                               | 36.3 (5)                |
|                             |          |                    | -41.777 (3)                              | 15:43:16.369 (8)           | -54:07:13.99 (5)                     | 0.39 (2)                              | 35 (4)                  |
|                             |          |                    | -40.841 (9)                              | 15:43:16.093 (4)           | -54:07:16.41 (2)                     | 0.48 (1)                              | 14.1 (2)                |
|                             |          |                    | -39.92 (1)                               | 15:43:16.89 (2)            | -54:07:12.2 (1)                      | 0.14 (3)                              | 1.0 (1)                 |
|                             | B        | 36                 | -39.25 (2)                               | 15:43:15.72 (3)            | -54:07:09.9 (2)                      | 1.36 (5)                              | 1.36 (4)                |
|                             |          | 44                 | -39.518 (8)                              | 15:43:15.68 (1)            | -54:07:10.40 (8)                     | 1.34 (2)                              | 4.18 (5)                |
|                             | D        | 36                 | -45.40 (2)                               | 15:43:19.004 (9)           | -54:07:40.5 (1)                      | 0.45 (4)                              | 1.09 (8)                |
|                             |          |                    | -43.039 (1)                              | 15:43:19.120 (3)           | -54:07:35.68 (1)                     | 0.218 (3)                             | 9.7 (1)                 |
|                             |          |                    | -42.16 (2)                               | 15:43:19.08 (5)            | -54:07:34.9 (3)                      | 0.34 (5)                              | 0.8 (1)                 |
|                             |          |                    | -43.280 (2)                              | 15:43:19.076 (3)           | -54:07:35.66 (2)                     | 0.311 (5)                             | 35.6 (4)                |
|                             |          | 44                 | -42.953 (4)                              | 15:43:18.969 (8)           | -54:07:35.69 (5)                     | 0.21 (1)                              | 11.2 (5)                |
|                             |          |                    | -42.362 (7)                              | 15:43:19.126 (4)           | -54:07:35.10 (3)                     | 0.35 (2)                              | 7.3 (4)                 |
|                             |          |                    | -46.9 (2)                                | 15:43:18.9 (2)             | -54:07:42 (1)                        | 1.9 (6)                               | 0.24 (5)                |
|                             |          |                    | -45.395 (1)                              | 15:43:19.008 (6)           | -54:07:40.55 (4)                     | 0.356 (4)                             | 22.9 (1)                |
|                             | E        | 36                 | -44.987 (3)                              | 15:43:18.97 (1)            | -54:07:40.54 (8)                     | 0.300 (7)                             | 9.5 (1)                 |
|                             |          |                    | -45.94 (3)                               | 15:43:19.033 (3)           | -54:07:40.47 (2)                     | 0.45 (4)                              | 13.1 (9)                |
|                             |          |                    | -45.572 (5)                              | 15:43:19.033 (3)           | -54:07:40.47 (2)                     | 0.35 (1)                              | 46 (1)                  |
|                             |          |                    | -45.143 (2)                              | 15:43:19.050 (3)           | -54:07:40.46 (2)                     | 0.352 (4)                             | 55.0 (4)                |
|                             |          | 44                 | -41.588 (5)                              | 15:43:18.72 (2)            | -54:07:14.8 (1)                      | 0.44 (1)                              | 2.50 (6)                |
|                             |          |                    | -36.58 (2)                               | 15:43:15.99 (1)            | -54:07:06.68 (9)                     | 1.39 (4)                              | 1.41 (4)                |
|                             |          |                    | -30.64 (2)                               | 15:43:15.43 (2)            | -54:07:16.5 (1)                      | 1.13 (4)                              | 1.59 (5)                |
|                             |          |                    | -53.40 (2)                               | 15:43:20.68 (5)            | -54:07:31.7 (3)                      | 0.58 (4)                              | 1.5 (1)                 |
| G326.64+0.61                | A        | 36                 | -39.914 (2)                              | 15:44:33.41 (2)            | -54:05:16.6 (1)                      | 0.299 (4)                             | 7.57 (8)                |
|                             |          |                    | -39.434 (2)                              | 15:44:33.418 (5)           | -54:05:16.47 (4)                     | 0.473 (8)                             | 8.78 (6)                |
|                             |          |                    | -38.908 (6)                              | 15:44:33.54 (3)            | -54:05:17.8 (2)                      | 0.18 (2)                              | 1.5 (2)                 |
|                             |          |                    | -38.50 (5)                               | 15:44:33.76 (3)            | -54:05:18.1 (2)                      | 0.7 (2)                               | 1.41 (8)                |

**Table 3** – *continued*

| Source name                 | Location | Frequency<br>(GHz) | LSR<br>velocity<br>(km s <sup>-1</sup> ) | $\alpha_{2000}$<br>(h:m:s) | $\delta_{2000}$<br>(°:arcmin:arcsec) | Line<br>FWHM<br>(km s <sup>-1</sup> ) | Flux<br>density<br>(Jy) |
|-----------------------------|----------|--------------------|------------------------------------------|----------------------------|--------------------------------------|---------------------------------------|-------------------------|
| G326.64+0.61<br>(continued) | A        | 36                 | -37.88 (3)                               | 15:44:33.66 (3)            | -54:05:18.1 (2)                      | 0.51 (8)                              | 2.2 (2)                 |
|                             |          |                    | -37.537 (2)                              | 15:44:33.20 (2)            | -54:05:18.1 (1)                      | 0.171 (8)                             | 4.0 (2)                 |
|                             |          |                    | -37.02 (2)                               | 15:44:33.972 (5)           | -54:05:18.49 (3)                     | 0.49 (4)                              | 2.9 (6)                 |
|                             |          |                    | -36.6 (1)                                | 15:44:34.03 (2)            | -54:05:18.7 (1)                      | 0.8 (2)                               | 1.6 (6)                 |
|                             |          |                    | -35.9 (6)                                | 15:44:34.04 (5)            | -54:05:18.4 (3)                      | 1.6 (6)                               | 0.5 (2)                 |
|                             |          | 44                 | -41.1 (1)                                | 15:44:33.36 (9)            | -54:05:18.4 (4)                      | 3.4 (2)                               | 0.63 (3)                |
|                             |          |                    | -40.95 (3)                               | 15:44:33.56 (8)            | -54:05:18.2 (5)                      | 0.46 (8)                              | 0.66 (9)                |
|                             |          |                    | -40.126 (2)                              | 15:44:33.436 (7)           | -54:05:16.27 (4)                     | 0.234 (5)                             | 11.6 (3)                |
|                             |          |                    | -39.766 (7)                              | 15:44:33.44 (2)            | -54:05:16.1 (1)                      | 0.54 (1)                              | 9.4 (1)                 |
|                             |          |                    | -38.211 (5)                              | 15:44:33.27 (2)            | -54:05:14.23 (9)                     | 0.37 (1)                              | 3.9 (1)                 |
|                             | B        | 44                 | -39.55 (1)                               | 15:44:33.64 (4)            | -54:05:21.7 (2)                      | 0.31 (3)                              | 1.5 (1)                 |
|                             |          |                    | -38.117 (6)                              | 15:44:33.55 (3)            | -54:05:21.3 (1)                      | 0.65 (1)                              | 3.77 (8)                |
|                             | C        | 44                 | -37.32 (5)                               | 15:44:29.9 (2)             | -54:05:17 (1)                        | 1.2 (1)                               | 1.0 (1)                 |
|                             |          |                    | -37.292 (1)                              | 15:44:29.660 (9)           | -54:05:18.28 (5)                     | 0.179 (3)                             | 14.4 (2)                |
|                             | D        | 36                 | -39.8 (2)                                | 15:44:32.4 (1)             | -54:05:32.7 (6)                      | 2.5 (2)                               | 0.73 (9)                |
|                             |          |                    | -39.26 (2)                               | 15:44:32.528 (8)           | -54:05:30.66 (5)                     | 0.94 (3)                              | 4.1 (1)                 |
|                             |          |                    | -38.40 (4)                               | 15:44:32.69 (2)            | -54:05:31.8 (1)                      | 0.84 (8)                              | 1.7 (1)                 |
|                             |          |                    | -40.443 (6)                              | 15:44:32.49 (4)            | -54:05:30.0 (2)                      | 0.42 (2)                              | 3.2 (1)                 |
|                             |          |                    | -39.538 (9)                              | 15:44:32.45 (3)            | -54:05:30.4 (2)                      | 0.69 (3)                              | 3.8 (2)                 |
|                             |          | 44                 | -39.38 (4)                               | 15:44:32.44 (4)            | -54:05:31.4 (2)                      | 3.3 (2)                               | 1.7 (2)                 |
|                             |          |                    | -38.77 (1)                               | 15:44:32.65 (4)            | -54:05:31.7 (2)                      | 0.46 (3)                              | 5.5 (2)                 |
|                             |          |                    | -38.30 (2)                               | 15:44:32.63 (3)            | -54:05:32.6 (1)                      | 0.46 (4)                              | 3.4 (2)                 |
|                             |          | E                  | -36.634 (4)                              | 15:44:32.21 (2)            | -54:05:25.1 (1)                      | 0.25 (1)                              | 1.62 (6)                |
|                             |          |                    | -36.887 (4)                              | 15:44:32.17 (2)            | -54:05:25.1 (1)                      | 0.31 (1)                              | 3.24 (9)                |
|                             | F        | 36                 | -43.7 (1)                                | 15:44:32.7 (1)             | -54:05:01.2 (6)                      | 3.9 (3)                               | 0.48 (6)                |
|                             |          |                    | -43.51 (1)                               | 15:44:32.78 (1)            | -54:05:00.95 (8)                     | 0.97 (3)                              | 4.04 (8)                |
|                             |          |                    | -42.52 (2)                               | 15:44:32.69 (5)            | -54:05:00.3 (3)                      | 0.81 (4)                              | 2.21 (8)                |
|                             | G        | 36                 | -41.61 (4)                               | 15:44:33.01 (4)            | -54:05:22.5 (3)                      | 1.9 (1)                               | 0.73 (3)                |
|                             |          |                    | -39.989 (3)                              | 15:44:32.91 (2)            | -54:05:23.1 (1)                      | 0.540 (7)                             | 4.87 (5)                |
|                             |          |                    | -36.242 (5)                              | 15:44:32.64 (2)            | -54:05:20.7 (1)                      | 0.30 (1)                              | 2.10 (8)                |
|                             | H        | 36                 | -37.70 (2)                               | 15:44:31.06 (5)            | -54:05:01.2 (3)                      | 0.51 (3)                              | 3.4 (1)                 |
|                             |          |                    | -37.427 (1)                              | 15:44:31.086 (4)           | -54:05:00.68 (3)                     | 0.209 (4)                             | 16.3 (3)                |
|                             | I        | 36                 | -37.324 (3)                              | 15:44:28.761 (6)           | -54:04:56.54 (4)                     | 0.502 (6)                             | 20.4 (1)                |
|                             |          |                    | -36.872 (9)                              | 15:44:28.92 (5)            | -54:04:57.3 (3)                      | 0.31 (2)                              | 4.5 (2)                 |
|                             | J        | 36                 | -36.63 (3)                               | 15:44:33.76 (9)            | -54:05:26.3 (4)                      | 0.7 (1)                               | 0.5 (1)                 |
|                             |          |                    | -35 (6)                                  | 15:44:33.96 (3)            | -54:05:26.2 (2)                      | 3 (3)                                 | 1 (7)                   |
|                             | K        | 36                 | -64.0 (2)                                | 15:44:28.2 (2)             | -54:04:47 (2)                        | 1.8 (4)                               | 0.84 (9)                |
|                             |          |                    | -62.84 (2)                               | 15:44:28.02 (4)            | -54:04:47.9 (2)                      | 0.45 (8)                              | 1.8 (2)                 |
|                             |          |                    | -28.6 (2)                                | 15:44:28.21 (8)            | -54:04:49.7 (4)                      | 2.9 (5)                               | 0.8 (1)                 |
|                             |          |                    | -28.31 (2)                               | 15:44:28.42 (4)            | -54:04:49.8 (3)                      | 0.30 (5)                              | 1.6 (2)                 |
|                             |          |                    | -26.53 (4)                               | 15:44:28.44 (8)            | -54:04:50.0 (5)                      | 0.8 (1)                               | 1.4 (2)                 |
| G326.66+0.57                | A        | 36                 | -41.33 (1)                               | 15:44:46.39 (6)            | -54:06:44.6 (4)                      | 0.18 (3)                              | 0.51 (8)                |
|                             | B        | 44                 | -41.20 (1)                               | 15:44:48.97 (2)            | -54:06:41.1 (2)                      | 0.19 (3)                              | 0.9 (1)                 |
| G326.86-0.68                | A        | 36                 | -68.80 (4)                               | 15:51:14.17 (4)            | -54:58:04.6 (3)                      | 0.48 (9)                              | 0.44 (8)                |
|                             |          |                    | -68.03 (4)                               | 15:51:14.11 (4)            | -54:58:04.5 (3)                      | 0.8 (1)                               | 0.7 (1)                 |
|                             |          |                    | -68.0 (1)                                | 15:51:14.11 (8)            | -54:58:05.3 (5)                      | 3.3 (2)                               | 0.8 (1)                 |
|                             |          |                    | -66.99 (1)                               | 15:51:13.99 (8)            | -54:58:05.3 (5)                      | 0.37 (5)                              | 0.7 (1)                 |
|                             |          |                    | -66.11 (2)                               | 15:51:13.82 (5)            | -54:58:05.5 (3)                      | 0.66 (6)                              | 0.85 (8)                |

Table 3 – continued

| Source name                 | Location | Frequency<br>(GHz) | LSR<br>velocity<br>(km s <sup>-1</sup> ) | $\alpha_{2000}$<br>(h:m:s) | $\delta_{2000}$<br>(°:arcmin:arcsec) | Line<br>FWHM<br>(km s <sup>-1</sup> ) | Flux<br>density<br>(Jy) |
|-----------------------------|----------|--------------------|------------------------------------------|----------------------------|--------------------------------------|---------------------------------------|-------------------------|
| G326.86-0.68<br>(continued) | A        | 44                 | -67.187 (7)                              | 15:51:13.68 (1)            | -54:58:04.86 (8)                     | 0.54 (2)                              | 10.2 (1)                |
|                             |          |                    | -66.583 (8)                              | 15:51:13.70 (2)            | -54:58:04.8 (1)                      | 0.52 (3)                              | 7.8 (1)                 |
|                             |          |                    | -65.99 (4)                               | 15:51:14.00 (5)            | -54:58:05.6 (3)                      | 0.54 (8)                              | 1.6 (1)                 |
|                             | B        | 44                 | -68.10 (1)                               | 15:51:14.17 (3)            | -54:58:03.3 (2)                      | 0.51 (3)                              | 1.70 (9)                |
|                             | C        | 44                 | -69.113 (8)                              | 15:51:14.55 (2)            | -54:58:07.4 (1)                      | 0.28 (2)                              | 1.9 (1)                 |
| G327.29-0.58                | D        | 44                 | -68.190 (9)                              | 15:51:13.32 (4)            | -54:58:01.9 (2)                      | 0.17 (2)                              | 1.3 (1)                 |
|                             | A        | 36                 | -47.76 (2)                               | 15:53:09.36 (6)            | -54:36:57.4 (4)                      | 0.17 (5)                              | 0.4 (1)                 |
|                             |          |                    | -46.6 (4)                                | 15:53:09.2 (1)             | -54:36:57.9 (6)                      | 2.8 (4)                               | 0.9 (1)                 |
|                             |          |                    | -46.472 (8)                              | 15:53:09.69 (2)            | -54:36:59.5 (1)                      | 0.47 (2)                              | 2.58 (9)                |
|                             |          |                    | -45.498 (7)                              | 15:53:09.66 (2)            | -54:36:59.3 (1)                      | 1.23 (4)                              | 5.8 (3)                 |
|                             |          |                    | -43.65 (5)                               | 15:53:09.35 (5)            | -54:36:55.6 (4)                      | 0.8 (1)                               | 0.59 (9)                |
|                             |          | 44                 | -48.03 (2)                               | 15:53:09.41 (3)            | -54:37:01.4 (2)                      | 0.50 (4)                              | 2.4 (1)                 |
|                             |          |                    | -46.692 (1)                              | 15:53:09.708 (3)           | -54:36:59.17 (2)                     | 0.361 (3)                             | 35.7 (2)                |
|                             |          |                    | -46.070 (8)                              | 15:53:09.660 (9)           | -54:36:58.82 (6)                     | 1.34 (2)                              | 15.8 (1)                |
|                             |          |                    | -45.06 (1)                               | 15:53:09.46 (8)            | -54:36:59.0 (4)                      | 0.40 (4)                              | 2.7 (2)                 |
|                             |          | B                  | -44.51 (4)                               | 15:53:07.78 (2)            | -54:37:06.3 (1)                      | 1.8 (1)                               | 1.21 (8)                |
|                             |          |                    | -43.93 (4)                               | 15:53:07.81 (8)            | -54:37:05.4 (5)                      | 5.8 (1)                               | 1.50 (8)                |
|                             |          |                    | -42.79 (6)                               | 15:53:07.87 (4)            | -54:37:06.7 (2)                      | 1.3 (1)                               | 0.61 (6)                |
|                             |          |                    | -45.646 (1)                              | 15:53:08.16 (1)            | -54:37:06.38 (6)                     | 0.283 (4)                             | 15.4 (2)                |
|                             |          |                    | -44.83 (4)                               | 15:53:07.65 (1)            | -54:37:05.88 (8)                     | 0.82 (5)                              | 12.6 (9)                |
|                             |          |                    | -44.51 (6)                               | 15:53:07.80 (5)            | -54:37:05.5 (3)                      | 5.5 (2)                               | 1.59 (8)                |
|                             |          |                    | -44.27 (3)                               | 15:53:07.663 (4)           | -54:37:05.83 (3)                     | 0.69 (2)                              | 14 (2)                  |
|                             |          |                    | -42.86 (2)                               | 15:53:07.88 (5)            | -54:37:06.5 (3)                      | 0.24 (4)                              | 1.0 (1)                 |
|                             |          | C                  | -41.353 (5)                              | 15:53:08.00 (3)            | -54:37:09.2 (2)                      | 0.44 (1)                              | 3.53 (9)                |
|                             |          |                    | -42.329 (2)                              | 15:53:09.34 (2)            | -54:36:45.4 (1)                      | 0.274 (5)                             | 5.12 (9)                |
|                             | D        | 36                 | -42.588 (3)                              | 15:53:09.28 (1)            | -54:36:44.89 (8)                     | 0.281 (7)                             | 8.8 (2)                 |
|                             | E        | 36                 | -46.80 (1)                               | 15:53:10.85 (2)            | -54:36:47.40 (9)                     | 1.09 (3)                              | 3.7 (1)                 |
|                             |          |                    | -46.4 (3)                                | 15:53:10.68 (8)            | -54:36:46.5 (5)                      | 3.6 (7)                               | 0.31 (9)                |
|                             |          | 44                 | -47.87 (8)                               | 15:53:10.9 (1)             | -54:36:47.0 (6)                      | 0.7 (2)                               | 1.8 (2)                 |
|                             |          |                    | -47.110 (9)                              | 15:53:10.85 (2)            | -54:36:46.5 (1)                      | 0.48 (2)                              | 10.2 (3)                |
|                             |          |                    | -46.400 (9)                              | 15:53:10.94 (3)            | -54:36:45.2 (2)                      | 0.32 (2)                              | 6.0 (4)                 |
|                             | F        | 44                 | -42.929 (6)                              | 15:53:11.13 (4)            | -54:36:45.5 (3)                      | 0.19 (2)                              | 6.0 (4)                 |
|                             |          |                    | -47.17 (1)                               | 15:53:07.32 (5)            | -54:36:57.9 (3)                      | 0.64 (3)                              | 1.43 (6)                |
|                             |          |                    | -43.02 (3)                               | 15:53:08.27 (8)            | -54:37:03.1 (5)                      | 1.19 (8)                              | 1.77 (8)                |
|                             |          |                    | -42.988 (9)                              | 15:53:08.36 (9)            | -54:37:03.6 (6)                      | 0.29 (3)                              | 1.12 (9)                |
|                             |          |                    | -41.7 (1)                                | 15:53:08.28 (9)            | -54:37:05.8 (8)                      | 1.1 (2)                               | 0.39 (4)                |
|                             | H        | 36                 | -41.23 (4)                               | 15:53:11.63 (5)            | -54:36:53.2 (3)                      | 1.3 (1)                               | 1.27 (8)                |
|                             |          |                    | -39.71 (3)                               | 15:53:11.7 (1)             | -54:36:53.7 (6)                      | 0.53 (8)                              | 1.2 (1)                 |
|                             |          |                    | -38.68 (3)                               | 15:53:11.71 (6)            | -54:36:53.7 (3)                      | 0.96 (8)                              | 1.92 (9)                |
|                             | I        | 36                 | -44.475 (2)                              | 15:53:08.61 (2)            | -54:36:49.6 (1)                      | 0.251 (6)                             | 3.67 (8)                |
| G327.39+0.20                | A        | 36                 | -91.28 (3)                               | 15:50:20.16 (8)            | -53:57:08.2 (6)                      | 0.65 (8)                              | 0.44 (5)                |
|                             |          |                    | -89.57 (2)                               | 15:50:20.26 (5)            | -53:57:08.0 (4)                      | 0.53 (5)                              | 0.64 (5)                |
|                             |          | 44                 | -91.60 (1)                               | 15:50:20.29 (2)            | -53:57:08.4 (1)                      | 0.34 (2)                              | 2.8 (1)                 |
|                             |          |                    | -91.15 (2)                               | 15:50:20.32 (3)            | -53:57:08.5 (3)                      | 0.33 (4)                              | 1.9 (1)                 |
|                             |          |                    | -89.742 (8)                              | 15:50:20.29 (2)            | -53:57:09.2 (1)                      | 0.60 (2)                              | 3.34 (9)                |
|                             | B        | 36                 | -89.02 (2)                               | 15:50:20.28 (8)            | -53:57:08.7 (6)                      | 0.33 (5)                              | 0.9 (1)                 |
|                             |          |                    | -89.67 (1)                               | 15:50:18.67 (2)            | -53:57:05.4 (1)                      | 0.49 (3)                              | 1.10 (5)                |
|                             |          |                    | -88.17 (5)                               | 15:50:18.34 (4)            | -53:57:06.2 (3)                      | 4.1 (1)                               | 0.76 (2)                |

**Table 3** – *continued*

| Source name                 | Location | Frequency<br>(GHz) | LSR<br>velocity<br>(km s <sup>-1</sup> ) | $\alpha_{2000}$<br>(h:m:s) | $\delta_{2000}$<br>(°:arcmin:arcsec) | Line<br>FWHM<br>(km s <sup>-1</sup> ) | Flux<br>density<br>(Jy) |
|-----------------------------|----------|--------------------|------------------------------------------|----------------------------|--------------------------------------|---------------------------------------|-------------------------|
| G327.39+0.20<br>(continued) | B        | 36                 | -87.40 (2)                               | 15:50:18.16 (4)            | -53:57:07.0 (3)                      | 0.52 (5)                              | 0.59 (5)                |
|                             |          | 44                 | -89.54 (2)                               | 15:50:18.53 (2)            | -53:57:07.1 (2)                      | 1.02 (4)                              | 2.57 (6)                |
|                             |          |                    | -87.97 (3)                               | 15:50:18.40 (5)            | -53:57:08.7 (4)                      | 1.20 (8)                              | 1.31 (6)                |
| G327.62-0.11                | A        | 36                 | -90.1 (2)                                | 15:52:50.1 (1)             | -54:02:59.6 (8)                      | 1.2 (4)                               | 0.18 (3)                |
|                             |          |                    | -89.39 (2)                               | 15:52:50.09 (4)            | -54:02:58.6 (3)                      | 0.38 (8)                              | 0.41 (8)                |
|                             |          |                    | -88.292 (6)                              | 15:52:50.20 (2)            | -54:03:01.6 (2)                      | 0.66 (1)                              | 1.61 (3)                |
|                             |          | 44                 | -88.82 (3)                               | 15:52:50.20 (1)            | -54:03:01.8 (1)                      | 0.32 (8)                              | 3 (1)                   |
|                             |          |                    | -88.39 (3)                               | 15:52:50.24 (2)            | -54:03:01.1 (2)                      | 0.6 (2)                               | 10.1 (7)                |
|                             |          |                    | -87.9 (2)                                | 15:52:50.27 (3)            | -54:03:00.9 (2)                      | 0.5 (2)                               | 2 (2)                   |
|                             |          |                    | -87.28 (1)                               | 15:52:50.37 (1)            | -54:03:06.0 (1)                      | 0.41 (3)                              | 2.3 (1)                 |
|                             | B        | 36                 | -87.1 (1)                                | 15:52:50.31 (6)            | -54:03:06.8 (5)                      | 5.5 (3)                               | 0.22 (1)                |
|                             |          |                    | -87.10 (2)                               | 15:52:50.38 (8)            | -54:03:06.0 (5)                      | 0.20 (4)                              | 0.36 (6)                |
|                             |          |                    |                                          |                            |                                      |                                       |                         |
| G328.21-0.59                | A        | 36                 | -41.727 (8)                              | 15:57:59.38 (2)            | -54:02:15.3 (1)                      | 0.32 (2)                              | 2.1 (1)                 |
|                             |          |                    | -40.816 (4)                              | 15:57:59.600 (6)           | -54:02:11.96 (4)                     | 0.31 (1)                              | 6.2 (4)                 |
|                             |          |                    | -40.732 (3)                              | 15:57:59.600 (6)           | -54:02:11.96 (4)                     | 0.546 (7)                             | 9.7 (1)                 |
|                             |          |                    | -40.62 (2)                               | 15:57:59.48 (6)            | -54:02:12.4 (3)                      | 0.67 (2)                              | 5.3 (3)                 |
|                             |          | 44                 | -42.2 (3)                                | 15:57:59.4 (1)             | -54:02:15 (1)                        | 2.5 (5)                               | 0.8 (1)                 |
|                             |          |                    | -41.934 (2)                              | 15:57:59.35 (2)            | -54:02:15.4 (1)                      | 0.275 (7)                             | 11.5 (2)                |
|                             |          |                    | -41.012 (2)                              | 15:57:59.589 (3)           | -54:02:12.05 (2)                     | 0.45 (1)                              | 30 (1)                  |
|                             | A        |                    | -40.55 (4)                               | 15:57:59.58 (1)            | -54:02:11.89 (9)                     | 0.95 (5)                              | 11.8 (4)                |
|                             |          | 36                 | -41.76 (6)                               | 15:57:58.46 (5)            | -53:59:22.1 (3)                      | 0.8 (1)                               | 0.38 (3)                |
|                             |          |                    | -40.99 (6)                               | 15:57:58.3 (1)             | -53:59:19.4 (7)                      | 0.5 (1)                               | 0.31 (4)                |
|                             |          | 44                 | -41.80 (2)                               | 15:57:58.53 (4)            | -53:59:19.4 (2)                      | 0.17 (4)                              | 1.1 (2)                 |
|                             |          |                    | -41.41 (1)                               | 15:57:58.280 (9)           | -53:59:18.01 (6)                     | 0.28 (6)                              | 3 (1)                   |
|                             |          |                    | -41.27 (3)                               | 15:57:58.28 (1)            | -53:59:18.04 (8)                     | 0.50 (2)                              | 8 (1)                   |
|                             | B        | 36                 | -43.45 (1)                               | 15:57:58.20 (5)            | -53:59:31.8 (3)                      | 0.15 (3)                              | 0.42 (8)                |
|                             |          | 44                 | -44.82 (8)                               | 15:57:58.24 (9)            | -53:59:32.6 (5)                      | 0.4 (1)                               | 0.6 (1)                 |
|                             |          |                    | -44.32 (4)                               | 15:57:58.32 (2)            | -53:59:32.1 (1)                      | 0.5 (1)                               | 1.18 (9)                |
| G328.24-0.55                | B        |                    | -43.697 (8)                              | 15:57:58.30 (2)            | -53:59:32.2 (1)                      | 0.41 (2)                              | 3.23 (9)                |
|                             |          | 36                 | -45.02 (2)                               | 15:58:04.20 (4)            | -53:58:45.4 (3)                      | 0.51 (6)                              | 2.3 (2)                 |
|                             |          |                    |                                          |                            |                                      |                                       |                         |
|                             | C        | 36                 | -45.02 (2)                               | 15:58:04.20 (4)            | -53:58:45.4 (3)                      | 0.51 (6)                              | 2.3 (2)                 |
|                             |          |                    |                                          |                            |                                      |                                       |                         |
|                             |          |                    |                                          |                            |                                      |                                       |                         |
|                             | A        | 44                 | -45.21 (3)                               | 15:57:59.10 (4)            | -53:57:51.4 (3)                      | 0.29 (6)                              | 0.53 (9)                |
|                             |          |                    | -44.572 (3)                              | 15:57:59.074 (9)           | -53:57:52.84 (6)                     | 0.210 (6)                             | 4.2 (1)                 |
|                             |          |                    |                                          |                            |                                      |                                       |                         |
|                             | B        | 36                 | -45.665 (4)                              | 15:57:59.82 (2)            | -53:57:17.0 (1)                      | 0.33 (1)                              | 4.0 (1)                 |
|                             |          |                    | -44.98 (8)                               | 15:57:59.88 (5)            | -53:57:16.8 (4)                      | 2.4 (2)                               | 0.64 (5)                |
|                             |          | 44                 | -45.89 (1)                               | 15:57:59.90 (1)            | -53:57:17.02 (8)                     | 0.38 (3)                              | 7.2 (4)                 |
| G328.25-0.53                |          |                    | -45.19 (3)                               | 15:57:59.87 (4)            | -53:57:16.6 (3)                      | 0.4 (2)                               | 2 (1)                   |
|                             |          |                    | -44.6 (3)                                | 15:57:59.88 (8)            | -53:57:17.5 (4)                      | 1.2 (9)                               | 1.3 (2)                 |
|                             |          |                    | -43.63 (2)                               | 15:58:00.01 (2)            | -53:57:16.6 (2)                      | 0.45 (5)                              | 3.3 (4)                 |
|                             | C        | 44                 | -48.12 (2)                               | 15:58:05.12 (6)            | -53:57:34.4 (3)                      | 0.45 (4)                              | 5.1 (4)                 |
|                             | D        | 36                 | -45.66 (1)                               | 15:57:58.98 (4)            | -53:57:14.4 (3)                      | 0.25 (4)                              | 1.8 (3)                 |
|                             |          |                    | -45.27 (1)                               | 15:57:58.98 (2)            | -53:57:14.9 (1)                      | 0.58 (2)                              | 5.70 (9)                |
|                             |          |                    |                                          |                            |                                      |                                       |                         |
|                             | E        | 36                 | -44.12 (2)                               | 15:58:02.20 (4)            | -53:57:06.0 (3)                      | 0.47 (4)                              | 2.5 (2)                 |
|                             | F        | 36                 | -46.94 (8)                               | 15:58:05.45 (9)            | -53:57:51.4 (7)                      | 1.8 (2)                               | 0.86 (8)                |
|                             | A        | 36                 | -42.09 (2)                               | 15:55:50.31 (8)            | -52:43:22.1 (5)                      | 1.05 (6)                              | 1.5 (2)                 |
|                             |          |                    | -42.049 (9)                              | 15:55:50.176 (7)           | -52:43:21.24 (4)                     | 0.44 (4)                              | 1.5 (2)                 |
|                             |          | 44                 | -42.92 (3)                               | 15:55:50.11 (2)            | -52:43:20.8 (1)                      | 0.34 (6)                              | 1.5 (3)                 |
|                             |          |                    | -42.458 (2)                              | 15:55:50.105 (3)           | -52:43:20.87 (1)                     | 0.528 (9)                             | 23.5 (6)                |
| G328.81+0.63                | A        |                    | -42.29 (2)                               | 15:55:50.12 (2)            | -52:43:21.3 (1)                      | 1.03 (2)                              | 12.1 (5)                |
|                             |          |                    |                                          |                            |                                      |                                       |                         |

Table 3 – continued

| Source name                 | Location | Frequency<br>(GHz) | LSR<br>velocity<br>(km s <sup>-1</sup> ) | $\alpha_{2000}$<br>(h:m:s) | $\delta_{2000}$<br>(°:arcmin:arcsec) | Line<br>FWHM<br>(km s <sup>-1</sup> ) | Flux<br>density<br>(Jy) |
|-----------------------------|----------|--------------------|------------------------------------------|----------------------------|--------------------------------------|---------------------------------------|-------------------------|
| G328.81+0.63<br>(continued) | B        | 44                 | -43.3 (1)                                | 15:55:49.09 (8)            | -52:43:22.7 (4)                      | 0.8 (1)                               | 2.3 (3)                 |
|                             |          |                    | -42.854 (3)                              | 15:55:49.102 (9)           | -52:43:22.77 (5)                     | 0.46 (1)                              | 10.3 (7)                |
|                             |          |                    | -41.98 (2)                               | 15:55:49.13 (4)            | -52:43:22.9 (2)                      | 0.43 (4)                              | 0.93 (8)                |
|                             | C        | 36                 | -40.38 (1)                               | 15:55:48.45 (2)            | -52:43:19.4 (1)                      | 0.47 (4)                              | 1.2 (1)                 |
|                             |          |                    | -40.26 (5)                               | 15:55:48.42 (8)            | -52:43:19.0 (4)                      | 1.2 (2)                               | 0.4 (1)                 |
|                             |          | 44                 | -41.49 (2)                               | 15:55:48.15 (2)            | -52:43:18.9 (1)                      | 0.64 (5)                              | 1.6 (1)                 |
|                             |          |                    | -40.97 (8)                               | 15:55:48.5 (1)             | -52:43:20.1 (7)                      | 3.2 (3)                               | 0.8 (1)                 |
|                             |          |                    | -40.555 (4)                              | 15:55:48.444 (4)           | -52:43:18.88 (2)                     | 0.55 (1)                              | 17 (1)                  |
|                             |          |                    | -40.505 (3)                              | 15:55:48.427 (5)           | -52:43:18.89 (3)                     | 0.30 (1)                              | 9 (1)                   |
|                             |          |                    | -39.839 (6)                              | 15:55:48.45 (3)            | -52:43:19.0 (2)                      | 0.33 (2)                              | 2.6 (1)                 |
|                             |          |                    | -41.174 (3)                              | 15:55:47.17 (2)            | -52:43:14.27 (9)                     | 0.529 (8)                             | 5.86 (8)                |
|                             | E        | 44                 | -40.7 (4)                                | 15:55:49.3 (1)             | -52:42:57 (1)                        | 4.5 (8)                               | 0.20 (3)                |
|                             |          |                    | -39.432 (8)                              | 15:55:49.35 (1)            | -52:42:58.93 (8)                     | 0.35 (2)                              | 2.6 (1)                 |
|                             | F        | 36                 | -39.00 (2)                               | 15:55:49.23 (5)            | -52:42:58.8 (3)                      | 0.24 (5)                              | 0.9 (1)                 |
|                             |          |                    | -43.32 (3)                               | 15:55:50.15 (8)            | -52:42:31.6 (5)                      | 0.6 (1)                               | 1.7 (5)                 |
|                             |          |                    | -42.9 (1)                                | 15:55:49.8 (2)             | -52:42:30 (1)                        | 2.0 (5)                               | 0.9 (6)                 |
|                             |          |                    | -42.51 (3)                               | 15:55:50.11 (3)            | -52:42:29.6 (2)                      | 0.52 (5)                              | 3.7 (6)                 |
|                             |          |                    | -42.338 (8)                              | 15:55:50.09 (3)            | -52:42:29.9 (2)                      | 0.18 (3)                              | 3.3 (5)                 |
|                             | G        | 36                 | -42.26 (1)                               | 15:55:49.80 (1)            | -52:42:44.63 (8)                     | 0.35 (2)                              | 1.55 (9)                |
|                             | H        | 36                 | -40.653 (8)                              | 15:55:48.28 (2)            | -52:43:36.9 (2)                      | 0.26 (2)                              | 1.12 (8)                |
|                             | I        | 36                 | -40.72 (8)                               | 15:55:50.32 (6)            | -52:43:30.1 (4)                      | 2.4 (2)                               | 0.35 (3)                |
|                             | J        | 36                 | -43.86 (6)                               | 15:55:48.43 (5)            | -52:43:05.7 (3)                      | 0.8 (2)                               | 0.41 (6)                |
| G329.03-0.20                | A        | 36                 | -47.248 (2)                              | 16:00:30.156 (5)           | -53:12:28.89 (4)                     | 0.209 (3)                             | 9.12 (8)                |
|                             |          |                    | -46.969 (1)                              | 16:00:30.223 (2)           | -53:12:28.71 (1)                     | 0.2199 (9)                            | 33.87 (8)               |
|                             |          |                    | -46.551 (1)                              | 16:00:30.224 (3)           | -53:12:28.81 (2)                     | 0.281 (2)                             | 12.74 (8)               |
|                             |          |                    | -46.00 (1)                               | 16:00:30.28 (2)            | -53:12:28.8 (1)                      | 0.55 (3)                              | 1.40 (5)                |
|                             |          |                    | -44.9 (2)                                | 16:00:30.3 (1)             | -53:12:28.5 (9)                      | 4.6 (3)                               | 0.30 (2)                |
|                             |          | 44                 | -47.489 (2)                              | 16:00:30.18 (1)            | -53:12:28.79 (8)                     | 0.195 (5)                             | 10.0 (2)                |
|                             |          |                    | -47.197 (1)                              | 16:00:30.267 (2)           | -53:12:28.59 (1)                     | 0.222 (1)                             | 60.9 (2)                |
|                             |          |                    | -46.790 (1)                              | 16:00:30.264 (2)           | -53:12:28.73 (1)                     | 0.375 (3)                             | 33.9 (1)                |
|                             |          |                    | -46.303 (3)                              | 16:00:30.25 (1)            | -53:12:28.73 (8)                     | 0.31 (1)                              | 7.9 (1)                 |
|                             |          |                    | -45.96 (1)                               | 16:00:30.27 (2)            | -53:12:28.7 (2)                      | 0.20 (3)                              | 1.7 (2)                 |
|                             | B        | 36                 | -47.69 (2)                               | 16:00:30.22 (5)            | -53:12:10.8 (4)                      | 1.02 (5)                              | 0.85 (4)                |
|                             |          |                    | -46.20 (2)                               | 16:00:30.2 (1)             | -53:12:13.3 (6)                      | 0.43 (4)                              | 1.16 (6)                |
|                             |          |                    | -45.657 (6)                              | 16:00:30.38 (2)            | -53:12:13.3 (1)                      | 0.41 (2)                              | 3.11 (6)                |
|                             |          |                    | -44.90 (2)                               | 16:00:30.60 (4)            | -53:12:12.3 (3)                      | 0.70 (6)                              | 1.19 (6)                |
|                             |          |                    | -43.6 (2)                                | 16:00:30.6 (1)             | -53:12:14.8 (7)                      | 1.6 (4)                               | 0.24 (3)                |
|                             |          |                    | -46.40 (1)                               | 16:00:30.40 (2)            | -53:12:13.5 (2)                      | 0.31 (3)                              | 2.6 (1)                 |
|                             |          |                    | -45.861 (8)                              | 16:00:30.47 (1)            | -53:12:13.73 (8)                     | 0.48 (2)                              | 6.2 (2)                 |
|                             |          |                    | -45.17 (4)                               | 16:00:30.64 (3)            | -53:12:13.2 (2)                      | 0.74 (8)                              | 2.0 (1)                 |
|                             | C        | 36                 | -46.718 (2)                              | 16:00:29.84 (1)            | -53:12:13.87 (9)                     | 0.209 (3)                             | 7.52 (8)                |
|                             |          |                    | -46.327 (5)                              | 16:00:29.71 (2)            | -53:12:19.0 (1)                      | 0.33 (2)                              | 2.35 (8)                |
|                             |          |                    | -45.93 (1)                               | 16:00:30.02 (4)            | -53:12:12.8 (3)                      | 0.20 (4)                              | 0.9 (3)                 |
|                             |          |                    | -45.68 (8)                               | 16:00:30.27 (6)            | -53:12:13.0 (3)                      | 0.4 (1)                               | 0.67 (9)                |
|                             |          | 44                 | -46.979 (7)                              | 16:00:29.88 (2)            | -53:12:14.0 (2)                      | 0.13 (1)                              | 3.8 (3)                 |
|                             |          |                    | -46.80 (1)                               | 16:00:29.89 (3)            | -53:12:16.1 (2)                      | 0.20 (3)                              | 3.6 (2)                 |
|                             |          |                    | -46.46 (1)                               | 16:00:29.72 (4)            | -53:12:19.7 (3)                      | 0.25 (2)                              | 2.6 (2)                 |
|                             | D        | 44                 | -45.41 (1)                               | 16:00:30.80 (1)            | -53:12:20.4 (1)                      | 0.29 (3)                              | 1.7 (1)                 |

**Table 3** – *continued*

| Source name                 | Location | Frequency<br>(GHz) | LSR<br>velocity<br>(km s <sup>-1</sup> ) | $\alpha_{2000}$<br>(h:m:s) | $\delta_{2000}$<br>(°:arcmin:arcsec) | Line<br>FWHM<br>(km s <sup>-1</sup> ) | Flux<br>density<br>(Jy) |
|-----------------------------|----------|--------------------|------------------------------------------|----------------------------|--------------------------------------|---------------------------------------|-------------------------|
| G329.03-0.20<br>(continued) | E        | 36                 | -41.0 (2)                                | 16:00:30.3 (1)             | -53:12:52.8 (8)                      | 1.4 (3)                               | 0.49 (8)                |
|                             |          |                    | -39.58 (8)                               | 16:00:30.34 (6)            | -53:12:51.0 (4)                      | 1.3 (4)                               | 0.79 (6)                |
|                             |          |                    | -38.45 (4)                               | 16:00:30.44 (4)            | -53:12:50.0 (3)                      | 0.8 (1)                               | 0.8 (1)                 |
|                             |          |                    | -37.4 (1)                                | 16:00:30.67 (8)            | -53:12:50.4 (5)                      | 0.8 (2)                               | 0.23 (4)                |
|                             | F        | 36                 | -43.985 (7)                              | 16:00:31.96 (2)            | -53:12:45.4 (1)                      | 0.42 (1)                              | 2.83 (6)                |
|                             |          |                    | -43.448 (8)                              | 16:00:31.93 (1)            | -53:12:45.7 (1)                      | 0.53 (2)                              | 3.28 (5)                |
|                             |          |                    | -42.33 (1)                               | 16:00:31.84 (8)            | -53:12:46.7 (5)                      | 0.68 (4)                              | 1.13 (5)                |
|                             |          |                    | -42.30 (9)                               | 16:00:31.9 (1)             | -53:12:46.1 (8)                      | 4.0 (2)                               | 0.52 (4)                |
|                             |          |                    | -40.305 (8)                              | 16:00:31.97 (3)            | -53:12:45.4 (2)                      | 0.30 (2)                              | 1.02 (6)                |
|                             |          |                    | -44.326 (9)                              | 16:00:31.99 (3)            | -53:12:45.3 (2)                      | 0.58 (2)                              | 7.5 (1)                 |
|                             |          | 44                 | -43.647 (3)                              | 16:00:31.953 (3)           | -53:12:45.69 (2)                     | 0.643 (6)                             | 27.7 (1)                |
|                             |          |                    | -42.458 (7)                              | 16:00:31.80 (3)            | -53:12:47.3 (2)                      | 0.76 (2)                              | 7.36 (8)                |
|                             |          |                    | -41.944 (8)                              | 16:00:31.93 (9)            | -53:12:46.3 (7)                      | 0.23 (2)                              | 2.5 (2)                 |
|                             |          |                    | -41.29 (4)                               | 16:00:31.98 (6)            | -53:12:45.9 (4)                      | 0.7 (1)                               | 0.84 (9)                |
|                             |          |                    | -40.518 (3)                              | 16:00:31.96 (2)            | -53:12:45.6 (1)                      | 0.328 (7)                             | 6.9 (1)                 |
|                             |          |                    | -44.63 (3)                               | 16:00:31.72 (2)            | -53:12:51.0 (1)                      | 1.50 (8)                              | 0.89 (5)                |
|                             | G        | 36                 | -42.4 (2)                                | 16:00:31.7 (3)             | -53:12:54 (2)                        | 3.0 (6)                               | 0.29 (2)                |
|                             |          |                    | -41.35 (2)                               | 16:00:31.9 (1)             | -53:12:53.4 (7)                      | 0.32 (4)                              | 0.50 (6)                |
|                             |          |                    | -40.04 (3)                               | 16:00:31.71 (5)            | -53:12:54.3 (3)                      | 0.49 (8)                              | 0.38 (5)                |
|                             |          | 44                 | -44.49 (2)                               | 16:00:31.76 (5)            | -53:12:51.3 (3)                      | 0.39 (6)                              | 1.0 (1)                 |
|                             |          |                    | -41.55 (1)                               | 16:00:31.93 (6)            | -53:12:52.4 (4)                      | 0.31 (3)                              | 1.9 (1)                 |
|                             |          |                    | -40.44 (1)                               | 16:00:31.84 (2)            | -53:12:53.0 (1)                      | 0.80 (3)                              | 2.90 (8)                |
|                             |          |                    | -38.86 (1)                               | 16:00:32.06 (2)            | -53:12:53.2 (1)                      | 0.22 (3)                              | 1.5 (2)                 |
|                             |          |                    | -37.989 (5)                              | 16:00:31.95 (1)            | -53:12:54.90 (8)                     | 0.48 (1)                              | 5.2 (1)                 |
|                             | H        | 36                 | -43.1 (2)                                | 16:00:31.8 (1)             | -53:12:57.5 (9)                      | 5.9 (4)                               | 0.26 (3)                |
|                             |          |                    | -42.10 (4)                               | 16:00:31.80 (8)            | -53:12:57.9 (6)                      | 1.6 (1)                               | 0.73 (4)                |
|                             |          |                    | -41.55 (1)                               | 16:00:31.85 (4)            | -53:12:58.1 (3)                      | 0.23 (3)                              | 0.76 (8)                |
|                             |          |                    | -40.69 (1)                               | 16:00:31.78 (4)            | -53:12:57.2 (3)                      | 0.31 (3)                              | 0.90 (6)                |
|                             |          | 44                 | -41.773 (5)                              | 16:00:31.86 (2)            | -53:12:57.4 (1)                      | 0.35 (1)                              | 4.3 (1)                 |
|                             |          |                    | -45.168 (1)                              | 16:00:30.145 (3)           | -53:12:34.61 (2)                     | 0.256 (2)                             | 7.85 (5)                |
|                             | I        | 36                 | -44.43 (1)                               | 16:01:06.77 (4)            | -53:16:22.8 (3)                      | 0.45 (3)                              | 2.0 (1)                 |
|                             |          | 36                 | -43.892 (7)                              | 16:01:06.82 (3)            | -53:16:22.8 (2)                      | 0.37 (2)                              | 2.9 (1)                 |
| G329.07-0.31                | A        | 36                 | -43.86 (3)                               | 16:01:06.7 (2)             | -53:16:23.0 (9)                      | 2.1 (1)                               | 1.4 (1)                 |
|                             |          |                    | -43.42 (3)                               | 16:01:07.02 (3)            | -53:16:22.4 (2)                      | 0.22 (8)                              | 0.4 (1)                 |
|                             |          |                    | -40.87 (3)                               | 16:01:07.27 (6)            | -53:16:25.4 (3)                      | 0.90 (8)                              | 0.68 (5)                |
|                             |          |                    | -44.73 (6)                               | 16:01:06.72 (5)            | -53:16:23.9 (4)                      | 1.7 (1)                               | 1.1 (2)                 |
|                             |          | 44                 | -44.56 (5)                               | 16:01:06.70 (2)            | -53:16:22.9 (1)                      | 0.5 (1)                               | 0.8 (2)                 |
|                             |          |                    | -44.109 (9)                              | 16:01:06.72 (2)            | -53:16:23.5 (1)                      | 0.26 (2)                              | 2.7 (2)                 |
|                             |          |                    | -43.971 (9)                              | 16:01:07.80 (2)            | -53:15:53.5 (1)                      | 0.59 (2)                              | 2.02 (6)                |
|                             |          |                    | -42.78 (1)                               | 16:01:12.55 (4)            | -53:16:00.7 (3)                      | 0.18 (3)                              | 0.7 (1)                 |
|                             | B        | 36                 | -42.18 (2)                               | 16:01:12.44 (3)            | -53:16:01.9 (2)                      | 0.63 (6)                              | 1.53 (6)                |
|                             |          |                    | -41.51 (3)                               | 16:01:12.44 (2)            | -53:16:01.8 (1)                      | 0.48 (6)                              | 0.96 (8)                |
|                             |          |                    | -39.5 (2)                                | 16:01:12.4 (1)             | -53:16:00 (1)                        | 5.8 (3)                               | 0.38 (2)                |
|                             |          |                    | -43.12 (2)                               | 16:01:12.36 (2)            | -53:15:59.8 (2)                      | 0.68 (5)                              | 1.36 (9)                |
|                             | C        | 36                 | -50.68 (2)                               | 16:01:09.03 (4)            | -53:16:07.0 (3)                      | 0.26 (4)                              | 0.43 (6)                |
|                             |          |                    | -48.08 (6)                               | 16:01:09.02 (4)            | -53:16:06.2 (2)                      | 2.5 (1)                               | 0.39 (2)                |
|                             |          |                    | -41.934 (6)                              | 16:01:08.89 (2)            | -53:16:08.0 (1)                      | 0.26 (2)                              | 1.34 (6)                |
|                             |          |                    | -41.3 (1)                                | 16:01:09.01 (8)            | -53:16:06.3 (4)                      | 0.6 (2)                               | 0.5 (1)                 |

Table 3 – continued

| Source name                 | Location | Frequency (GHz) | LSR velocity (km s <sup>-1</sup> ) | $\alpha_{2000}$ (h:m:s) | $\delta_{2000}$ (°:arcmin:arcsec) | Line FWHM (km s <sup>-1</sup> ) | Flux density (Jy) |
|-----------------------------|----------|-----------------|------------------------------------|-------------------------|-----------------------------------|---------------------------------|-------------------|
| G329.07-0.31<br>(continued) | D        | 36              | -40.73 (4)                         | 16:01:09.06 (2)         | -53:16:06.2 (1)                   | 0.5 (1)                         | 1.3 (2)           |
|                             |          |                 | -40.01 (3)                         | 16:01:08.89 (3)         | -53:16:06.6 (2)                   | 0.7 (2)                         | 1.26 (5)          |
|                             |          |                 | -39.5 (1)                          | 16:01:08.85 (8)         | -53:16:06.6 (4)                   | 0.4 (2)                         | 0.3 (2)           |
|                             |          |                 | -38.6 (3)                          | 16:01:08.9 (1)          | -53:16:08.1 (6)                   | 4.9 (6)                         | 0.32 (2)          |
|                             |          |                 | -35.14 (3)                         | 16:01:09.06 (5)         | -53:16:08.1 (3)                   | 0.37 (8)                        | 0.28 (5)          |
|                             |          |                 | -32.51 (3)                         | 16:01:09.02 (4)         | -53:16:07.6 (3)                   | 0.32 (8)                        | 0.24 (5)          |
|                             |          |                 | -32.3 (2)                          | 16:01:08.90 (8)         | -53:16:08.6 (4)                   | 5.8 (5)                         | 0.33 (1)          |
|                             |          |                 | -28.39 (3)                         | 16:01:08.94 (5)         | -53:16:08.0 (3)                   | 0.48 (8)                        | 0.30 (4)          |
|                             |          | 44              | -42.73 (1)                         | 16:01:08.88 (3)         | -53:16:07.8 (2)                   | 0.28 (3)                        | 1.07 (8)          |
|                             |          |                 | -42.130 (2)                        | 16:01:08.868 (7)        | -53:16:07.90 (6)                  | 0.339 (6)                       | 5.41 (8)          |
|                             |          |                 | -41.0 (1)                          | 16:01:09.04 (8)         | -53:16:06.6 (6)                   | 3.5 (2)                         | 0.48 (3)          |
|                             |          |                 | -40.72 (4)                         | 16:01:09.05 (3)         | -53:16:05.9 (2)                   | 0.4 (1)                         | 0.30 (8)          |
|                             | E        | 36              | -45.66 (2)                         | 16:01:10.53 (4)         | -53:16:18.0 (2)                   | 0.12 (8)                        | 0.2 (1)           |
|                             |          |                 | -45.3 (8)                          | 16:01:10.7 (1)          | -53:16:17.7 (7)                   | 1 (1)                           | 0.3 (2)           |
|                             |          |                 | -44.72 (4)                         | 16:01:10.53 (4)         | -53:16:17.8 (2)                   | 0.7 (2)                         | 1.1 (5)           |
|                             |          |                 | -44.27 (2)                         | 16:01:10.59 (1)         | -53:16:17.25 (9)                  | 0.32 (4)                        | 1.1 (2)           |
|                             |          |                 | -43.54 (2)                         | 16:01:10.61 (3)         | -53:16:16.6 (2)                   | 1.01 (6)                        | 1.46 (6)          |
|                             |          |                 | -43.3 (3)                          | 16:01:10.7 (1)          | -53:16:11.1 (9)                   | 5.5 (6)                         | 0.24 (4)          |
|                             |          |                 | -42.73 (2)                         | 16:01:10.55 (5)         | -53:16:12.2 (3)                   | 0.14 (4)                        | 0.5 (2)           |
|                             |          |                 | -42.51 (5)                         | 16:01:10.71 (8)         | -53:16:11.8 (5)                   | 0.3 (1)                         | 0.41 (8)          |
|                             | F        | 36              | -40.885 (7)                        | 16:01:10.05 (4)         | -53:15:53.3 (2)                   | 0.35 (2)                        | 1.42 (6)          |
|                             |          |                 | -39.21 (2)                         | 16:01:09.67 (2)         | -53:15:51.1 (1)                   | 0.72 (5)                        | 0.82 (4)          |
| G329.18-0.31                | A        | 44              | -56.08 (3)                         | 16:01:46.31 (6)         | -53:11:58.3 (5)                   | 0.50 (6)                        | 0.71 (8)          |
|                             | B        | 36              | -55.81 (4)                         | 16:01:44.54 (4)         | -53:11:26.8 (2)                   | 0.68 (9)                        | 0.81 (6)          |
|                             |          |                 | -55.119 (7)                        | 16:01:44.59 (1)         | -53:11:26.58 (8)                  | 0.44 (2)                        | 3.10 (8)          |
|                             |          |                 | -53.58 (4)                         | 16:01:44.62 (5)         | -53:11:26.6 (3)                   | 0.43 (9)                        | 0.40 (8)          |
|                             |          |                 | -53.2 (3)                          | 16:01:44.6 (1)          | -53:11:26.3 (9)                   | 6.4 (6)                         | 0.26 (2)          |
|                             |          |                 | -50.061 (2)                        | 16:01:44.729 (3)        | -53:11:27.09 (2)                  | 0.564 (6)                       | 7.95 (6)          |
|                             |          |                 | -49.38 (1)                         | 16:01:44.75 (6)         | -53:11:26.0 (4)                   | 0.30 (3)                        | 0.94 (8)          |
|                             |          | 44              | -54.86 (3)                         | 16:01:44.65 (5)         | -53:11:25.9 (4)                   | 0.83 (8)                        | 0.84 (8)          |
|                             |          |                 | -50.288 (2)                        | 16:01:44.733 (9)        | -53:11:27.12 (6)                  | 0.534 (4)                       | 20.0 (1)          |
|                             |          |                 | -49.610 (4)                        | 16:01:44.64 (3)         | -53:11:26.2 (2)                   | 0.423 (9)                       | 6.9 (1)           |
|                             |          |                 | -49.5 (1)                          | 16:01:45.0 (1)          | -53:11:27.8 (7)                   | 4.5 (3)                         | 0.58 (5)          |
|                             | C        | 36              | -49.304 (6)                        | 16:01:46.62 (3)         | -53:11:50.8 (2)                   | 0.31 (1)                        | 1.38 (5)          |
|                             |          |                 | -48.251 (5)                        | 16:01:46.90 (2)         | -53:11:52.66 (9)                  | 0.17 (1)                        | 1.25 (8)          |
|                             |          | 44              | -51.62 (1)                         | 16:01:46.78 (2)         | -53:11:48.4 (1)                   | 0.38 (4)                        | 0.99 (8)          |
|                             |          |                 | -51.000 (7)                        | 16:01:46.77 (1)         | -53:11:48.6 (1)                   | 0.47 (2)                        | 2.27 (9)          |
|                             |          |                 | -49.9 (1)                          | 16:01:46.72 (9)         | -53:11:49.0 (6)                   | 1.6 (3)                         | 0.43 (5)          |
|                             |          |                 | -49.520 (6)                        | 16:01:46.56 (1)         | -53:11:49.92 (8)                  | 0.28 (2)                        | 1.88 (9)          |
|                             | D        | 36              | -47.86 (2)                         | 16:01:48.24 (4)         | -53:11:46.4 (2)                   | 0.92 (5)                        | 0.73 (3)          |
|                             |          |                 | -49.71 (8)                         | 16:01:48.30 (8)         | -53:11:48.2 (6)                   | 1.7 (2)                         | 0.47 (4)          |
|                             |          | 44              | -48.023 (7)                        | 16:01:48.230 (9)        | -53:11:46.46 (8)                  | 0.71 (2)                        | 2.97 (6)          |
|                             |          |                 | -45.16 (4)                         | 16:01:48.43 (8)         | -53:11:47.5 (5)                   | 0.6 (1)                         | 0.43 (6)          |
|                             | E        | 36              | -47.82 (9)                         | 16:01:47.36 (8)         | -53:11:42.5 (4)                   | 2.0 (2)                         | 0.25 (2)          |
|                             |          |                 | -48.8 (2)                          | 16:01:47.4 (1)          | -53:11:42.5 (9)                   | 2.6 (4)                         | 0.40 (3)          |
|                             |          | 44              | -47.967 (9)                        | 16:01:47.43 (2)         | -53:11:42.2 (2)                   | 0.32 (3)                        | 1.26 (9)          |
|                             |          |                 | -47.06 (2)                         | 16:01:47.15 (8)         | -53:11:40.8 (6)                   | 0.72 (5)                        | 1.14 (8)          |
|                             | F        | 44              | -49.977 (4)                        | 16:01:47.095 (9)        | -53:11:55.65 (8)                  | 0.233 (9)                       | 2.98 (9)          |

**Table 3** – *continued*

| Source<br>name              | Location | Frequency<br>(GHz) | LSR<br>velocity<br>(km s <sup>-1</sup> ) | $\alpha_{2000}$<br>(h:m:s) | $\delta_{2000}$<br>(°:arcmin:arcsec) | Line<br>FWHM<br>(km s <sup>-1</sup> ) | Flux<br>density<br>(Jy) |
|-----------------------------|----------|--------------------|------------------------------------------|----------------------------|--------------------------------------|---------------------------------------|-------------------------|
| G329.18-0.31<br>(continued) | F        | 44                 | -49.2 (1)                                | 16:01:47.05 (8)            | -53:11:55.3 (6)                      | 2.7 (2)                               | 0.35 (3)                |
|                             | G        | 44                 | -75.89 (4)                               | 16:01:45.67 (4)            | -53:11:35.4 (3)                      | 0.34 (9)                              | 0.33 (8)                |
|                             |          |                    | -49.944 (3)                              | 16:01:45.71 (1)            | -53:11:33.87 (8)                     | 0.223 (7)                             | 3.7 (1)                 |
|                             |          |                    | -48.43 (8)                               | 16:01:45.65 (5)            | -53:11:32.8 (4)                      | 2.0 (2)                               | 0.49 (3)                |
|                             | H        | 36                 | -59.61 (2)                               | 16:01:43.21 (8)            | -53:11:20.3 (4)                      | 0.21 (5)                              | 0.8 (1)                 |
|                             |          |                    | -58.12 (2)                               | 16:01:43.33 (2)            | -53:11:20.2 (1)                      | 0.45 (8)                              | 1.6 (2)                 |
|                             |          |                    | -57.67 (2)                               | 16:01:43.36 (1)            | -53:11:20.09 (6)                     | 0.28 (6)                              | 1.3 (2)                 |
|                             |          |                    | -57.55 (6)                               | 16:01:43.27 (6)            | -53:11:20.0 (3)                      | 2.1 (2)                               | 1.4 (3)                 |
|                             |          |                    | -57.228 (9)                              | 16:01:43.330 (7)           | -53:11:20.19 (4)                     | 0.47 (3)                              | 4.5 (2)                 |
|                             |          |                    | -52.5 (3)                                | 16:01:43.2 (1)             | -53:11:20.7 (7)                      | 5.6 (7)                               | 0.37 (3)                |
|                             |          | 44                 | -57.0 (1)                                | 16:01:43.4 (1)             | -53:11:20.6 (7)                      | 1.6 (2)                               | 0.8 (1)                 |
|                             |          |                    | -49.94 (1)                               | 16:01:43.31 (1)            | -53:11:19.51 (8)                     | 0.33 (3)                              | 2.8 (2)                 |
|                             |          |                    | -48.73 (8)                               | 16:01:43.32 (3)            | -53:11:18.7 (3)                      | 3.0 (2)                               | 1.63 (8)                |
|                             | I        | 36                 | -48.44 (3)                               | 16:01:46.99 (5)            | -53:11:31.1 (3)                      | 0.26 (8)                              | 0.36 (8)                |
|                             |          |                    | -47.99 (2)                               | 16:01:46.48 (4)            | -53:11:30.9 (2)                      | 0.39 (5)                              | 0.82 (8)                |
|                             |          |                    | -47.76 (9)                               | 16:01:46.6 (1)             | -53:11:32.5 (8)                      | 2.4 (2)                               | 0.41 (4)                |
|                             |          |                    | -45.36 (1)                               | 16:01:46.39 (2)            | -53:11:30.8 (1)                      | 0.67 (3)                              | 1.96 (4)                |
|                             |          |                    | -44.55 (1)                               | 16:01:46.37 (3)            | -53:11:30.3 (2)                      | 0.53 (3)                              | 1.61 (5)                |
|                             | J        | 36                 | -50.35 (6)                               | 16:01:44.98 (5)            | -53:11:48.3 (3)                      | 2.9 (1)                               | 0.55 (2)                |
|                             | K        | 36                 | -49.03 (2)                               | 16:01:50.13 (4)            | -53:11:44.4 (2)                      | 1.75 (4)                              | 1.82 (3)                |
| G329.47+0.50                | A        | 36                 | -67.92 (2)                               | 15:59:40.62 (9)            | -52:23:02.9 (7)                      | 0.35 (4)                              | 0.53 (6)                |
|                             |          |                    | -66.211 (9)                              | 15:59:40.77 (2)            | -52:23:04.2 (2)                      | 0.32 (2)                              | 1.11 (6)                |
|                             |          | 44                 | -68.28 (8)                               | 15:59:40.86 (6)            | -52:23:04.3 (4)                      | 1.1 (2)                               | 0.6 (1)                 |
|                             |          |                    | -68.19 (2)                               | 15:59:40.81 (4)            | -52:23:04.3 (3)                      | 0.28 (6)                              | 1.0 (2)                 |
|                             |          |                    | -66.454 (6)                              | 15:59:40.76 (1)            | -52:23:03.98 (8)                     | 0.31 (1)                              | 5.8 (1)                 |
|                             |          |                    | -66.04 (6)                               | 15:59:40.91 (5)            | -52:23:04.0 (4)                      | 0.4 (1)                               | 0.6 (1)                 |
|                             | B        | 36                 | -66.490 (5)                              | 15:59:40.13 (2)            | -52:23:34.7 (2)                      | 0.28 (1)                              | 1.52 (5)                |
|                             |          | 44                 | -69.08 (1)                               | 15:59:40.54 (8)            | -52:23:33.0 (5)                      | 0.24 (2)                              | 1.3 (1)                 |
|                             |          |                    | -66.745 (4)                              | 15:59:40.15 (1)            | -52:23:34.03 (8)                     | 0.300 (9)                             | 3.5 (1)                 |
|                             | C        | 36                 | -67.11 (2)                               | 15:59:40.04 (5)            | -52:23:29.3 (4)                      | 0.36 (5)                              | 0.38 (5)                |
|                             |          | 44                 | -68.00 (2)                               | 15:59:40.15 (6)            | -52:23:28.4 (4)                      | 0.37 (4)                              | 0.81 (8)                |
|                             |          |                    | -67.27 (2)                               | 15:59:40.11 (6)            | -52:23:29.0 (4)                      | 0.34 (4)                              | 0.86 (8)                |
|                             |          |                    | -65.64 (3)                               | 15:59:40.09 (4)            | -52:23:28.9 (3)                      | 0.31 (8)                              | 0.39 (9)                |
|                             | D        | 44                 | -67.32 (1)                               | 15:59:41.34 (3)            | -52:23:09.5 (2)                      | 0.30 (3)                              | 1.1 (1)                 |
|                             | E        | 44                 | -69.61 (3)                               | 15:59:41.0 (2)             | -52:23:30 (1)                        | 0.40 (8)                              | 0.56 (9)                |
|                             |          |                    | -69.0 (2)                                | 15:59:40.81 (8)            | -52:23:28.2 (5)                      | 3.6 (4)                               | 0.34 (6)                |
|                             |          |                    | -68.76 (5)                               | 15:59:40.50 (8)            | -52:23:26.5 (6)                      | 0.4 (2)                               | 0.28 (9)                |
|                             |          |                    | -67.87 (3)                               | 15:59:40.58 (3)            | -52:23:25.4 (2)                      | 0.25 (8)                              | 0.4 (1)                 |
|                             | F        | 44                 | -70.0 (1)                                | 15:59:41.0 (1)             | -52:23:28 (1)                        | 1.3 (3)                               | 0.39 (5)                |
|                             |          |                    | -68.74 (3)                               | 15:59:40.96 (4)            | -52:23:29.3 (3)                      | 0.79 (8)                              | 1.13 (8)                |
|                             | G        | 36                 | -69.087 (6)                              | 15:59:41.510 (8)           | -52:23:36.61 (6)                     | 0.47 (1)                              | 1.75 (4)                |
|                             |          | 44                 | -69.38 (2)                               | 15:59:41.55 (3)            | -52:23:36.5 (2)                      | 0.44 (4)                              | 1.20 (8)                |
|                             | H        | 36                 | -66.2 (1)                                | 15:59:40.2 (1)             | -52:22:54.5 (9)                      | 3.6 (3)                               | 0.36 (3)                |
|                             | I        | 36                 | -76.19 (8)                               | 15:59:40.70 (3)            | -52:23:30.7 (3)                      | 0.6 (2)                               | 0.17 (4)                |
|                             |          |                    | -74.5 (2)                                | 15:59:40.6 (1)             | -52:23:30.1 (8)                      | 7.2 (4)                               | 0.41 (2)                |
|                             |          |                    | -74.033 (5)                              | 15:59:40.620 (7)           | -52:23:30.16 (6)                     | 0.57 (1)                              | 3.12 (5)                |
|                             |          |                    | -73.36 (2)                               | 15:59:40.69 (2)            | -52:23:30.6 (2)                      | 0.42 (6)                              | 0.65 (5)                |
|                             |          |                    | -72.652 (9)                              | 15:59:40.608 (8)           | -52:23:30.29 (6)                     | 0.52 (2)                              | 1.48 (5)                |



Table 3 – continued

| Source name                 | Location | Frequency<br>(GHz) | LSR<br>velocity<br>(km s <sup>-1</sup> ) | $\alpha_{2000}$<br>(h:m:s) | $\delta_{2000}$<br>(°:arcmin:arcsec) | Line<br>FWHM<br>(km s <sup>-1</sup> ) | Flux<br>density<br>(Jy) |
|-----------------------------|----------|--------------------|------------------------------------------|----------------------------|--------------------------------------|---------------------------------------|-------------------------|
| G329.47+0.50<br>(continued) | I        | 36                 | -69.76 (3)                               | 15:59:40.63 (4)            | -52:23:32.2 (3)                      | 0.78 (9)                              | 0.53 (5)                |
|                             |          |                    | -68.2 (4)                                | 15:59:40.68 (8)            | -52:23:34.2 (6)                      | 2.9 (7)                               | 0.18 (3)                |
|                             | J        | 36                 | -68.85 (1)                               | 15:59:38.09 (3)            | -52:23:44.1 (2)                      | 0.36 (3)                              | 1.10 (8)                |
| G331.13-0.24                | K        | 36                 | -72.33 (4)                               | 15:59:40.62 (3)            | -52:24:15.7 (3)                      | 2.9 (1)                               | 1.42 (4)                |
|                             | A        | 36                 | -91.202 (4)                              | 16:10:59.528 (2)           | -51:50:25.63 (2)                     | 0.464 (5)                             | 23.4 (3)                |
|                             |          |                    | -90.665 (3)                              | 16:10:59.524 (3)           | -51:50:25.68 (2)                     | 0.55 (1)                              | 26.0 (1)                |
|                             |          |                    | -90.126 (8)                              | 16:10:59.528 (7)           | -51:50:25.65 (4)                     | 0.35 (2)                              | 4.8 (3)                 |
|                             |          |                    | -89.53 (4)                               | 16:10:59.566 (5)           | -51:50:25.43 (3)                     | 0.97 (8)                              | 2.01 (8)                |
|                             |          |                    | -86.9 (1)                                | 16:10:59.52 (4)            | -51:50:24.8 (3)                      | 2.1 (3)                               | 0.60 (4)                |
|                             |          |                    | -83.73 (9)                               | 16:11:00.0 (1)             | -51:50:26.1 (7)                      | 2.7 (2)                               | 0.84 (4)                |
|                             |          | 44                 | -91.384 (3)                              | 16:10:59.518 (2)           | -51:50:25.90 (1)                     | 0.489 (4)                             | 80.3 (5)                |
|                             |          |                    | -90.913 (3)                              | 16:10:59.512 (1)           | -51:50:25.968 (9)                    | 0.482 (5)                             | 75.7 (5)                |
|                             |          |                    | -90.160 (6)                              | 16:10:59.531 (2)           | -51:50:25.80 (2)                     | 0.54 (2)                              | 15.5 (2)                |
|                             |          |                    | -89.452 (8)                              | 16:10:59.537 (2)           | -51:50:25.76 (1)                     | 0.66 (2)                              | 13.3 (2)                |
|                             |          |                    | -87.73 (6)                               | 16:10:59.7 (1)             | -51:50:25 (1)                        | 3.3 (1)                               | 5.1 (2)                 |
|                             |          |                    | -87.457 (8)                              | 16:10:59.544 (7)           | -51:50:25.70 (5)                     | 0.79 (3)                              | 7.3 (2)                 |
|                             |          |                    | -82.86 (5)                               | 16:10:59.76 (8)            | -51:50:25.5 (5)                      | 0.86 (9)                              | 1.2 (1)                 |
|                             | B        | 36                 | -88.58 (1)                               | 16:11:00.655 (5)           | -51:50:23.53 (3)                     | 0.53 (1)                              | 14.5 (4)                |
|                             |          |                    | -88.224 (3)                              | 16:11:00.696 (3)           | -51:50:23.69 (2)                     | 0.413 (4)                             | 24.9 (7)                |
|                             | C        | 36                 | -88.860 (4)                              | 16:11:00.693 (5)           | -51:50:23.98 (4)                     | 0.410 (6)                             | 23.8 (4)                |
|                             |          |                    | -88.457 (3)                              | 16:11:00.677 (2)           | -51:50:23.98 (1)                     | 0.471 (4)                             | 46.8 (3)                |
|                             |          |                    | -84.6 (2)                                | 16:11:00.28 (8)            | -51:50:25.2 (6)                      | 3.3 (4)                               | 0.32 (4)                |
|                             |          |                    | -84.36 (3)                               | 16:11:00.32 (2)            | -51:50:26.0 (1)                      | 0.40 (5)                              | 1.7 (2)                 |
|                             |          |                    | -83.95 (3)                               | 16:11:00.23 (3)            | -51:50:25.9 (2)                      | 0.41 (5)                              | 1.7 (1)                 |
|                             |          |                    | -84.617 (5)                              | 16:11:00.297 (8)           | -51:50:26.44 (5)                     | 0.37 (1)                              | 8.0 (1)                 |
|                             | D        | 44                 | -84.155 (8)                              | 16:11:00.266 (6)           | -51:50:26.05 (5)                     | 0.47 (2)                              | 6.0 (1)                 |
|                             |          |                    | -89.25 (6)                               | 16:10:59.27 (3)            | -51:50:12.3 (2)                      | 0.6 (2)                               | 0.4 (1)                 |
|                             |          |                    | -85.63 (3)                               | 16:10:59.23 (4)            | -51:50:11.7 (2)                      | 0.99 (8)                              | 1.4 (1)                 |
|                             |          |                    | -84.64 (2)                               | 16:10:59.41 (2)            | -51:50:11.3 (1)                      | 0.61 (5)                              | 1.28 (9)                |
|                             |          | 36                 | -87.16 (2)                               | 16:10:59.15 (3)            | -51:50:12.7 (2)                      | 0.91 (5)                              | 2.8 (1)                 |
|                             |          |                    | -86.11 (2)                               | 16:10:59.36 (2)            | -51:50:12.1 (1)                      | 0.52 (5)                              | 5.4 (2)                 |
|                             |          |                    | -85.60 (2)                               | 16:10:59.29 (2)            | -51:50:11.5 (2)                      | 0.45 (3)                              | 7.2 (3)                 |
|                             |          |                    | -84.706 (1)                              | 16:10:59.435 (3)           | -51:50:11.69 (2)                     | 0.528 (3)                             | 30.7 (1)                |
| G331.34-0.35                | A        | 36                 | -65.755 (6)                              | 16:12:26.451 (3)           | -51:46:20.47 (2)                     | 0.45 (1)                              | 8.55 (9)                |
|                             |          |                    | -65.45 (2)                               | 16:12:26.450 (1)           | -51:46:20.505 (9)                    | 0.22 (2)                              | 6.4 (8)                 |
|                             |          |                    | -65.287 (9)                              | 16:12:26.444 (2)           | -51:46:20.46 (1)                     | 0.198 (8)                             | 9.5 (9)                 |
|                             |          |                    | -65.857 (9)                              | 16:12:26.472 (7)           | -51:46:20.36 (4)                     | 0.54 (1)                              | 20.5 (3)                |
|                             |          | 44                 | -65.542 (2)                              | 16:12:26.467 (3)           | -51:46:20.31 (2)                     | 0.297 (6)                             | 21.4 (8)                |
| G331.44-0.19                | A        | 36                 | -91.51 (1)                               | 16:12:12.19 (5)            | -51:35:13.8 (4)                      | 0.35 (3)                              | 0.69 (5)                |
|                             |          | 44                 | -91.714 (2)                              | 16:12:12.242 (4)           | -51:35:14.01 (4)                     | 0.359 (5)                             | 10.2 (1)                |
|                             |          |                    | -90.15 (5)                               | 16:12:12.18 (4)            | -51:35:14.5 (3)                      | 1.7 (1)                               | 1.02 (6)                |
|                             | B        | 44                 | -91.721 (6)                              | 16:12:11.01 (1)            | -51:35:22.7 (1)                      | 0.38 (1)                              | 4.0 (1)                 |
|                             |          |                    | -90.10 (8)                               | 16:12:10.98 (6)            | -51:35:22.8 (5)                      | 1.6 (2)                               | 0.76 (6)                |
|                             | C        | 36                 | -88.7 (2)                                | 16:12:11.56 (8)            | -51:35:18.7 (6)                      | 2.3 (4)                               | 0.35 (2)                |
|                             |          |                    | -87.68 (2)                               | 16:12:11.36 (4)            | -51:35:19.2 (3)                      | 0.56 (5)                              | 1.02 (8)                |
|                             |          |                    | -86.66 (5)                               | 16:12:11.40 (8)            | -51:35:19.3 (6)                      | 0.9 (1)                               | 0.41 (5)                |
|                             |          |                    | -88.47 (2)                               | 16:12:11.40 (4)            | -51:35:19.3 (3)                      | 0.16 (6)                              | 0.7 (2)                 |
|                             |          | 44                 | -87.926 (4)                              | 16:12:11.35 (1)            | -51:35:18.9 (1)                      | 0.43 (1)                              | 7.2 (2)                 |

**Table 3** – *continued*

| Source name                 | Location | Frequency<br>(GHz) | LSR<br>velocity<br>(km s <sup>-1</sup> ) | $\alpha_{2000}$<br>(h:m:s) | $\delta_{2000}$<br>(°:arcmin:arcsec) | Line<br>FWHM<br>(km s <sup>-1</sup> ) | Flux<br>density<br>(Jy) |
|-----------------------------|----------|--------------------|------------------------------------------|----------------------------|--------------------------------------|---------------------------------------|-------------------------|
| G331.44-0.19<br>(continued) | C        | 44                 | -87.51 (8)                               | 16:12:11.39 (2)            | -51:35:19.3 (2)                      | 1.6 (1)                               | 2.1 (1)                 |
|                             |          |                    | -86.66 (2)                               | 16:12:11.44 (2)            | -51:35:19.2 (2)                      | 0.39 (6)                              | 1.3 (2)                 |
|                             | D        | 44                 | -87.964 (5)                              | 16:12:12.57 (2)            | -51:35:09.2 (2)                      | 0.19 (1)                              | 2.9 (2)                 |
|                             |          |                    | -86.5 (2)                                | 16:12:12.6 (1)             | -51:35:10 (1)                        | 3.2 (5)                               | 0.28 (4)                |
|                             | E        | 44                 | -87.83 (2)                               | 16:12:10.10 (3)            | -51:35:28.1 (3)                      | 0.31 (6)                              | 1.3 (2)                 |
|                             |          |                    | -87.48 (6)                               | 16:12:10.19 (5)            | -51:35:28.3 (4)                      | 1.5 (1)                               | 1.3 (1)                 |
| G332.30-0.09                | F        | 44                 | -88.277 (9)                              | 16:12:12.64 (1)            | -51:34:50.41 (9)                     | 0.45 (2)                              | 3.1 (1)                 |
|                             |          |                    | -51.18 (3)                               | 16:15:45.89 (2)            | -50:55:54.3 (2)                      | 0.80 (8)                              | 0.75 (5)                |
|                             | A        | 36                 | -49.71 (2)                               | 16:15:45.78 (5)            | -50:55:54.3 (4)                      | 1.58 (5)                              | 2.31 (6)                |
|                             |          |                    | -49.678 (1)                              | 16:15:45.777 (5)           | -50:55:54.53 (4)                     | 0.298 (3)                             | 9.95 (8)                |
|                             |          | 44                 | -50.89 (4)                               | 16:15:45.86 (2)            | -50:55:54.5 (1)                      | 0.52 (5)                              | 4.9 (3)                 |
|                             |          |                    | -50.587 (7)                              | 16:15:45.86 (1)            | -50:55:54.36 (6)                     | 0.30 (2)                              | 6.6 (8)                 |
|                             |          |                    | -49.93 (2)                               | 16:15:46.10 (8)            | -50:55:53.5 (4)                      | 2.34 (5)                              | 5.9 (4)                 |
|                             |          |                    | -49.882 (1)                              | 16:15:45.776 (6)           | -50:55:54.62 (3)                     | 0.286 (7)                             | 24 (1)                  |
|                             |          |                    | -49.62 (2)                               | 16:15:45.784 (8)           | -50:55:54.46 (4)                     | 0.58 (3)                              | 14.5 (7)                |
|                             |          |                    | -48.400 (4)                              | 16:15:45.63 (2)            | -50:55:55.43 (9)                     | 0.44 (1)                              | 6.1 (1)                 |
|                             |          |                    | -46.74 (3)                               | 16:15:45.57 (5)            | -50:55:51.9 (3)                      | 0.48 (8)                              | 0.66 (9)                |
|                             |          | B                  | -48.721 (7)                              | 16:15:44.79 (2)            | -50:55:52.9 (1)                      | 0.32 (2)                              | 1.57 (6)                |
|                             |          |                    | -48.16 (3)                               | 16:15:44.82 (6)            | -50:55:53.6 (4)                      | 0.37 (8)                              | 0.41 (6)                |
|                             | C        | 44                 | -48.946 (3)                              | 16:15:44.80 (1)            | -50:55:53.05 (8)                     | 0.285 (7)                             | 5.7 (1)                 |
|                             |          |                    | -46.153 (8)                              | 16:15:44.20 (2)            | -50:55:56.2 (1)                      | 0.70 (2)                              | 3.14 (8)                |
| G332.60-0.17                | A        | 36                 | -45.901 (5)                              | 16:17:29.60 (2)            | -50:46:09.7 (2)                      | 0.29 (2)                              | 2.2 (2)                 |
|                             |          |                    | -45.812 (6)                              | 16:17:29.30 (3)            | -50:46:10.9 (2)                      | 0.74 (2)                              | 3.3 (2)                 |
|                             |          | 44                 | -46.55 (2)                               | 16:17:29.31 (8)            | -50:46:15 (1)                        | 0.20 (4)                              | 0.7 (1)                 |
|                             |          |                    | -46.13 (3)                               | 16:17:29.25 (4)            | -50:46:11.0 (4)                      | 0.36 (3)                              | 5.6 (6)                 |
|                             |          |                    | -45.82 (1)                               | 16:17:29.23 (2)            | -50:46:10.7 (2)                      | 0.37 (2)                              | 12 (1)                  |
|                             |          |                    | -45.51 (9)                               | 16:17:29.26 (5)            | -50:46:11.0 (4)                      | 0.8 (1)                               | 2.9 (4)                 |
|                             | B        | 36                 | -49.3 (3)                                | 16:17:29.6 (1)             | -50:46:04 (1)                        | 5.1 (6)                               | 0.19 (2)                |
|                             |          |                    | -46.82 (4)                               | 16:17:29.57 (6)            | -50:46:01.7 (4)                      | 1.0 (1)                               | 0.39 (4)                |
|                             |          | 44                 | -46.90 (9)                               | 16:17:29.64 (8)            | -50:46:01.9 (6)                      | 2.0 (2)                               | 0.36 (3)                |
|                             |          |                    | -48.67 (8)                               | 16:21:19.1 (2)             | -50:54:11.7 (7)                      | 1.9 (2)                               | 0.24 (3)                |
| G332.94-0.69                | A        | 36                 | -48.48 (1)                               | 16:21:19.32 (6)            | -50:54:12.1 (4)                      | 0.23 (3)                              | 0.53 (6)                |
|                             |          |                    | -50.58 (1)                               | 16:21:19.16 (2)            | -50:54:13.7 (1)                      | 0.21 (3)                              | 1.0 (1)                 |
|                             |          | 44                 | -50.18 (6)                               | 16:21:19.31 (8)            | -50:54:13.6 (5)                      | 1.3 (1)                               | 0.86 (5)                |
|                             |          |                    | -49.27 (1)                               | 16:21:19.37 (2)            | -50:54:11.9 (2)                      | 0.38 (3)                              | 1.9 (1)                 |
|                             |          |                    | -48.603 (9)                              | 16:21:19.32 (3)            | -50:54:12.5 (2)                      | 0.79 (3)                              | 3.60 (5)                |
|                             |          |                    | -47.29 (2)                               | 16:21:19.25 (2)            | -50:54:13.3 (2)                      | 0.79 (6)                              | 0.87 (5)                |
|                             |          | B                  | -48.18 (5)                               | 16:21:19.27 (6)            | -50:54:06.2 (4)                      | 1.1 (1)                               | 0.25 (2)                |
|                             |          |                    | -48.46 (4)                               | 16:21:19.35 (3)            | -50:54:05.8 (2)                      | 0.88 (8)                              | 1.13 (5)                |
|                             | C        | 36                 | -47.63 (3)                               | 16:21:19.32 (5)            | -50:54:05.5 (4)                      | 0.62 (6)                              | 0.96 (8)                |
|                             |          |                    | -49.39 (2)                               | 16:21:21.36 (5)            | -50:54:18.8 (3)                      | 0.75 (6)                              | 0.56 (4)                |
|                             |          | 44                 | -49.49 (2)                               | 16:21:21.45 (4)            | -50:54:18.6 (3)                      | 0.53 (5)                              | 1.37 (8)                |
|                             |          |                    | -58.121 (6)                              | 16:21:22.40 (4)            | -50:52:53.8 (2)                      | 0.28 (2)                              | 1.8 (2)                 |
|                             |          |                    | -58.03 (1)                               | 16:21:22.44 (2)            | -50:52:54.1 (1)                      | 0.65 (3)                              | 1.5 (2)                 |
|                             |          |                    | -52.98 (8)                               | 16:21:22.14 (8)            | -50:52:54.4 (4)                      | 4.3 (2)                               | 0.38 (1)                |
| G332.96-0.68                | A        | 36                 | -49.53 (4)                               | 16:21:22.6 (2)             | -50:52:49 (1)                        | 0.4 (1)                               | 0.20 (5)                |
|                             |          |                    | -48.42 (2)                               | 16:21:22.50 (8)            | -50:52:49.4 (5)                      | 0.98 (6)                              | 0.65 (3)                |
|                             |          |                    | -47.20 (2)                               | 16:21:22.72 (3)            | -50:52:56.7 (2)                      | 0.34 (4)                              | 0.64 (5)                |
|                             |          |                    |                                          |                            |                                      |                                       |                         |

Table 3 – continued

| Source name                 | Location | Frequency (GHz) | LSR velocity (km s <sup>-1</sup> ) | $\alpha_{2000}$ (h:m:s) | $\delta_{2000}$ (°:arcmin:arcsec) | Line FWHM (km s <sup>-1</sup> ) | Flux density (Jy) |
|-----------------------------|----------|-----------------|------------------------------------|-------------------------|-----------------------------------|---------------------------------|-------------------|
| G332.96-0.68<br>(continued) | A        | 36              | -46.66 (4)                         | 16:21:22.73 (6)         | -50:52:56.0 (4)                   | 0.5 (1)                         | 0.35 (4)          |
|                             |          | 44              | -50.928 (8)                        | 16:21:22.76 (1)         | -50:52:55.54 (9)                  | 0.61 (2)                        | 2.57 (8)          |
|                             |          |                 | -49.5 (5)                          | 16:21:23.0 (1)          | -50:52:55.6 (9)                   | 2.7 (9)                         | 0.24 (3)          |
|                             |          |                 | -48.629 (4)                        | 16:21:22.81 (1)         | -50:52:56.2 (1)                   | 0.32 (1)                        | 4.1 (1)           |
|                             |          |                 | -48.12 (1)                         | 16:21:22.66 (2)         | -50:52:57.3 (2)                   | 0.27 (3)                        | 1.2 (1)           |
|                             |          |                 | -47.43 (1)                         | 16:21:22.76 (2)         | -50:52:56.6 (2)                   | 0.38 (1)                        | 8.7 (9)           |
|                             |          |                 | -46.95 (2)                         | 16:21:22.768 (3)        | -50:52:56.13 (2)                  | 0.61 (8)                        | 13.1 (3)          |
|                             |          |                 | -46.565 (7)                        | 16:21:22.758 (8)        | -50:52:56.26 (6)                  | 0.35 (2)                        | 10 (2)            |
|                             | B        | 36              | -48.7 (1)                          | 16:21:22.8 (1)          | -50:53:06.0 (8)                   | 2.7 (3)                         | 0.19 (3)          |
|                             |          |                 | -48.63 (1)                         | 16:21:22.83 (3)         | -50:53:05.1 (2)                   | 0.47 (3)                        | 0.81 (4)          |
| G333.03-0.06                | A        | 36              | -40.757 (4)                        | 16:18:56.73 (1)         | -50:23:54.80 (9)                  | 0.324 (9)                       | 1.74 (4)          |
|                             |          |                 | -39.892 (8)                        | 16:18:56.70 (1)         | -50:23:54.73 (9)                  | 0.59 (2)                        | 1.17 (3)          |
|                             |          | 44              | -42.16 (2)                         | 16:18:56.64 (4)         | -50:23:53.7 (3)                   | 0.55 (5)                        | 0.76 (8)          |
|                             |          |                 | -40.970 (2)                        | 16:18:56.761 (4)        | -50:23:55.02 (3)                  | 0.352 (6)                       | 8.44 (9)          |
|                             |          |                 | -40.607 (7)                        | 16:18:56.743 (7)        | -50:23:54.84 (5)                  | 0.20 (2)                        | 2.0 (1)           |
|                             |          |                 | -40.039 (5)                        | 16:18:56.718 (8)        | -50:23:54.83 (6)                  | 0.73 (1)                        | 5.28 (6)          |
| G333.13-0.44                | A        | 36              | -50.31 (2)                         | 16:21:02.59 (3)         | -50:36:01.0 (2)                   | 0.98 (5)                        | 1.04 (4)          |
|                             |          |                 | -49.881 (1)                        | 16:21:02.920 (1)        | -50:35:59.748 (5)                 | 0.192 (2)                       | 50.7 (7)          |
|                             |          |                 | -49.821 (2)                        | 16:21:02.902 (5)        | -50:35:59.68 (3)                  | 0.478 (5)                       | 37.4 (7)          |
|                             |          |                 | -49.344 (2)                        | 16:21:02.892 (6)        | -50:35:59.63 (4)                  | 0.249 (5)                       | 14.8 (2)          |
|                             |          |                 | -49.02 (6)                         | 16:21:02.6 (2)          | -50:36:00.7 (6)                   | 3.9 (1)                         | 0.79 (2)          |
|                             |          |                 | -48.976 (2)                        | 16:21:02.88 (3)         | -50:35:59.5 (2)                   | 0.342 (7)                       | 17.4 (1)          |
|                             |          |                 | -48.491 (7)                        | 16:21:02.70 (3)         | -50:35:55.0 (2)                   | 0.41 (2)                        | 9.0 (3)           |
|                             |          |                 | -47.99 (1)                         | 16:21:02.2 (1)          | -50:35:52.4 (9)                   | 0.58 (3)                        | 7.4 (1)           |
|                             |          |                 | -47.376 (9)                        | 16:21:02.65 (1)         | -50:35:54.88 (9)                  | 0.26 (1)                        | 10.9 (4)          |
|                             |          |                 | -47.181 (4)                        | 16:21:02.63 (3)         | -50:35:54.6 (2)                   | 0.196 (4)                       | 16.7 (8)          |
|                             |          |                 | -46.393 (6)                        | 16:21:02.229 (7)        | -50:35:53.46 (5)                  | 0.79 (2)                        | 7.22 (6)          |
|                             |          |                 | -45.54 (2)                         | 16:21:02.27 (2)         | -50:35:53.6 (1)                   | 0.65 (3)                        | 2.55 (8)          |
|                             |          | 44              | -51.19 (8)                         | 16:21:02.78 (2)         | -50:36:02.1 (2)                   | 0.5 (2)                         | 1.0 (3)           |
|                             |          |                 | -50.054 (1)                        | 16:21:02.884 (8)        | -50:35:59.92 (6)                  | 0.286 (2)                       | 66.2 (9)          |
|                             |          |                 | -49.912 (5)                        | 16:21:02.88 (1)         | -50:35:59.95 (8)                  | 0.636 (4)                       | 38.7 (5)          |
|                             |          |                 | -49.094 (4)                        | 16:21:02.64 (1)         | -50:35:55.48 (8)                  | 0.454 (8)                       | 34.6 (4)          |
|                             |          |                 | -48.368 (3)                        | 16:21:02.13 (2)         | -50:35:50.7 (2)                   | 0.70 (1)                        | 47.4 (3)          |
|                             |          |                 | -47.487 (4)                        | 16:21:02.679 (4)        | -50:35:54.78 (3)                  | 0.46 (1)                        | 36.4 (4)          |
|                             |          |                 | -46.76 (2)                         | 16:21:02.24 (1)         | -50:35:53.46 (8)                  | 0.59 (5)                        | 24.5 (7)          |
|                             |          |                 | -46.23 (5)                         | 16:21:02.25 (2)         | -50:35:53.5 (1)                   | 0.5 (1)                         | 7 (2)             |
|                             |          |                 | -45.69 (5)                         | 16:21:02.227 (9)        | -50:35:53.44 (8)                  | 0.60 (8)                        | 9.0 (6)           |
|                             | B        | 44              | -53.13 (4)                         | 16:20:59.58 (4)         | -50:35:52.8 (4)                   | 0.40 (8)                        | 2.5 (2)           |
|                             |          |                 | -52.79 (6)                         | 16:20:59.55 (5)         | -50:35:51.5 (4)                   | 2.5 (2)                         | 1.8 (1)           |
|                             |          |                 | -52.73 (2)                         | 16:20:59.50 (4)         | -50:35:50.9 (3)                   | 0.35 (3)                        | 5.4 (3)           |
|                             |          |                 | -50.808 (4)                        | 16:20:59.40 (1)         | -50:35:48.7 (1)                   | 0.336 (9)                       | 8.8 (2)           |
|                             | C        | 44              | -50.028 (2)                        | 16:21:02.014 (3)        | -50:36:20.40 (3)                  | 0.345 (4)                       | 21.5 (2)          |
|                             | D        | 44              | -51.552 (1)                        | 16:21:03.101 (4)        | -50:35:38.16 (3)                  | 0.259 (3)                       | 11.0 (1)          |
|                             | DF       | 36              | -51.346 (2)                        | 16:21:03.106 (3)        | -50:35:38.26 (2)                  | 0.280 (3)                       | 6.58 (6)          |
|                             |          |                 | -50.27 (8)                         | 16:21:04.1 (1)          | -50:35:38 (1)                     | 1.9 (1)                         | 0.38 (2)          |
|                             |          |                 | -50.070 (1)                        | 16:21:03.787 (4)        | -50:35:39.73 (3)                  | 0.424 (3)                       | 21.99 (6)         |
|                             |          |                 | -49.673 (3)                        | 16:21:03.82 (2)         | -50:35:39.5 (1)                   | 0.263 (6)                       | 5.4 (1)           |
|                             |          |                 | -48.556 (6)                        | 16:21:03.53 (2)         | -50:35:42.2 (1)                   | 0.29 (1)                        | 1.82 (6)          |

Table 3 – *continued*

| Source name                 | Location | Frequency<br>(GHz) | LSR<br>velocity<br>(km s <sup>-1</sup> ) | $\alpha_{2000}$<br>(h:m:s) | $\delta_{2000}$<br>(°:arcmin:arcsec) | Line<br>FWHM<br>(km s <sup>-1</sup> ) | Flux<br>density<br>(Jy) |
|-----------------------------|----------|--------------------|------------------------------------------|----------------------------|--------------------------------------|---------------------------------------|-------------------------|
| G333.13-0.44<br>(continued) | E        | 36                 | -50.74 (5)                               | 16:21:03.27 (5)            | -50:35:47.7 (3)                      | 2.1 (1)                               | 0.47 (2)                |
|                             |          | 44                 | -52.52 (8)                               | 16:21:03.15 (8)            | -50:35:47.4 (5)                      | 1.8 (2)                               | 0.52 (3)                |
|                             | F        | 44                 | -51.00 (2)                               | 16:21:03.17 (3)            | -50:35:47.5 (2)                      | 0.65 (5)                              | 1.5 (1)                 |
|                             |          | 44                 | -50.294 (2)                              | 16:21:03.803 (3)           | -50:35:39.74 (2)                     | 0.533 (4)                             | 31.1 (1)                |
| G333.13-0.56                | G        | 44                 | -49.787 (2)                              | 16:21:03.827 (7)           | -50:35:39.60 (5)                     | 0.392 (4)                             | 21.4 (2)                |
|                             |          | 44                 | -55.660 (7)                              | 16:21:01.94 (1)            | -50:35:17.3 (1)                      | 0.34 (2)                              | 4.1 (2)                 |
|                             | H        | 36                 | -51.92 (3)                               | 16:21:04.90 (8)            | -50:35:41.3 (5)                      | 0.53 (8)                              | 0.35 (4)                |
|                             |          | 36                 | -59.903 (8)                              | 16:21:34.37 (3)            | -50:41:06.4 (2)                      | 0.25 (3)                              | 1.2 (1)                 |
| G333.13-0.56                | A        | 36                 | -59.5 (1)                                | 16:21:34.3 (1)             | -50:41:06.0 (9)                      | 0.7 (5)                               | 0.23 (5)                |
|                             |          | 36                 | -58.776 (7)                              | 16:21:34.22 (2)            | -50:41:06.0 (2)                      | 0.36 (2)                              | 1.91 (6)                |
|                             | B        | 44                 | -60.12 (2)                               | 16:21:34.41 (1)            | -50:41:06.3 (1)                      | 0.42 (3)                              | 2.9 (1)                 |
|                             |          | 44                 | -59.59 (2)                               | 16:21:34.35 (1)            | -50:41:06.00 (9)                     | 0.47 (8)                              | 3.1 (1)                 |
| G333.13-0.56                | B        | 36                 | -59.28 (2)                               | 16:21:34.35 (3)            | -50:41:05.9 (3)                      | 0.16 (6)                              | 0.9 (4)                 |
|                             |          | 36                 | -58.99 (1)                               | 16:21:34.32 (2)            | -50:41:05.7 (2)                      | 0.40 (2)                              | 3.8 (1)                 |
|                             | C        | 36                 | -60.166 (7)                              | 16:21:35.449 (7)           | -50:40:49.08 (5)                     | 0.59 (2)                              | 1.75 (5)                |
|                             |          | 36                 | -58.775 (4)                              | 16:21:35.60 (1)            | -50:40:47.07 (9)                     | 0.26 (1)                              | 2.00 (8)                |
| G333.13-0.56                | C        | 36                 | -58.152 (8)                              | 16:21:35.36 (8)            | -50:40:42.6 (5)                      | 0.31 (2)                              | 1.60 (8)                |
|                             |          | 36                 | -57.709 (3)                              | 16:21:35.76 (2)            | -50:40:46.3 (2)                      | 0.331 (6)                             | 5.57 (8)                |
|                             | D        | 36                 | -57.277 (8)                              | 16:21:35.5 (1)             | -50:40:44 (1)                        | 0.33 (2)                              | 1.16 (5)                |
|                             |          | 36                 | -56.71 (6)                               | 16:21:36.3 (1)             | -50:40:45 (1)                        | 3.54 (8)                              | 1.79 (5)                |
| G333.13-0.56                | E        | 36                 | -56.679 (8)                              | 16:21:35.6 (2)             | -50:40:44 (1)                        | 1.15 (1)                              | 2.31 (3)                |
|                             |          | 36                 | -56.3 (1)                                | 16:21:35.79 (2)            | -50:40:46.4 (2)                      | 0.6 (1)                               | 2.2 (5)                 |
|                             | F        | 36                 | -56.158 (7)                              | 16:21:35.80 (2)            | -50:40:46.5 (2)                      | 0.25 (3)                              | 4 (1)                   |
|                             |          | 36                 | -55.860 (3)                              | 16:21:36.47 (3)            | -50:40:47.4 (2)                      | 0.15 (1)                              | 3.0 (3)                 |
| G333.13-0.56                | G        | 36                 | -55.316 (9)                              | 16:21:36.47 (4)            | -50:40:45.5 (3)                      | 0.85 (4)                              | 3.95 (8)                |
|                             |          | 36                 | -54.50 (2)                               | 16:21:36.43 (6)            | -50:40:45.3 (4)                      | 0.57 (4)                              | 3.4 (2)                 |
|                             | H        | 36                 | -54.234 (2)                              | 16:21:36.05 (2)            | -50:40:47.6 (2)                      | 0.257 (8)                             | 6.6 (3)                 |
|                             |          | 36                 | -62.11 (3)                               | 16:21:36.15 (5)            | -50:40:49.0 (4)                      | 0.53 (8)                              | 0.78 (9)                |
| G333.13-0.56                | I        | 36                 | -59.98 (3)                               | 16:21:35.70 (5)            | -50:40:46.5 (4)                      | 0.43 (6)                              | 0.8 (1)                 |
|                             |          | 36                 | -59.04 (2)                               | 16:21:35.64 (8)            | -50:40:48.0 (7)                      | 0.62 (6)                              | 1.23 (9)                |
|                             | J        | 36                 | -57.78 (3)                               | 16:21:35.78 (3)            | -50:40:46.9 (2)                      | 0.87 (8)                              | 2.44 (8)                |
|                             |          | 36                 | -57.31 (1)                               | 16:21:35.96 (4)            | -50:40:48.0 (3)                      | 0.24 (5)                              | 1.3 (3)                 |
| G333.13-0.56                | K        | 36                 | -56.91 (1)                               | 16:21:36.42 (3)            | -50:40:47.5 (3)                      | 0.25 (4)                              | 1.4 (2)                 |
|                             |          | 36                 | -56.080 (1)                              | 16:21:36.498 (3)           | -50:40:48.16 (2)                     | 0.188 (3)                             | 21.1 (3)                |
|                             | L        | 36                 | -55.71 (3)                               | 16:21:36.50 (2)            | -50:40:47.5 (2)                      | 1.4 (1)                               | 5.0 (4)                 |
|                             |          | 36                 | -55.68 (1)                               | 16:21:36.44 (2)            | -50:40:47.2 (1)                      | 0.23 (3)                              | 3.7 (4)                 |
| G333.13-0.56                | M        | 36                 | -55.422 (8)                              | 16:21:36.40 (4)            | -50:40:47.1 (3)                      | 0.22 (2)                              | 4.6 (3)                 |
|                             |          | 36                 | -54.61 (2)                               | 16:21:36.040 (8)           | -50:40:47.90 (6)                     | 0.45 (3)                              | 19 (1)                  |
|                             | N        | 36                 | -54.379 (2)                              | 16:21:36.039 (4)           | -50:40:47.90 (3)                     | 0.270 (7)                             | 29 (2)                  |
|                             |          | 36                 | -60.4 (2)                                | 16:21:37.67 (9)            | -50:41:15.7 (7)                      | 5.0 (4)                               | 0.38 (4)                |
| G333.13-0.56                | O        | 36                 | -59.39 (2)                               | 16:21:37.92 (3)            | -50:41:17.9 (2)                      | 0.99 (8)                              | 1.47 (8)                |
|                             |          | 36                 | -58.732 (8)                              | 16:21:37.95 (2)            | -50:41:17.7 (2)                      | 0.17 (2)                              | 1.5 (2)                 |
|                             | P        | 36                 | -58.348 (4)                              | 16:21:37.961 (9)           | -50:41:15.13 (8)                     | 0.52 (1)                              | 7.64 (8)                |
|                             |          | 36                 | -53.35 (2)                               | 16:21:37.87 (8)            | -50:41:17.9 (6)                      | 0.88 (6)                              | 1.01 (6)                |
| G333.13-0.56                | Q        | 36                 | -49.88 (6)                               | 16:21:37.82 (6)            | -50:41:18.9 (5)                      | 2.1 (1)                               | 0.59 (4)                |
|                             |          | 36                 | -59.888 (8)                              | 16:21:38.02 (3)            | -50:41:18.2 (2)                      | 0.39 (2)                              | 3.8 (2)                 |
|                             | R        | 36                 | -58.998 (5)                              | 16:21:37.985 (9)           | -50:41:18.32 (8)                     | 0.15 (1)                              | 4.4 (3)                 |
|                             |          | 36                 | -58.442 (5)                              | 16:21:37.98 (1)            | -50:41:15.07 (9)                     | 0.61 (1)                              | 11.8 (4)                |

Table 3 – continued

| Source name                 | Location | Frequency<br>(GHz) | LSR<br>velocity<br>(km s <sup>-1</sup> ) | $\alpha_{2000}$<br>(h:m:s) | $\delta_{2000}$<br>(°:arcmin:arcsec) | Line<br>FWHM<br>(km s <sup>-1</sup> ) | Flux<br>density<br>(Jy) |
|-----------------------------|----------|--------------------|------------------------------------------|----------------------------|--------------------------------------|---------------------------------------|-------------------------|
| G333.13-0.56<br>(continued) | C        | 44                 | -58.361 (7)                              | 16:21:37.98 (4)            | -50:41:16.0 (3)                      | 0.17 (2)                              | 3.3 (4)                 |
|                             | D        | 44                 | -59.56 (1)                               | 16:21:35.76 (2)            | -50:40:54.6 (2)                      | 0.35 (2)                              | 4.4 (1)                 |
|                             |          |                    | -59.13 (1)                               | 16:21:35.756 (6)           | -50:40:54.90 (5)                     | 0.35 (2)                              | 13.4 (7)                |
|                             |          |                    | -58.82 (3)                               | 16:21:35.80 (2)            | -50:40:54.7 (1)                      | 0.36 (3)                              | 7.1 (7)                 |
|                             |          |                    | -55.252 (7)                              | 16:21:35.76 (4)            | -50:40:35.0 (3)                      | 0.20 (2)                              | 2.1 (1)                 |
|                             | E        | 44                 | -55.252 (7)                              | 16:21:35.76 (4)            | -50:40:35.0 (3)                      | 0.20 (2)                              | 2.1 (1)                 |
| G333.16-0.10                | F        | 36                 | -62.40 (2)                               | 16:21:34.94 (2)            | -50:40:55.0 (1)                      | 0.50 (5)                              | 0.59 (5)                |
|                             |          |                    | -61.6 (2)                                | 16:21:34.8 (1)             | -50:40:56.8 (7)                      | 2.1 (3)                               | 0.19 (2)                |
|                             |          |                    | -92.53 (3)                               | 16:19:42.16 (9)            | -50:20:00.2 (6)                      | 0.72 (8)                              | 0.29 (3)                |
|                             | A        | 44                 | -92.94 (1)                               | 16:19:42.15 (2)            | -50:19:59.7 (2)                      | 0.18 (2)                              | 1.0 (1)                 |
|                             |          |                    | -92.436 (9)                              | 16:19:42.21 (2)            | -50:20:00.0 (2)                      | 0.36 (2)                              | 1.58 (8)                |
|                             |          |                    | -91.94 (2)                               | 16:19:42.76 (6)            | -50:19:55.7 (4)                      | 0.22 (4)                              | 0.30 (4)                |
|                             |          | 36                 | -91.267 (4)                              | 16:19:42.71 (2)            | -50:19:55.1 (1)                      | 0.55 (1)                              | 1.86 (3)                |
|                             |          |                    | -90.52 (1)                               | 16:19:42.82 (4)            | -50:19:54.6 (3)                      | 0.29 (3)                              | 0.39 (4)                |
|                             |          |                    | -91.511 (3)                              | 16:19:42.691 (4)           | -50:19:55.22 (3)                     | 0.650 (7)                             | 6.90 (6)                |
|                             |          |                    | -90.69 (1)                               | 16:19:42.70 (2)            | -50:19:54.9 (2)                      | 0.28 (2)                              | 1.27 (9)                |
| G333.18-0.09                | A        | 36                 | -87.42 (2)                               | 16:19:45.53 (5)            | -50:18:32.6 (4)                      | 0.46 (4)                              | 0.54 (4)                |
|                             |          |                    | -86.63 (1)                               | 16:19:45.62 (3)            | -50:18:34.1 (2)                      | 0.25 (3)                              | 0.51 (5)                |
|                             |          |                    | -87.71 (3)                               | 16:19:45.56 (4)            | -50:18:32.5 (2)                      | 0.62 (9)                              | 1.0 (1)                 |
|                             |          | 44                 | -86.841 (4)                              | 16:19:45.61 (1)            | -50:18:33.56 (9)                     | 0.32 (1)                              | 4.6 (2)                 |
|                             |          |                    | -86.3 (2)                                | 16:19:46.06 (4)            | -50:18:31.8 (3)                      | 1.8 (4)                               | 0.58 (6)                |
|                             |          |                    | -85.890 (6)                              | 16:19:45.97 (3)            | -50:18:32.0 (2)                      | 0.23 (2)                              | 2.1 (1)                 |
|                             | B        | 36                 | -86.20 (1)                               | 16:19:46.48 (3)            | -50:18:37.1 (2)                      | 0.61 (2)                              | 1.10 (3)                |
|                             |          | 44                 | -86.336 (8)                              | 16:19:46.49 (3)            | -50:18:37.2 (2)                      | 0.69 (2)                              | 3.08 (8)                |
| G333.23-0.06                | A        | 36                 | -106.4 (1)                               | 16:19:49.40 (5)            | -50:15:13.4 (4)                      | 0.6 (2)                               | 0.5 (2)                 |
|                             |          |                    | -97.76 (4)                               | 16:19:49.436 (6)           | -50:15:13.67 (4)                     | 0.86 (9)                              | 2.1 (2)                 |
|                             |          |                    | -96.07 (3)                               | 16:19:49.434 (9)           | -50:15:13.57 (8)                     | 1.6 (1)                               | 5.5 (3)                 |
|                             |          |                    | -95.798 (3)                              | 16:19:49.439 (3)           | -50:15:13.74 (2)                     | 0.474 (8)                             | 21.6 (4)                |
|                             |          |                    | -93.88 (6)                               | 16:19:49.41 (1)            | -50:15:13.8 (1)                      | 1.2 (1)                               | 1.5 (1)                 |
|                             |          |                    | -88.7 (3)                                | 16:19:49.42 (3)            | -50:15:13.0 (3)                      | 3.5 (3)                               | 1.2 (2)                 |
|                             |          |                    | -88.09 (4)                               | 16:19:49.510 (9)           | -50:15:13.37 (8)                     | 0.81 (4)                              | 10.2 (9)                |
|                             |          |                    | -87.900 (3)                              | 16:19:49.529 (3)           | -50:15:13.34 (2)                     | 0.336 (9)                             | 24.5 (9)                |
|                             |          |                    | -87.089 (6)                              | 16:19:49.456 (2)           | -50:15:14.20 (1)                     | 1.02 (1)                              | 51.8 (3)                |
|                             |          | 44                 | -91.0 (2)                                | 16:19:49.44 (3)            | -50:15:13.8 (2)                      | 1.8 (2)                               | 1.3 (2)                 |
|                             |          |                    | -89.89 (3)                               | 16:19:49.45 (2)            | -50:15:14.4 (1)                      | 0.9 (1)                               | 4.5 (2)                 |
|                             |          |                    | -88.93 (2)                               | 16:19:49.48 (1)            | -50:15:14.07 (9)                     | 0.68 (6)                              | 6.7 (3)                 |
|                             |          |                    | -87.532 (8)                              | 16:19:49.526 (1)           | -50:15:13.821 (9)                    | 1.18 (1)                              | 132 (2)                 |
|                             |          |                    | -87.410 (2)                              | 16:19:49.468 (1)           | -50:15:14.331 (5)                    | 0.512 (6)                             | 152 (3)                 |
|                             |          |                    | -87.092 (1)                              | 16:19:49.471 (1)           | -50:15:14.354 (5)                    | 0.249 (3)                             | 90 (2)                  |
|                             |          |                    | -86.741 (1)                              | 16:19:49.487 (2)           | -50:15:14.34 (1)                     | 0.641 (3)                             | 69 (2)                  |
|                             | B        | 36                 | -88.73 (1)                               | 16:19:51.36 (3)            | -50:15:18.6 (2)                      | 0.56 (4)                              | 1.14 (6)                |
|                             |          |                    | -86.02 (3)                               | 16:19:51.67 (1)            | -50:15:18.01 (8)                     | 0.68 (8)                              | 3 (1)                   |
|                             |          |                    | -85.38 (8)                               | 16:19:51.60 (5)            | -50:15:16.9 (4)                      | 1.20 (6)                              | 6.4 (6)                 |
|                             |          |                    | -85.316 (2)                              | 16:19:51.55 (2)            | -50:15:16.9 (2)                      | 0.297 (6)                             | 11.4 (3)                |
|                             |          | 44                 | -91.58 (2)                               | 16:19:51.78 (2)            | -50:15:15.4 (1)                      | 0.62 (5)                              | 1.4 (1)                 |
|                             |          |                    | -89.015 (5)                              | 16:19:51.32 (1)            | -50:15:19.75 (8)                     | 0.47 (1)                              | 5.6 (1)                 |
|                             |          |                    | -88.160 (4)                              | 16:19:51.40 (1)            | -50:15:17.88 (8)                     | 0.264 (9)                             | 5.2 (2)                 |
|                             |          |                    | -86.140 (2)                              | 16:19:52.135 (7)           | -50:15:17.98 (4)                     | 0.334 (5)                             | 11.5 (1)                |
|                             |          |                    | -85.564 (2)                              | 16:19:51.53 (1)            | -50:15:16.45 (8)                     | 0.317 (4)                             | 20.5 (2)                |

**Table 3** – *continued*

| Source name                 | Location | Frequency<br>(GHz) | LSR<br>velocity<br>(km s <sup>-1</sup> ) | $\alpha_{2000}$<br>(h:m:s) | $\delta_{2000}$<br>(°:arcmin:arcsec) | Line<br>FWHM<br>(km s <sup>-1</sup> ) | Flux<br>density<br>(Jy) |
|-----------------------------|----------|--------------------|------------------------------------------|----------------------------|--------------------------------------|---------------------------------------|-------------------------|
| G333.23-0.06<br>(continued) | B        | 44                 | -84.986 (5)                              | 16:19:51.54 (2)            | -50:15:16.2 (1)                      | 0.51 (1)                              | 8.1 (1)                 |
|                             | C        | 44                 | -88.240 (8)                              | 16:19:51.29 (5)            | -50:15:12.6 (3)                      | 0.25 (2)                              | 2.2 (1)                 |
|                             |          |                    | -87.309 (1)                              | 16:19:51.536 (4)           | -50:15:10.75 (3)                     | 0.189 (2)                             | 20.2 (2)                |
|                             |          |                    | -85.557 (3)                              | 16:19:51.32 (6)            | -50:15:11.2 (4)                      | 0.389 (7)                             | 9.0 (1)                 |
|                             |          |                    | -85.31 (6)                               | 16:19:51.47 (8)            | -50:15:14.8 (7)                      | 2.0 (1)                               | 0.98 (9)                |
|                             | D        | 44                 | -89.2 (1)                                | 16:19:50.84 (8)            | -50:15:08.1 (5)                      | 3.8 (3)                               | 0.65 (4)                |
|                             |          |                    | -88.54 (1)                               | 16:19:50.85 (3)            | -50:15:07.6 (2)                      | 0.25 (3)                              | 1.5 (1)                 |
|                             | E        | 44                 | -90.44 (1)                               | 16:19:49.60 (2)            | -50:15:05.3 (1)                      | 0.61 (3)                              | 2.6 (1)                 |
|                             | F        | 36                 | -89.3 (1)                                | 16:19:51.05 (6)            | -50:15:06.4 (5)                      | 1.4 (2)                               | 0.74 (4)                |
|                             |          |                    | -88.45 (2)                               | 16:19:51.16 (6)            | -50:15:05.4 (4)                      | 0.55 (8)                              | 0.9 (1)                 |
| G333.32+0.11                | A        | 44                 | -49.62 (2)                               | 16:19:28.88 (9)            | -50:04:39.2 (8)                      | 0.68 (6)                              | 1.6 (3)                 |
|                             |          |                    | -49.582 (7)                              | 16:19:28.84 (2)            | -50:04:39.4 (1)                      | 0.24 (3)                              | 2.0 (3)                 |
|                             |          |                    | -44.47 (2)                               | 16:19:28.942 (9)           | -50:04:41.20 (8)                     | 0.71 (3)                              | 5.42 (9)                |
|                             |          |                    | -44.02 (1)                               | 16:19:28.92 (3)            | -50:04:41.5 (2)                      | 0.35 (3)                              | 2.4 (3)                 |
|                             | B        | 36                 | -50.71 (9)                               | 16:19:28.14 (5)            | -50:04:42.6 (4)                      | 2.0 (2)                               | 0.46 (2)                |
|                             |          |                    | -48.2 (1)                                | 16:19:28.09 (4)            | -50:04:39.5 (3)                      | 1.6 (2)                               | 1.21 (6)                |
|                             |          |                    | -47.957 (9)                              | 16:19:28.16 (2)            | -50:04:38.9 (2)                      | 0.22 (3)                              | 0.9 (1)                 |
|                             |          |                    | -47.352 (8)                              | 16:19:27.77 (2)            | -50:04:38.6 (2)                      | 0.53 (4)                              | 2.1 (3)                 |
|                             |          |                    | -46.46 (4)                               | 16:19:28.44 (4)            | -50:04:37.7 (4)                      | 0.7 (1)                               | 0.6 (2)                 |
|                             |          |                    | -45.6 (2)                                | 16:19:28.48 (6)            | -50:04:38.2 (5)                      | 1.4 (3)                               | 0.51 (4)                |
|                             |          | 44                 | -48.33 (2)                               | 16:19:28.224 (9)           | -50:04:39.11 (8)                     | 0.58 (3)                              | 3.5 (2)                 |
|                             |          |                    | -48.171 (6)                              | 16:19:28.26 (2)            | -50:04:39.3 (2)                      | 0.18 (2)                              | 2.4 (3)                 |
|                             |          |                    | -47.56 (3)                               | 16:19:28.23 (5)            | -50:04:38.7 (4)                      | 0.52 (8)                              | 1.04 (8)                |
|                             |          |                    | -46.77 (1)                               | 16:19:28.20 (2)            | -50:04:38.4 (1)                      | 0.33 (2)                              | 1.7 (1)                 |
|                             | C        | 36                 | -46.942 (9)                              | 16:19:28.09 (3)            | -50:04:44.8 (2)                      | 0.41 (2)                              | 1.30 (6)                |
|                             |          | 44                 | -47.187 (6)                              | 16:19:28.074 (8)           | -50:04:44.93 (6)                     | 0.49 (1)                              | 3.58 (8)                |
|                             | D        | 36                 | -46.26 (1)                               | 16:19:28.65 (1)            | -50:04:53.6 (1)                      | 0.60 (3)                              | 1.00 (4)                |
|                             |          |                    | -45.46 (2)                               | 16:19:28.77 (6)            | -50:04:54.0 (5)                      | 0.35 (6)                              | 0.60 (6)                |
|                             |          |                    | -44.961 (5)                              | 16:19:28.706 (5)           | -50:04:53.88 (4)                     | 0.43 (1)                              | 3.67 (5)                |
|                             |          | 44                 | -46.40 (1)                               | 16:19:28.62 (1)            | -50:04:54.4 (1)                      | 0.46 (2)                              | 2.36 (9)                |
|                             |          |                    | -45.23 (5)                               | 16:19:28.64 (8)            | -50:04:53.6 (5)                      | 1.0 (2)                               | 0.8 (3)                 |
|                             |          |                    | -45.160 (2)                              | 16:19:28.700 (5)           | -50:04:54.15 (4)                     | 0.348 (8)                             | 10.4 (3)                |
|                             | E        | 36                 | -54.01 (3)                               | 16:19:27.75 (2)            | -50:04:48.7 (2)                      | 1.19 (8)                              | 0.58 (3)                |
| G333.47-0.16                | A        | 36                 | -45.31 (9)                               | 16:21:19.71 (5)            | -50:09:45.6 (4)                      | 0.6 (1)                               | 0.68 (8)                |
|                             |          |                    | -45.06 (2)                               | 16:21:19.93 (3)            | -50:09:42.7 (2)                      | 0.22 (8)                              | 0.4 (3)                 |
|                             |          |                    | -44.71 (3)                               | 16:21:19.70 (3)            | -50:09:45.1 (3)                      | 0.33 (5)                              | 0.55 (8)                |
|                             |          |                    | -43.34 (1)                               | 16:21:19.92 (8)            | -50:09:39.6 (6)                      | 0.20 (3)                              | 0.47 (6)                |
|                             |          |                    | -42.49 (1)                               | 16:21:19.83 (9)            | -50:09:40.9 (7)                      | 0.23 (3)                              | 0.42 (5)                |
|                             |          | 44                 | -45.305 (4)                              | 16:21:19.866 (9)           | -50:09:41.72 (8)                     | 0.501 (9)                             | 7.00 (8)                |
|                             | B        |                    | -44.59 (4)                               | 16:21:19.95 (9)            | -50:09:42.0 (7)                      | 0.6 (1)                               | 0.73 (8)                |
|                             |          |                    | -41.164 (8)                              | 16:21:19.85 (3)            | -50:09:42.9 (2)                      | 0.24 (2)                              | 1.4 (1)                 |
|                             |          | 36                 | -41.73 (5)                               | 16:21:20.05 (4)            | -50:09:37.4 (3)                      | 0.34 (8)                              | 0.9 (5)                 |
|                             |          |                    | -41.49 (2)                               | 16:21:20.09 (1)            | -50:09:38.08 (9)                     | 0.19 (6)                              | 0.8 (5)                 |
|                             |          |                    | -41.4 (2)                                | 16:21:20.04 (4)            | -50:09:38.1 (3)                      | 0.5 (2)                               | 0.6 (3)                 |
|                             |          | 44                 | -41.91 (5)                               | 16:21:19.92 (5)            | -50:09:37.5 (4)                      | 0.90 (6)                              | 1.7 (1)                 |
|                             | C        |                    | -41.507 (6)                              | 16:21:20.06 (1)            | -50:09:37.61 (9)                     | 0.40 (2)                              | 3.2 (2)                 |
|                             |          | 44                 | -45.04 (1)                               | 16:21:20.57 (2)            | -50:09:54.2 (1)                      | 0.21 (3)                              | 0.9 (1)                 |
|                             |          |                    | -44.54 (8)                               | 16:21:20.54 (4)            | -50:09:53.6 (4)                      | 1.3 (1)                               | 0.76 (6)                |

Table 3 – continued

| Source name                 | Location | Frequency<br>(GHz) | LSR<br>velocity<br>(km s <sup>-1</sup> ) | $\alpha_{2000}$<br>(h:m:s) | $\delta_{2000}$<br>(°:arcmin:arcsec) | Line<br>FWHM<br>(km s <sup>-1</sup> ) | Flux<br>density<br>(Jy) |
|-----------------------------|----------|--------------------|------------------------------------------|----------------------------|--------------------------------------|---------------------------------------|-------------------------|
| G333.47-0.16<br>(continued) | C        | 44                 | -44.040 (6)                              | 16:21:20.58 (2)            | -50:09:54.6 (1)                      | 0.31 (2)                              | 2.5 (1)                 |
|                             |          |                    | -42.70 (4)                               | 16:21:20.48 (3)            | -50:09:55.4 (2)                      | 0.31 (4)                              | 2.3 (9)                 |
|                             | D        | 36                 | -43.6 (1)                                | 16:21:20.1 (1)             | -50:09:47.1 (7)                      | 1.7 (2)                               | 0.45 (5)                |
|                             |          |                    | -43.46 (1)                               | 16:21:20.20 (2)            | -50:09:47.2 (2)                      | 0.25 (4)                              | 0.49 (6)                |
|                             |          |                    | -43.098 (1)                              | 16:21:20.118 (3)           | -50:09:46.61 (2)                     | 0.216 (3)                             | 7.13 (8)                |
|                             |          |                    | -42.34 (3)                               | 16:21:20.42 (6)            | -50:09:46.7 (5)                      | 0.38 (8)                              | 0.34 (5)                |
|                             |          |                    | -41.3 (1)                                | 16:21:20.55 (8)            | -50:09:46.9 (5)                      | 2.5 (2)                               | 0.63 (3)                |
|                             |          |                    | -41.25 (1)                               | 16:21:20.44 (6)            | -50:09:46.5 (5)                      | 0.25 (3)                              | 0.54 (6)                |
|                             |          | 44                 | -43.56 (3)                               | 16:21:20.10 (3)            | -50:09:45.7 (3)                      | 1.54 (9)                              | 0.98 (8)                |
|                             |          |                    | -43.479 (2)                              | 16:21:20.041 (7)           | -50:09:46.20 (6)                     | 0.336 (6)                             | 7.0 (1)                 |
|                             | E        | 36                 | -43.85 (6)                               | 16:21:19.58 (9)            | -50:09:33.4 (7)                      | 0.7 (2)                               | 0.23 (4)                |
|                             |          |                    | -42.934 (9)                              | 16:21:19.61 (1)            | -50:09:33.69 (9)                     | 0.35 (2)                              | 4.64 (9)                |
|                             |          | 44                 | -42.68 (1)                               | 16:21:19.63 (3)            | -50:09:34.1 (2)                      | 0.23 (2)                              | 2.1 (3)                 |
|                             |          |                    | -44.19 (2)                               | 16:21:19.64 (1)            | -50:09:33.23 (9)                     | 0.62 (5)                              | 1.06 (8)                |
|                             |          |                    | -43.10 (1)                               | 16:21:19.57 (1)            | -50:09:33.9 (1)                      | 0.36 (2)                              | 12.1 (7)                |
|                             |          |                    | -42.85 (1)                               | 16:21:19.59 (1)            | -50:09:33.87 (9)                     | 0.32 (1)                              | 11 (1)                  |
|                             | F        | 36                 | -45.8 (1)                                | 16:21:21.24 (9)            | -50:09:42.8 (7)                      | 4.0 (4)                               | 0.26 (1)                |
|                             |          |                    | -42.33 (3)                               | 16:21:20.6 (1)             | -50:09:45.6 (7)                      | 0.4 (1)                               | 0.26 (5)                |
|                             |          |                    | -41.24 (8)                               | 16:21:20.54 (5)            | -50:09:46.0 (4)                      | 2.6 (2)                               | 0.54 (3)                |
|                             |          |                    | -41.16 (3)                               | 16:21:20.58 (8)            | -50:09:45.9 (5)                      | 0.45 (8)                              | 0.33 (5)                |
|                             |          |                    | -38.71 (2)                               | 16:21:20.9 (1)             | -50:09:45.5 (7)                      | 0.20 (4)                              | 0.40 (6)                |
|                             |          |                    | -38.934 (9)                              | 16:21:20.963 (8)           | -50:09:45.02 (8)                     | 0.37 (2)                              | 1.87 (9)                |
|                             |          | 44                 | -38.934 (9)                              | 16:21:20.963 (8)           | -50:09:45.02 (8)                     | 0.37 (2)                              | 1.87 (9)                |
|                             | G        | 36                 | -46.63 (9)                               | 16:21:19.84 (5)            | -50:09:50.5 (4)                      | 4.5 (2)                               | 0.36 (1)                |
|                             | H        | 36                 | -42.050 (8)                              | 16:21:19.16 (6)            | -50:09:40.7 (5)                      | 0.22 (2)                              | 0.85 (6)                |
| G333.56-0.02                | A        | 36                 | -39.834 (4)                              | 16:21:08.787 (4)           | -49:59:48.52 (3)                     | 0.528 (7)                             | 11.9 (3)                |
|                             |          |                    | -39.709 (2)                              | 16:21:08.77 (1)            | -49:59:48.6 (1)                      | 0.232 (6)                             | 7.0 (2)                 |
|                             |          |                    | -39.56 (1)                               | 16:21:08.81 (1)            | -49:59:48.6 (1)                      | 1.10 (2)                              | 3.7 (2)                 |
|                             |          | 44                 | -40.10 (2)                               | 16:21:08.76 (2)            | -49:59:48.3 (2)                      | 1.40 (3)                              | 8.3 (4)                 |
|                             |          |                    | -40.024 (2)                              | 16:21:08.751 (3)           | -49:59:48.48 (2)                     | 0.512 (4)                             | 36.0 (4)                |
|                             |          |                    | -39.432 (5)                              | 16:21:08.74 (1)            | -49:59:48.3 (1)                      | 0.53 (1)                              | 12.0 (3)                |
| G333.59-0.21                | A        | 44                 | -51.46 (2)                               | 16:22:06.68 (6)            | -50:06:19.3 (4)                      | 0.25 (4)                              | 2.0 (2)                 |
|                             |          |                    | -50.14 (3)                               | 16:22:06.66 (3)            | -50:06:19.0 (2)                      | 1.02 (8)                              | 2.4 (1)                 |
|                             |          |                    | -49.19 (3)                               | 16:22:06.64 (4)            | -50:06:18.4 (3)                      | 0.41 (8)                              | 2.0 (3)                 |
|                             |          |                    | -48.47 (9)                               | 16:22:06.67 (8)            | -50:06:20.4 (6)                      | 0.9 (2)                               | 1.1 (1)                 |
|                             | B        | 36                 | -49.374 (5)                              | 16:22:06.638 (9)           | -50:06:26.56 (6)                     | 0.56 (1)                              | 6.8 (1)                 |
|                             |          | 44                 | -49.574 (3)                              | 16:22:06.661 (8)           | -50:06:26.68 (6)                     | 0.534 (5)                             | 26.6 (2)                |
| G335.06-0.43                | A        | 36                 | -40.691 (2)                              | 16:29:23.456 (2)           | -49:12:20.17 (1)                     | 0.280 (4)                             | 5.00 (6)                |
|                             |          |                    | -39.4 (1)                                | 16:29:23.13 (9)            | -49:12:21.1 (7)                      | 3.5 (3)                               | 0.26 (2)                |
|                             |          | 44                 | -42.143 (6)                              | 16:29:23.48 (2)            | -49:12:22.6 (1)                      | 0.25 (2)                              | 3.0 (2)                 |
|                             |          |                    | -42.0 (1)                                | 16:29:23.33 (8)            | -49:12:23.3 (4)                      | 1.0 (3)                               | 0.6 (2)                 |
|                             |          |                    | -40.910 (2)                              | 16:29:23.456 (4)           | -49:12:20.37 (3)                     | 0.301 (6)                             | 16.8 (5)                |
|                             |          |                    | -40.69 (8)                               | 16:29:23.38 (3)            | -49:12:19.7 (2)                      | 0.67 (8)                              | 1.5 (3)                 |
|                             | B        | 36                 | -38.98 (4)                               | 16:29:23.23 (3)            | -49:12:19.6 (2)                      | 1.1 (1)                               | 0.92 (6)                |
|                             |          |                    | -37.83 (3)                               | 16:29:23.29 (3)            | -49:12:19.7 (2)                      | 0.57 (8)                              | 0.87 (9)                |
|                             |          |                    | -38.964 (6)                              | 16:29:22.806 (4)           | -49:12:31.90 (3)                     | 0.52 (1)                              | 2.20 (5)                |
|                             |          |                    | -38.1 (1)                                | 16:29:22.9 (2)             | -49:12:32 (1)                        | 0.5 (2)                               | 0.12 (5)                |
|                             |          | 44                 | -39.20 (1)                               | 16:29:22.80 (1)            | -49:12:32.05 (8)                     | 0.46 (2)                              | 7.6 (5)                 |
|                             |          |                    | -38.5 (6)                                | 16:29:22.85 (3)            | -49:12:31.1 (2)                      | 1 (1)                                 | 1.3 (8)                 |

**Table 3** – *continued*

| Source name                 | Location    | Frequency<br>(GHz) | LSR velocity<br>(km s <sup>-1</sup> ) | $\alpha_{2000}$<br>(h:m:s) | $\delta_{2000}$<br>( $^{\circ}$ :arcmin:arcsec) | Line FWHM<br>(km s <sup>-1</sup> ) | Flux density<br>(Jy) |         |
|-----------------------------|-------------|--------------------|---------------------------------------|----------------------------|-------------------------------------------------|------------------------------------|----------------------|---------|
| G335.06-0.43<br>(continued) | B           | 44                 | -38.140 (9)                           | 16:29:23.08 (2)            | -49:12:31.5 (1)                                 | 0.4 (1)                            | 4 (3)                |         |
|                             |             |                    | -37.62 (5)                            | 16:29:23.09 (5)            | -49:12:31.2 (4)                                 | 0.32 (8)                           | 1.3 (4)              |         |
|                             | C           | 36                 | -39.745 (7)                           | 16:29:21.47 (3)            | -49:12:27.8 (2)                                 | 0.21 (2)                           | 1.13 (8)             |         |
|                             | D           | 36                 | -41.23 (2)                            | 16:29:23.31 (6)            | -49:12:32.5 (4)                                 | 0.26 (4)                           | 0.50 (8)             |         |
|                             | E           | 36                 | -39.60 (4)                            | 16:29:25.10 (5)            | -49:12:27.7 (3)                                 | 0.65 (9)                           | 0.39 (5)             |         |
| -35.58 (8)                  |             |                    | 16:29:25.27 (2)                       | -49:12:28.2 (2)            | 1.6 (2)                                         | 0.33 (3)                           |                      |         |
| G335.59-0.29                | A           | 36                 | -44.852 (9)                           | 16:31:00.47 (3)            | -48:43:56.5 (2)                                 | 0.29 (3)                           | 1.1 (1)              |         |
|                             |             |                    | -44.53 (3)                            | 16:31:00.48 (5)            | -48:43:56.4 (4)                                 | 0.80 (4)                           | 1.21 (6)             |         |
|                             |             |                    | 44                                    | -48.160 (5)                | 16:31:00.39 (1)                                 | -48:43:53.81 (8)                   | 0.28 (2)             | 3.0 (2) |
|                             |             |                    |                                       | -48.10 (2)                 | 16:31:00.50 (8)                                 | -48:43:52.2 (8)                    | 0.79 (8)             | 1.4 (2) |
|                             |             |                    |                                       | -44.93 (3)                 | 16:31:00.30 (2)                                 | -48:43:55.2 (2)                    | 0.4 (1)              | 2 (1)   |
|                             | B           | 36                 | -44.6 (3)                             | 16:31:00.24 (4)            | -48:43:55.6 (3)                                 | 0.7 (3)                            | 1.4 (7)              |         |
|                             |             |                    | -43.441 (8)                           | 16:31:00.58 (2)            | -48:43:51.4 (1)                                 | 0.34 (2)                           | 1.82 (8)             |         |
|                             |             |                    | -51.8 (5)                             | 16:30:56.6 (1)             | -48:43:36.4 (8)                                 | 6 (1)                              | 0.32 (6)             |         |
|                             |             |                    | -48.4 (1)                             | 16:30:56.62 (5)            | -48:43:37.0 (3)                                 | 3.1 (2)                            | 1.10 (6)             |         |
|                             |             |                    | -46.84 (2)                            | 16:30:56.46 (4)            | -48:43:36.1 (3)                                 | 1.46 (4)                           | 4.23 (9)             |         |
|                             |             |                    | -45.8 (3)                             | 16:30:56.44 (2)            | -48:43:34.3 (2)                                 | 0.9 (2)                            | 24 (20)              |         |
|                             |             |                    | -45.55 (3)                            | 16:30:56.446 (2)           | -48:43:33.59 (1)                                | 0.59 (6)                           | 115 (30)             |         |
|                             |             |                    | -45.268 (3)                           | 16:30:56.455 (2)           | -48:43:33.60 (2)                                | 0.41 (1)                           | 144 (20)             |         |
|                             |             |                    | -44.69 (2)                            | 16:30:56.39 (3)            | -48:43:33.6 (2)                                 | 0.27 (3)                           | 3.3 (3)              |         |
|                             |             |                    | 44                                    | -47.5 (5)                  | 16:30:56.4 (1)                                  | -48:43:35.3 (8)                    | 1.2 (8)              | 0.7 (2) |
|                             | -46.88 (2)  | 16:30:56.34 (3)    |                                       | -48:43:35.5 (2)            | 0.54 (8)                                        | 3.2 (8)                            |                      |         |
|                             | -45.640 (3) | 16:30:56.472 (4)   |                                       | -48:43:33.54 (3)           | 0.704 (5)                                       | 61 (1)                             |                      |         |
|                             | -45.544 (1) | 16:30:56.477 (4)   |                                       | -48:43:33.50 (3)           | 0.357 (3)                                       | 75 (1)                             |                      |         |
|                             | -44.77 (1)  | 16:30:56.38 (3)    |                                       | -48:43:33.8 (2)            | 0.28 (3)                                        | 2.5 (2)                            |                      |         |
|                             | C           | 44                 | -45.61 (5)                            | 16:31:04.3 (1)             | -48:43:43.2 (8)                                 | 1.8 (2)                            | 3.5 (4)              |         |
|                             |             |                    | -45.578 (5)                           | 16:31:04.35 (5)            | -48:43:43.9 (4)                                 | 0.40 (2)                           | 15.0 (5)             |         |
|                             | D           | 36                 | -44.82 (1)                            | 16:30:57.129 (6)           | -48:43:50.44 (5)                                | 0.21 (2)                           | 12 (8)               |         |
|                             |             |                    | -44.71 (9)                            | 16:30:57.116 (8)           | -48:43:50.20 (8)                                | 0.28 (8)                           | 7 (5)                |         |
|                             |             |                    | -44.34 (3)                            | 16:30:57.17 (8)            | -48:43:49.9 (6)                                 | 0.80 (3)                           | 1.06 (8)             |         |
|                             | 44          | 44                 | -44.993 (6)                           | 16:30:57.15 (3)            | -48:43:49.9 (2)                                 | 0.21 (2)                           | 2.2 (1)              |         |
|                             |             |                    | -43.73 (2)                            | 16:30:59.80 (2)            | -48:43:51.0 (2)                                 | 0.39 (4)                           | 0.93 (8)             |         |
|                             | F           | 44                 | -47.832 (5)                           | 16:30:58.61 (1)            | -48:43:55.0 (1)                                 | 0.33 (1)                           | 2.8 (1)              |         |
|                             |             |                    | -47.1 (1)                             | 16:30:58.74 (4)            | -48:43:54.0 (3)                                 | 1.4 (2)                            | 0.39 (4)             |         |
|                             | G           | 36                 | -50.7 (2)                             | 16:30:58.66 (8)            | -48:44:12.0 (6)                                 | 4.9 (5)                            | 0.42 (2)             |         |
|                             |             |                    | -47.7 (1)                             | 16:30:58.31 (5)            | -48:44:05.1 (4)                                 | 1.6 (2)                            | 1.0 (1)              |         |
|                             |             |                    | -47.03 (1)                            | 16:30:58.311 (9)           | -48:44:05.16 (8)                                | 0.60 (4)                           | 2.7 (2)              |         |
|                             |             |                    | -46.45 (2)                            | 16:30:58.31 (2)            | -48:44:04.9 (1)                                 | 0.42 (3)                           | 1.7 (1)              |         |
|                             |             |                    | -48.51 (9)                            | 16:30:58.32 (4)            | -48:44:05.3 (3)                                 | 1.7 (2)                            | 0.93 (5)             |         |
|                             |             |                    | -47.41 (2)                            | 16:30:58.36 (3)            | -48:44:04.8 (2)                                 | 0.43 (6)                           | 1.6 (3)              |         |
|                             | H           | 36                 | -46.85 (9)                            | 16:30:58.34 (4)            | -48:44:05.9 (3)                                 | 1.1 (1)                            | 1.6 (1)              |         |
|                             |             |                    | -48.70 (3)                            | 16:30:58.47 (4)            | -48:43:35.1 (4)                                 | 0.46 (8)                           | 0.7 (2)              |         |
|                             |             |                    | -48.1 (2)                             | 16:30:58.5 (1)             | -48:43:35.3 (8)                                 | 0.9 (3)                            | 0.38 (6)             |         |
|                             |             |                    | -44.51 (4)                            | 16:30:58.53 (9)            | -48:43:44.8 (7)                                 | 0.57 (8)                           | 0.50 (5)             |         |
|                             |             |                    | -43.58 (5)                            | 16:30:58.80 (6)            | -48:43:38.8 (5)                                 | 0.8 (2)                            | 0.41 (8)             |         |
|                             |             |                    | -42.44 (2)                            | 16:30:58.61 (2)            | -48:43:32.4 (2)                                 | 0.52 (3)                           | 2.3 (1)              |         |
| -41.9 (1)                   |             |                    | 16:30:58.52 (8)                       | -48:43:33.0 (5)            | 0.6 (2)                                         | 0.5 (1)                            |                      |         |
| -40.8 (2)                   |             |                    | 16:30:58.5 (1)                        | -48:43:32.6 (7)            | 3.8 (4)                                         | 0.52 (2)                           |                      |         |



Table 3 – continued

| Source name                 | Location | Frequency<br>(GHz) | LSR<br>velocity<br>(km s <sup>-1</sup> ) | $\alpha_{2000}$<br>(h:m:s) | $\delta_{2000}$<br>(°:arcmin:arcsec) | Line<br>FWHM<br>(km s <sup>-1</sup> ) | Flux<br>density<br>(Jy) |
|-----------------------------|----------|--------------------|------------------------------------------|----------------------------|--------------------------------------|---------------------------------------|-------------------------|
| G335.59-0.29<br>(continued) | I        | 36                 | -44.961 (8)                              | 16:31:03.85 (1)            | -48:43:01.2 (1)                      | 0.51 (2)                              | 9.7 (3)                 |
|                             | J        | 36                 | -43.1 (1)                                | 16:31:01.2 (1)             | -48:43:50.7 (9)                      | 1.2 (2)                               | 1.0 (1)                 |
|                             |          |                    | -41.92 (8)                               | 16:31:01.34 (4)            | -48:43:51.4 (3)                      | 1.1 (1)                               | 1.1 (2)                 |
|                             |          |                    | -40.7 (5)                                | 16:31:01.3 (2)             | -48:43:51 (1)                        | 3.3 (7)                               | 0.48 (6)                |
| G335.79+0.17                | A        | 44                 | -52.64 (2)                               | 16:29:47.70 (3)            | -48:16:08.8 (3)                      | 0.67 (4)                              | 1.45 (8)                |
|                             |          |                    | -50.219 (4)                              | 16:29:47.662 (7)           | -48:16:06.68 (6)                     | 0.546 (8)                             | 6.30 (8)                |
|                             | B        | 36                 | -48.78 (2)                               | 16:29:47.67 (5)            | -48:16:06.6 (4)                      | 0.58 (5)                              | 1.10 (8)                |
|                             |          |                    | -51.483 (5)                              | 16:29:47.02 (3)            | -48:15:59.9 (2)                      | 0.16 (1)                              | 1.49 (9)                |
|                             |          |                    | -48.86 (1)                               | 16:29:47.14 (3)            | -48:15:58.4 (2)                      | 0.52 (3)                              | 1.20 (6)                |
|                             | C        | 44                 | -51.707 (3)                              | 16:29:46.99 (1)            | -48:16:00.01 (9)                     | 0.191 (6)                             | 4.3 (1)                 |
|                             |          |                    | -49.21 (2)                               | 16:29:47.12 (3)            | -48:15:58.5 (3)                      | 0.50 (5)                              | 1.3 (1)                 |
|                             |          |                    | -52.26 (5)                               | 16:29:46.89 (8)            | -48:15:48.7 (4)                      | 0.7 (1)                               | 0.39 (5)                |
|                             |          |                    | -50.49 (2)                               | 16:29:47.17 (2)            | -48:15:48.7 (2)                      | 0.49 (5)                              | 1.1 (1)                 |
|                             |          |                    | -49.941 (5)                              | 16:29:46.98 (4)            | -48:15:50.9 (3)                      | 0.16 (1)                              | 2.4 (1)                 |
|                             |          |                    | -49.628 (7)                              | 16:29:47.15 (1)            | -48:15:48.76 (9)                     | 0.36 (2)                              | 2.8 (1)                 |
|                             |          | 44                 | -49.50 (6)                               | 16:29:46.9 (2)             | -48:15:49.6 (9)                      | 2.34 (9)                              | 1.6 (1)                 |
|                             |          |                    | -48.87 (1)                               | 16:29:46.92 (1)            | -48:15:50.76 (8)                     | 0.26 (3)                              | 1.9 (1)                 |
|                             |          |                    | -48.48 (1)                               | 16:29:46.95 (2)            | -48:15:50.7 (1)                      | 0.32 (4)                              | 2.1 (1)                 |
|                             |          |                    | -48.104 (6)                              | 16:29:46.946 (8)           | -48:15:50.63 (6)                     | 0.26 (1)                              | 3.8 (1)                 |
|                             |          |                    | -51.18 (1)                               | 16:29:47.29 (2)            | -48:15:47.1 (2)                      | 0.47 (3)                              | 4.8 (1)                 |
|                             |          |                    | -50.720 (5)                              | 16:29:47.30 (1)            | -48:15:47.23 (8)                     | 0.32 (1)                              | 9.2 (2)                 |
|                             |          |                    | -50.153 (2)                              | 16:29:46.914 (6)           | -48:15:51.69 (4)                     | 0.216 (5)                             | 14.4 (3)                |
|                             |          |                    | -49.66 (2)                               | 16:29:47.06 (3)            | -48:15:49.2 (3)                      | 0.91 (9)                              | 3.5 (1)                 |
|                             |          |                    | -48.933 (3)                              | 16:29:46.91 (2)            | -48:15:51.1 (2)                      | 0.31 (1)                              | 7.4 (3)                 |
|                             |          |                    | -48.705 (1)                              | 16:29:46.928 (1)           | -48:15:50.927 (8)                    | 0.211 (2)                             | 40.3 (3)                |
|                             |          |                    | -48.343 (2)                              | 16:29:46.926 (2)           | -48:15:50.80 (2)                     | 0.313 (3)                             | 23.9 (1)                |
|                             | D        | 44                 | -50.14 (1)                               | 16:29:46.96 (1)            | -48:15:40.6 (1)                      | 0.61 (3)                              | 3.5 (1)                 |
|                             | E        | 36                 | -48.83 (1)                               | 16:29:45.4 (1)             | -48:15:34.5 (7)                      | 0.32 (3)                              | 1.7 (1)                 |
|                             |          | 44                 | -49.020 (3)                              | 16:29:45.412 (7)           | -48:15:34.95 (6)                     | 0.313 (7)                             | 11.8 (2)                |
|                             | F        | 44                 | -47.93 (1)                               | 16:29:45.36 (2)            | -48:15:30.2 (2)                      | 0.17 (3)                              | 3.6 (4)                 |
|                             |          |                    | -47.9 (6)                                | 16:29:45.37 (8)            | -48:15:30.4 (6)                      | 2.7 (8)                               | 1.3 (2)                 |
|                             | G        | 36                 | -52.78 (3)                               | 16:29:47.45 (8)            | -48:15:44.2 (6)                      | 0.61 (8)                              | 0.65 (8)                |
|                             | H        | 36                 | -51.40 (1)                               | 16:29:47.56 (8)            | -48:15:36.7 (5)                      | 0.26 (3)                              | 1.4 (1)                 |
| G336.41-0.26                | A        | 36                 | -87.55 (5)                               | 16:34:13.7 (1)             | -48:06:21.3 (9)                      | 1.5 (1)                               | 0.58 (9)                |
|                             |          |                    | -87.419 (1)                              | 16:34:13.819 (4)           | -48:06:22.44 (3)                     | 0.468 (3)                             | 19.09 (9)               |
|                             |          | 44                 | -87.802 (8)                              | 16:34:13.811 (4)           | -48:06:22.22 (3)                     | 0.386 (7)                             | 44 (3)                  |
|                             |          |                    | -87.68 (3)                               | 16:34:13.73 (4)            | -48:06:20.6 (4)                      | 1.4 (1)                               | 1.7 (2)                 |
|                             |          |                    | -87.53 (1)                               | 16:34:13.808 (2)           | -48:06:22.24 (2)                     | 0.42 (1)                              | 42 (2)                  |
|                             |          |                    | -87.53 (1)                               | 16:34:13.808 (2)           | -48:06:22.24 (2)                     | 0.42 (1)                              | 42 (2)                  |
|                             | B        | 36                 | -90.55 (1)                               | 16:34:13.29 (2)            | -48:06:14.1 (1)                      | 0.41 (3)                              | 0.99 (6)                |
|                             |          |                    | -89.74 (1)                               | 16:34:13.27 (1)            | -48:06:13.96 (8)                     | 0.89 (3)                              | 3.19 (4)                |
|                             |          |                    | -88.57 (4)                               | 16:34:13.28 (4)            | -48:06:13.7 (3)                      | 1.13 (9)                              | 0.99 (3)                |
|                             |          |                    | -86.65 (3)                               | 16:34:13.22 (5)            | -48:06:13.7 (3)                      | 0.84 (8)                              | 0.52 (4)                |
|                             |          | 44                 | -90.733 (9)                              | 16:34:13.26 (1)            | -48:06:13.80 (9)                     | 0.42 (2)                              | 3.9 (2)                 |
|                             |          |                    | -90.045 (4)                              | 16:34:13.248 (2)           | -48:06:13.82 (2)                     | 0.57 (2)                              | 12.1 (8)                |
|                             |          |                    | -89.50 (1)                               | 16:34:13.259 (6)           | -48:06:13.66 (6)                     | 0.24 (4)                              | 2.0 (3)                 |
|                             |          |                    | -89.32 (8)                               | 16:34:13.29 (1)            | -48:06:13.7 (1)                      | 1.4 (1)                               | 5.8 (3)                 |

**Table 3** – *continued*

| Source name  | Location | Frequency (GHz) | LSR velocity (km s <sup>-1</sup> ) | $\alpha_{2000}$ (h:m:s) | $\delta_{2000}$ (°:arcmin:arcsec) | Line FWHM (km s <sup>-1</sup> ) | Flux density (Jy) |
|--------------|----------|-----------------|------------------------------------|-------------------------|-----------------------------------|---------------------------------|-------------------|
| G336.41-0.26 | B        | 44              | -87.01 (4)                         | 16:34:13.36 (4)         | -48:06:13.2 (3)                   | 0.95 (9)                        | 1.12 (8)          |
| G337.40-0.40 | A        | 36              | -44.46 (4)                         | 16:38:50.55 (2)         | -47:28:03.1 (2)                   | 0.57 (8)                        | 1.06 (6)          |
|              |          |                 | -43.998 (4)                        | 16:38:50.517 (4)        | -47:28:02.08 (3)                  | 0.350 (8)                       | 5.6 (1)           |
|              |          |                 | -42.22 (3)                         | 16:38:50.55 (3)         | -47:28:02.7 (2)                   | 0.33 (6)                        | 0.44 (8)          |
|              |          |                 | -39.86 (6)                         | 16:38:50.52 (3)         | -47:27:59.8 (2)                   | 4.3 (2)                         | 0.69 (2)          |
|              |          | 44              | -45.40 (1)                         | 16:38:50.502 (7)        | -47:28:03.16 (5)                  | 0.75 (3)                        | 3.41 (8)          |
|              |          |                 | -44.811 (5)                        | 16:38:50.507 (3)        | -47:28:03.17 (3)                  | 0.32 (1)                        | 5.6 (1)           |
|              |          |                 | -44.263 (1)                        | 16:38:50.514 (2)        | -47:28:02.04 (2)                  | 0.534 (2)                       | 49.0 (1)          |
|              |          |                 | -43.22 (4)                         | 16:38:50.51 (4)         | -47:28:01.9 (3)                   | 1.5 (1)                         | 1.68 (5)          |
|              |          |                 | -42.409 (1)                        | 16:38:50.554 (1)        | -47:28:03.258 (9)                 | 0.296 (1)                       | 41.7 (1)          |
|              |          |                 | -41.32 (1)                         | 16:38:50.748 (8)        | -47:28:04.81 (6)                  | 0.26 (2)                        | 5.9 (8)           |
|              |          |                 | -41.08 (5)                         | 16:38:50.76 (1)         | -47:28:04.9 (1)                   | 0.36 (6)                        | 2.8 (4)           |
|              |          |                 | -40.28 (2)                         | 16:38:50.77 (2)         | -47:28:05.1 (1)                   | 0.42 (3)                        | 5.4 (2)           |
|              |          |                 | -40.027 (7)                        | 16:38:50.782 (7)        | -47:28:05.04 (5)                  | 0.23 (2)                        | 4.3 (7)           |
|              |          |                 | -39.615 (8)                        | 16:38:50.783 (7)        | -47:28:01.40 (6)                  | 0.45 (3)                        | 3.7 (1)           |
|              |          |                 | -39.14 (2)                         | 16:38:50.78 (4)         | -47:28:01.1 (3)                   | 0.22 (5)                        | 0.9 (2)           |
|              |          |                 | -38.74 (3)                         | 16:38:49.78 (3)         | -47:28:10.7 (2)                   | 0.44 (8)                        | 0.92 (9)          |
|              |          |                 | -37.95 (2)                         | 16:38:50.07 (5)         | -47:28:06.6 (3)                   | 0.20 (6)                        | 0.5 (1)           |
|              |          |                 | -36.95 (5)                         | 16:38:49.91 (2)         | -47:28:06.4 (2)                   | 0.55 (6)                        | 4.0 (4)           |
|              |          |                 | -36.706 (8)                        | 16:38:49.887 (8)        | -47:28:06.42 (6)                  | 0.25 (5)                        | 3 (1)             |
|              |          |                 | -36.331 (4)                        | 16:38:49.913 (3)        | -47:28:06.59 (2)                  | 0.286 (7)                       | 7.8 (2)           |
|              |          |                 | -35.376 (6)                        | 16:38:50.041 (6)        | -47:28:03.02 (4)                  | 0.24 (1)                        | 2.4 (1)           |
|              | B        | 36              | -44.89 (4)                         | 16:38:46.86 (3)         | -47:27:59.3 (3)                   | 1.3 (1)                         | 0.70 (5)          |
|              | C        | 36              | -40.55 (1)                         | 16:38:50.87 (4)         | -47:27:40.1 (3)                   | 0.19 (2)                        | 1.2 (1)           |
|              | D        | 36              | -38.53 (2)                         | 16:38:49.75 (3)         | -47:28:10.4 (3)                   | 0.41 (5)                        | 0.47 (4)          |
|              | E        | 36              | -36.53 (5)                         | 16:38:49.94 (5)         | -47:28:05.8 (4)                   | 0.9 (1)                         | 0.29 (3)          |
| G337.92-0.46 | A        | 36              | -43.5 (1)                          | 16:41:09.07 (6)         | -47:08:09.7 (5)                   | 1.2 (4)                         | 0.17 (9)          |
|              |          |                 | -43.44 (1)                         | 16:41:09.171 (2)        | -47:08:08.73 (2)                  | 0.31 (1)                        | 19 (1)            |
|              |          |                 | -43.306 (3)                        | 16:41:09.183 (4)        | -47:08:08.80 (4)                  | 0.208 (6)                       | 19 (2)            |
|              |          | 44              | -44.01 (8)                         | 16:41:09.13 (3)         | -47:08:08.2 (2)                   | 0.6 (1)                         | 3.3 (1)           |
|              |          |                 | -43.66 (1)                         | 16:41:09.149 (1)        | -47:08:08.47 (1)                  | 0.378 (9)                       | 239 (20)          |
|              |          |                 | -43.494 (5)                        | 16:41:09.153 (1)        | -47:08:08.52 (1)                  | 0.306 (6)                       | 178 (30)          |
|              |          |                 | -43.01 (1)                         | 16:41:09.18 (2)         | -47:08:08.5 (1)                   | 0.17 (2)                        | 2.6 (3)           |
|              |          |                 | -40.40 (2)                         | 16:41:09.85 (1)         | -47:08:18.9 (1)                   | 0.56 (5)                        | 0.99 (8)          |
|              | B        | 44              | -40.40 (2)                         | 16:41:09.85 (1)         | -47:08:18.9 (1)                   | 0.56 (5)                        | 0.99 (8)          |
|              |          |                 | -38.77 (3)                         | 16:41:10.05 (6)         | -47:08:26.2 (6)                   | 0.45 (8)                        | 0.56 (8)          |
|              | C        | 36              | -38.06 (2)                         | 16:41:10.12 (3)         | -47:08:26.5 (3)                   | 0.46 (6)                        | 0.73 (8)          |
|              |          |                 | -36.95 (3)                         | 16:41:09.95 (8)         | -47:08:26.3 (5)                   | 0.64 (8)                        | 0.58 (6)          |
|              |          | 44              | -45.18 (2)                         | 16:41:09.86 (4)         | -47:08:25.9 (3)                   | 0.26 (6)                        | 0.8 (1)           |
|              |          |                 | -44.0 (5)                          | 16:41:10.00 (8)         | -47:08:26.1 (5)                   | 1.0 (5)                         | 1 (1)             |
|              |          |                 | -39.03 (5)                         | 16:41:10.06 (2)         | -47:08:26.1 (2)                   | 0.39 (6)                        | 3.2 (4)           |
|              |          |                 | -38.71 (2)                         | 16:41:10.18 (2)         | -47:08:25.5 (2)                   | 0.32 (6)                        | 4.0 (9)           |
|              |          |                 | -38.30 (2)                         | 16:41:10.06 (2)         | -47:08:25.9 (1)                   | 0.52 (4)                        | 5.6 (2)           |
|              |          |                 | -37.48 (8)                         | 16:41:09.96 (3)         | -47:08:25.6 (3)                   | 0.4 (1)                         | 2.3 (5)           |
|              |          |                 | -37.13 (3)                         | 16:41:09.99 (1)         | -47:08:26.1 (1)                   | 0.36 (4)                        | 4.5 (8)           |
|              |          |                 | -39.52 (2)                         | 16:41:12.49 (3)         | -47:08:15.5 (2)                   | 0.41 (4)                        | 3.0 (3)           |
|              | D        | 44              | -39.52 (2)                         | 16:41:12.49 (3)         | -47:08:15.5 (2)                   | 0.41 (4)                        | 3.0 (3)           |
|              | E        | 44              | -39.48 (3)                         | 16:41:10.48 (5)         | -47:08:01.5 (3)                   | 0.34 (8)                        | 0.55 (9)          |
|              |          |                 | -38.7 (1)                          | 16:41:10.32 (4)         | -47:08:02.9 (3)                   | 3.5 (3)                         | 0.43 (3)          |
|              | F        | 44              | -39.49 (2)                         | 16:41:04.69 (3)         | -47:08:05.9 (2)                   | 0.55 (6)                        | 1.3 (1)           |

Table 3 – continued

| Source name                 | Location | Frequency<br>(GHz) | LSR<br>velocity<br>(km s <sup>-1</sup> ) | $\alpha_{2000}$<br>(h:m:s) | $\delta_{2000}$<br>(°:arcmin:arcsec) | Line<br>FWHM<br>(km s <sup>-1</sup> ) | Flux<br>density<br>(Jy) |
|-----------------------------|----------|--------------------|------------------------------------------|----------------------------|--------------------------------------|---------------------------------------|-------------------------|
| G337.92-0.46<br>(continued) | F        | 44                 | -37.4 (3)                                | 16:41:04.6 (1)             | -47:08:07.5 (8)                      | 3.1 (8)                               | 0.25 (5)                |
|                             | G        | 36                 | -41.981 (8)                              | 16:41:06.25 (2)            | -47:07:01.1 (1)                      | 0.40 (2)                              | 5.0 (2)                 |
|                             | H        | 36                 | -41.7 (2)                                | 16:41:04.8 (1)             | -47:07:12 (1)                        | 1.0 (5)                               | 0.4 (1)                 |
|                             |          |                    | -40.97 (2)                               | 16:41:04.90 (6)            | -47:07:11.0 (5)                      | 0.36 (5)                              | 2.1 (2)                 |
| G338.92+0.55                | I        | 36                 | -39.595 (6)                              | 16:41:04.43 (1)            | -47:07:32.6 (1)                      | 0.24 (1)                              | 2.6 (1)                 |
|                             | A        | 36                 | -62.810 (1)                              | 16:40:33.265 (2)           | -45:42:00.72 (2)                     | 0.508 (1)                             | 90.3 (1)                |
|                             |          |                    | -62.301 (1)                              | 16:40:33.261 (1)           | -45:42:00.62 (1)                     | 0.388 (1)                             | 63.0 (1)                |
|                             |          | 44                 | -63.060 (1)                              | 16:40:33.278 (2)           | -45:42:00.53 (1)                     | 0.507 (1)                             | 157.7 (2)               |
|                             |          |                    | -62.502 (1)                              | 16:40:33.270 (1)           | -45:42:00.473 (5)                    | 0.377 (2)                             | 95.0 (3)                |
|                             | B        | 44                 | -64.046 (5)                              | 16:40:33.69 (4)            | -45:42:06.7 (3)                      | 0.50 (1)                              | 4.8 (1)                 |
|                             | C        | 36                 | -65.21 (3)                               | 16:40:34.07 (6)            | -45:42:10.0 (5)                      | 0.71 (6)                              | 1.01 (8)                |
|                             |          |                    | -63.68 (4)                               | 16:40:34.3 (1)             | -45:42:08 (1)                        | 1.4 (1)                               | 1.10 (8)                |
|                             |          | 44                 | -63.41 (1)                               | 16:40:34.20 (2)            | -45:42:07.5 (2)                      | 0.26 (4)                              | 1.1 (1)                 |
|                             |          |                    | -66.701 (6)                              | 16:40:34.08 (2)            | -45:42:08.7 (1)                      | 0.34 (1)                              | 6.1 (3)                 |
|                             |          |                    | -66.113 (9)                              | 16:40:34.07 (1)            | -45:42:08.97 (8)                     | 0.73 (5)                              | 6.7 (1)                 |
|                             |          |                    | -65.648 (8)                              | 16:40:34.08 (3)            | -45:42:09.2 (2)                      | 0.20 (3)                              | 2.4 (3)                 |
|                             | D        | 36                 | -65.0 (1)                                | 16:40:33.75 (3)            | -45:42:09.7 (2)                      | 0.6 (3)                               | 2 (4)                   |
|                             |          |                    | -64.536 (6)                              | 16:40:33.72 (2)            | -45:42:09.5 (1)                      | 0.14 (2)                              | 2.3 (3)                 |
|                             |          |                    | -64.5 (8)                                | 16:40:33.69 (5)            | -45:42:07.5 (5)                      | 1 (1)                                 | 2 (2)                   |
|                             |          |                    | -63.641 (6)                              | 16:40:34.10 (2)            | -45:42:06.9 (1)                      | 0.35 (2)                              | 5.2 (4)                 |
|                             |          | 44                 | -64.89 (3)                               | 16:40:34.27 (5)            | -45:42:13.6 (4)                      | 0.78 (6)                              | 0.99 (8)                |
|                             |          |                    | -65.251 (8)                              | 16:40:34.363 (9)           | -45:42:14.26 (8)                     | 0.37 (1)                              | 10.4 (2)                |
|                             |          | 36                 | -64.850 (6)                              | 16:40:34.350 (4)           | -45:42:14.31 (3)                     | 0.37 (1)                              | 15.4 (2)                |
|                             |          |                    | -65.832 (4)                              | 16:40:34.80 (2)            | -45:41:58.3 (1)                      | 0.33 (1)                              | 5.3 (1)                 |
|                             |          |                    | -65.63 (3)                               | 16:40:34.72 (5)            | -45:41:58.8 (4)                      | 2.25 (8)                              | 2.33 (8)                |
|                             |          |                    | -63.72 (3)                               | 16:40:34.49 (6)            | -45:41:59.0 (5)                      | 0.66 (8)                              | 0.99 (9)                |
|                             |          |                    | -61.724 (7)                              | 16:40:34.57 (2)            | -45:41:58.3 (1)                      | 0.26 (2)                              | 2.4 (1)                 |
|                             |          |                    | -67.721 (8)                              | 16:40:34.87 (1)            | -45:41:58.34 (8)                     | 0.39 (3)                              | 3.6 (2)                 |
|                             | E        | 44                 | -66.89 (1)                               | 16:40:34.91 (3)            | -45:41:58.5 (2)                      | 0.30 (4)                              | 2.0 (2)                 |
|                             |          |                    | -66.13 (9)                               | 16:40:34.80 (6)            | -45:41:57.8 (4)                      | 2.4 (2)                               | 1.5 (2)                 |
|                             |          |                    | -66.036 (2)                              | 16:40:34.817 (8)           | -45:41:58.12 (6)                     | 0.332 (6)                             | 14.0 (2)                |
|                             |          |                    | -65.51 (3)                               | 16:40:34.79 (4)            | -45:41:57.8 (3)                      | 0.13 (8)                              | 0.5 (3)                 |
|                             |          | 36                 | -64.00 (3)                               | 16:40:34.60 (6)            | -45:41:57.5 (3)                      | 0.52 (8)                              | 1.2 (1)                 |
|                             |          |                    | -61.99 (6)                               | 16:40:34.6 (2)             | -45:41:58 (1)                        | 0.6 (2)                               | 0.8 (3)                 |
|                             |          |                    | -61.943 (6)                              | 16:40:34.59 (2)            | -45:41:58.6 (1)                      | 0.18 (2)                              | 3.8 (4)                 |
|                             |          |                    | -77.65 (3)                               | 16:40:34.26 (2)            | -45:41:33.2 (2)                      | 0.93 (6)                              | 1.45 (8)                |
|                             |          |                    | -73.55 (1)                               | 16:40:34.27 (1)            | -45:41:33.5 (1)                      | 0.62 (3)                              | 2.7 (1)                 |
|                             |          |                    | -66.38 (4)                               | 16:40:34.20 (3)            | -45:41:34.3 (3)                      | 0.5 (1)                               | 0.8 (1)                 |
|                             |          |                    | -58.48 (2)                               | 16:40:34.08 (6)            | -45:41:34.0 (6)                      | 0.86 (4)                              | 2.02 (9)                |
|                             |          |                    | -77.88 (1)                               | 16:40:34.30 (2)            | -45:41:33.4 (1)                      | 1.11 (3)                              | 5.1 (1)                 |
|                             |          | 44                 | -73.830 (7)                              | 16:40:34.269 (9)           | -45:41:33.57 (8)                     | 0.56 (2)                              | 5.0 (1)                 |
|                             |          |                    | -58.61 (1)                               | 16:40:34.29 (3)            | -45:41:32.8 (2)                      | 0.65 (3)                              | 3.4 (1)                 |
|                             | G        | 36                 | -61.65 (2)                               | 16:40:35.81 (2)            | -45:41:36.0 (2)                      | 0.94 (4)                              | 5.5 (2)                 |
|                             |          |                    | -60.285 (3)                              | 16:40:35.59 (5)            | -45:41:28.3 (4)                      | 0.808 (6)                             | 21.8 (2)                |
|                             |          |                    | -60.229 (1)                              | 16:40:35.804 (2)           | -45:41:28.48 (2)                     | 0.371 (1)                             | 190.4 (3)               |
|                             |          |                    | -58.81 (1)                               | 16:40:35.46 (4)            | -45:41:24.8 (3)                      | 1.02 (2)                              | 8.7 (2)                 |
|                             | H        | 44                 | -60.416 (1)                              | 16:40:35.815 (3)           | -45:41:28.31 (2)                     | 0.304 (1)                             | 383.2 (8)               |
|                             |          |                    | -63.20 (1)                               | 16:40:34.075 (9)           | -45:41:43.06 (9)                     | 1.16 (3)                              | 4.5 (1)                 |

**Table 3** – *continued*

| Source name                        | Location         | Frequency<br>(GHz) | LSR velocity<br>(km s <sup>-1</sup> ) | $\alpha_{2000}$<br>(h:m:s) | $\delta_{2000}$<br>( <sup>o</sup> :arcmin:arcsec) | Line FWHM<br>(km s <sup>-1</sup> ) | Flux density<br>(Jy) |                  |          |          |
|------------------------------------|------------------|--------------------|---------------------------------------|----------------------------|---------------------------------------------------|------------------------------------|----------------------|------------------|----------|----------|
| G338.92+0.55<br><i>(continued)</i> | H                | 36                 | -63.087 (2)                           | 16:40:34.040 (5)           | -45:41:43.13 (4)                                  | 0.240 (7)                          | 6.6 (2)              |                  |          |          |
|                                    |                  |                    | -61.72 (2)                            | 16:40:34.12 (2)            | -45:41:42.6 (1)                                   | 0.89 (5)                           | 3.38 (8)             |                  |          |          |
|                                    |                  |                    | -60.68 (1)                            | 16:40:33.99 (2)            | -45:41:41.5 (2)                                   | 0.74 (5)                           | 5.16 (8)             |                  |          |          |
|                                    |                  |                    | -60.113 (6)                           | 16:40:33.88 (1)            | -45:41:39.7 (1)                                   | 0.36 (2)                           | 9.7 (3)              |                  |          |          |
|                                    |                  |                    | -59.73 (1)                            | 16:40:33.81 (2)            | -45:41:42.2 (2)                                   | 0.31 (3)                           | 4.9 (4)              |                  |          |          |
|                                    |                  | -59.35 (2)         | 16:40:33.77 (4)                       | -45:41:41.5 (3)            | 0.50 (4)                                          | 4.2 (1)                            |                      |                  |          |          |
|                                    |                  | 44                 | -61.944 (9)                           | 16:40:33.624 (9)           | -45:41:42.28 (6)                                  | 0.57 (2)                           | 12.0 (2)             |                  |          |          |
|                                    |                  |                    | -61.245 (7)                           | 16:40:33.705 (5)           | -45:41:42.12 (3)                                  | 0.61 (2)                           | 16.0 (2)             |                  |          |          |
|                                    |                  |                    | -60.342 (2)                           | 16:40:33.866 (3)           | -45:41:39.37 (2)                                  | 0.17 (1)                           | 28 (5)               |                  |          |          |
|                                    |                  |                    | -60.003 (1)                           | 16:40:33.785 (6)           | -45:41:42.38 (4)                                  | 0.295 (4)                          | 54.2 (4)             |                  |          |          |
|                                    | I                |                    | 36                                    | -60.842 (5)                | 16:40:33.38 (4)                                   | -45:41:35.6 (4)                    | 0.20 (1)             | 2.5 (1)          |          |          |
|                                    |                  | -59.515 (2)        |                                       | 16:40:33.175 (6)           | -45:41:35.80 (5)                                  | 0.390 (8)                          | 14.1 (5)             |                  |          |          |
|                                    |                  | -59.18 (5)         |                                       | 16:40:33.39 (2)            | -45:41:35.5 (1)                                   | 0.78 (5)                           | 3.0 (3)              |                  |          |          |
|                                    |                  | -58.363 (5)        |                                       | 16:40:33.46 (2)            | -45:41:34.7 (2)                                   | 0.28 (1)                           | 4.0 (1)              |                  |          |          |
|                                    |                  | -57.807 (8)        |                                       | 16:40:33.46 (1)            | -45:41:35.6 (1)                                   | 0.54 (2)                           | 3.09 (8)             |                  |          |          |
|                                    |                  | 44                 | -61.447 (3)                           | 16:40:33.32 (1)            | -45:41:35.43 (8)                                  | 0.235 (7)                          | 7.6 (2)              |                  |          |          |
|                                    |                  |                    | -61.081 (2)                           | 16:40:33.346 (8)           | -45:41:35.46 (6)                                  | 0.230 (4)                          | 13.3 (2)             |                  |          |          |
|                                    |                  |                    | -59.766 (8)                           | 16:40:33.176 (6)           | -45:41:35.62 (4)                                  | 0.35 (1)                           | 27 (5)               |                  |          |          |
|                                    |                  |                    | -59.50 (8)                            | 16:40:33.19 (2)            | -45:41:35.4 (1)                                   | 0.5 (1)                            | 13 (3)               |                  |          |          |
|                                    |                  |                    | -58.9 (4)                             | 16:40:33.35 (6)            | -45:41:34.9 (4)                                   | 0.8 (6)                            | 0.8 (3)              |                  |          |          |
|                                    |                  |                    | -57.48 (4)                            | 16:40:33.55 (3)            | -45:41:32.5 (2)                                   | 1.09 (9)                           | 1.56 (8)             |                  |          |          |
|                                    |                  |                    | -63.99 (3)                            | 16:40:35.40 (4)            | -45:41:42.7 (3)                                   | 1.65 (8)                           | 1.45 (6)             |                  |          |          |
| G339.88-1.26                       | A                | 36                 | -31.679 (4)                           | 16:52:05.495 (4)           | -46:08:40.83 (3)                                  | 0.448 (9)                          | 2.65 (5)             |                  |          |          |
|                                    |                  | 44                 | -32.51 (3)                            | 16:52:05.43 (8)            | -46:08:41.1 (5)                                   | 0.25 (8)                           | 0.6 (1)              |                  |          |          |
|                                    |                  |                    | -32.144 (8)                           | 16:52:05.49 (1)            | -46:08:40.7 (1)                                   | 0.27 (2)                           | 6.4 (1)              |                  |          |          |
|                                    |                  |                    | -31.872 (4)                           | 16:52:05.494 (2)           | -46:08:40.96 (1)                                  | 0.23 (1)                           | 10.6 (4)             |                  |          |          |
|                                    |                  |                    | -31.60 (1)                            | 16:52:05.49 (2)            | -46:08:41.6 (2)                                   | 0.31 (2)                           | 5.3 (2)              |                  |          |          |
|                                    | B                | 36                 | -31.6 (2)                             | 16:52:03.2 (1)             | -46:08:13.5 (8)                                   | 2.5 (4)                            | 0.17 (3)             |                  |          |          |
|                                    |                  |                    | -31.07 (3)                            | 16:52:03.06 (8)            | -46:08:13.9 (5)                                   | 0.39 (8)                           | 0.39 (8)             |                  |          |          |
|                                    |                  | 44                 | -31.33 (1)                            | 16:52:03.11 (2)            | -46:08:14.5 (1)                                   | 0.43 (3)                           | 1.9 (1)              |                  |          |          |
|                                    |                  |                    | G341.19-0.23                          | A                          | 36                                                | -70.22 (6)                         | 16:52:16.35 (8)      | -44:28:43.4 (5)  | 1.6 (1)  | 0.53 (4) |
|                                    |                  |                    |                                       |                            |                                                   | -62.643 (6)                        | 16:52:16.351 (7)     | -44:28:44.34 (5) | 0.56 (2) | 3.26 (8) |
| -62.3 (1)                          | 16:52:16.3 (1)   | -44:28:44.2 (8)    |                                       |                            |                                                   | 4.1 (4)                            | 0.45 (4)             |                  |          |          |
| -58.55 (4)                         | 16:52:16.32 (5)  | -44:28:44.7 (3)    |                                       |                            |                                                   | 1.1 (1)                            | 0.64 (5)             |                  |          |          |
| -56.98 (5)                         | 16:52:16.28 (8)  | -44:28:44.7 (4)    |                                       |                            |                                                   | 0.8 (1)                            | 0.55 (6)             |                  |          |          |
| -55.48 (1)                         | 16:52:16.32 (2)  | -44:28:43.8 (1)    |                                       |                            |                                                   | 1.26 (4)                           | 2.56 (5)             |                  |          |          |
| -53.12 (4)                         | 16:52:16.30 (3)  | -44:28:43.9 (2)    |                                       |                            |                                                   | 2.0 (1)                            | 1.62 (4)             |                  |          |          |
| -51.99 (1)                         | 16:52:16.29 (3)  | -44:28:43.8 (2)    |                                       |                            |                                                   | 0.39 (3)                           | 1.9 (1)              |                  |          |          |
| -51.25 (3)                         | 16:52:16.324 (2) | -44:28:44.14 (1)   |                                       |                            |                                                   | 0.75 (4)                           | 6.5 (7)              |                  |          |          |
| -50.33 (5)                         | 16:52:16.332 (9) | -44:28:44.16 (6)   |                                       |                            |                                                   | 1.1 (3)                            | 5.7 (3)              |                  |          |          |
| -49.4 (1)                          | 16:52:16.333 (9) | -44:28:44.24 (6)   | 0.8 (2)                               | 2 (1)                      |                                                   |                                    |                      |                  |          |          |
| -48.768 (7)                        | 16:52:16.326 (6) | -44:28:44.17 (4)   | 0.37 (2)                              | 4.0 (3)                    |                                                   |                                    |                      |                  |          |          |
| -48.25 (4)                         | 16:52:16.33 (3)  | -44:28:44.2 (2)    | 0.68 (8)                              | 1.6 (1)                    |                                                   |                                    |                      |                  |          |          |
| -46.4 (2)                          | 16:52:16.35 (3)  | -44:28:44.2 (2)    | 5.4 (6)                               | 0.83 (2)                   |                                                   |                                    |                      |                  |          |          |
| -42.26 (4)                         | 16:52:16.30 (2)  | -44:28:43.5 (2)    | 0.77 (8)                              | 2.7 (1)                    |                                                   |                                    |                      |                  |          |          |
| -41.85 (2)                         | 16:52:16.288 (2) | -44:28:43.56 (2)   | 0.28 (1)                              | 58 (8)                     |                                                   |                                    |                      |                  |          |          |
| -41.733 (3)                        | 16:52:16.296 (3) | -44:28:43.52 (2)   | 0.206 (7)                             | 57 (10)                    |                                                   |                                    |                      |                  |          |          |
| -41.335 (7)                        | 16:52:16.408 (8) | -44:28:43.34 (5)   | 0.25 (2)                              | 9 (3)                      |                                                   |                                    |                      |                  |          |          |

Table 3 – continued

| Source name                 | Location        | Frequency<br>(GHz) | LSR<br>velocity<br>(km s <sup>-1</sup> ) | $\alpha$ 2000<br>(h:m:s) | $\delta$ 2000<br>( $^{\circ}$ :arcmin:arcsec) | Line<br>FWHM<br>(km s <sup>-1</sup> ) | Flux<br>density<br>(Jy) |                  |          |          |
|-----------------------------|-----------------|--------------------|------------------------------------------|--------------------------|-----------------------------------------------|---------------------------------------|-------------------------|------------------|----------|----------|
| G341.19-0.23<br>(continued) | A               | 36                 | -41.2 (1)                                | 16:52:16.44 (2)          | -44:28:42.7 (1)                               | 0.4 (1)                               | 3 (2)                   |                  |          |          |
|                             |                 |                    | -38.59 (3)                               | 16:52:16.42 (3)          | -44:28:43.0 (2)                               | 2.56 (8)                              | 1.23 (3)                |                  |          |          |
|                             |                 |                    | -34.6 (1)                                | 16:52:16.45 (1)          | -44:28:43.14 (9)                              | 1.2 (1)                               | 2.7 (4)                 |                  |          |          |
|                             |                 |                    | -34.345 (9)                              | 16:52:16.430 (6)         | -44:28:43.17 (4)                              | 0.39 (4)                              | 2.1 (3)                 |                  |          |          |
|                             |                 |                    | -33.51 (8)                               | 16:52:16.44 (3)          | -44:28:43.0 (2)                               | 1.08 (9)                              | 3.1 (4)                 |                  |          |          |
|                             |                 |                    | -31.34 (1)                               | 16:52:16.43 (3)          | -44:28:43.1 (2)                               | 0.40 (4)                              | 1.2 (1)                 |                  |          |          |
|                             |                 |                    | -31.14 (8)                               | 16:52:16.7 (1)           | -44:28:43.7 (6)                               | 1.7 (2)                               | 0.60 (8)                |                  |          |          |
|                             |                 |                    | -26.5 (1)                                | 16:52:16.2 (1)           | -44:28:42.5 (7)                               | 3.7 (3)                               | 0.35 (3)                |                  |          |          |
|                             |                 |                    | -16.97 (2)                               | 16:52:16.38 (1)          | -44:28:42.93 (8)                              | 0.90 (4)                              | 1.98 (5)                |                  |          |          |
|                             |                 |                    | -15.94 (4)                               | 16:52:16.34 (3)          | -44:28:42.7 (2)                               | 0.71 (8)                              | 0.81 (6)                |                  |          |          |
|                             |                 | 44                 | -50.2 (2)                                | 16:52:16.29 (3)          | -44:28:44.4 (2)                               | 3.1 (4)                               | 0.88 (9)                |                  |          |          |
|                             |                 |                    | -49.01 (3)                               | 16:52:16.33 (1)          | -44:28:43.9 (1)                               | 0.31 (8)                              | 1.5 (3)                 |                  |          |          |
|                             |                 |                    | -44.9 (2)                                | 16:52:16.35 (3)          | -44:28:43.2 (3)                               | 3.2 (6)                               | 0.80 (9)                |                  |          |          |
|                             |                 |                    | -42.47 (3)                               | 16:52:16.30 (1)          | -44:28:43.49 (9)                              | 0.70 (6)                              | 7.8 (3)                 |                  |          |          |
|                             |                 |                    | -42.043 (1)                              | 16:52:16.275 (1)         | -44:28:43.397 (6)                             | 0.317 (2)                             | 101.1 (9)               |                  |          |          |
|                             |                 |                    | -41.49 (2)                               | 16:52:16.416 (2)         | -44:28:42.96 (2)                              | 0.21 (4)                              | 5 (2)                   |                  |          |          |
|                             |                 |                    | -41.26 (9)                               | 16:52:16.46 (2)          | -44:28:42.6 (2)                               | 0.4 (1)                               | 2.9 (6)                 |                  |          |          |
|                             |                 |                    | G341.22-0.21                             | A                        | 36                                            | -45.98 (2)                            | 16:52:18.15 (8)         | -44:26:52.6 (5)  | 0.27 (5) | 0.45 (8) |
|                             |                 |                    |                                          |                          |                                               | -44.82 (1)                            | 16:52:18.200 (8)        | -44:26:52.67 (5) | 0.52 (2) | 3.04 (6) |
|                             |                 |                    |                                          |                          |                                               | -44.49 (1)                            | 16:52:18.36 (4)         | -44:26:51.7 (3)  | 0.21 (3) | 1.0 (2)  |
| -43.29 (1)                  | 16:52:18.58 (8) | -44:26:53.9 (5)    |                                          |                          |                                               | 0.22 (3)                              | 0.58 (8)                |                  |          |          |
| -42.673 (4)                 | 16:52:18.29 (2) | -44:26:53.0 (1)    |                                          |                          |                                               | 0.31 (1)                              | 2.15 (6)                |                  |          |          |
| -42.113 (6)                 | 16:52:18.50 (6) | -44:26:52.2 (4)    |                                          |                          |                                               | 0.20 (1)                              | 1.36 (8)                |                  |          |          |
| -42.0 (2)                   | 16:52:18.60 (8) | -44:26:52.0 (7)    |                                          |                          |                                               | 5.0 (4)                               | 0.33 (3)                |                  |          |          |
| -40.74 (3)                  | 16:52:18.56 (3) | -44:26:53.7 (2)    |                                          |                          |                                               | 0.72 (8)                              | 0.50 (4)                |                  |          |          |
| 44                          | -46.152 (5)     | 16:52:18.16 (1)    |                                          |                          |                                               | -44:26:52.50 (8)                      | 0.26 (1)                | 2.54 (9)         |          |          |
|                             | -45.029 (7)     | 16:52:18.18 (1)    |                                          |                          |                                               | -44:26:52.64 (8)                      | 0.59 (1)                | 7.26 (8)         |          |          |
|                             | -44.61 (1)      | 16:52:18.25 (5)    | -44:26:52.0 (4)                          | 0.28 (4)                 | 2.3 (2)                                       |                                       |                         |                  |          |          |
|                             | -44.26 (2)      | 16:52:18.54 (2)    | -44:26:50.0 (2)                          | 0.31 (5)                 | 2.1 (1)                                       |                                       |                         |                  |          |          |
|                             | -43.61 (2)      | 16:52:18.0 (1)     | -44:26:53.2 (9)                          | 0.57 (8)                 | 1.95 (8)                                      |                                       |                         |                  |          |          |
|                             | -42.956 (3)     | 16:52:18.126 (9)   | -44:26:53.33 (8)                         | 0.398 (7)                | 7.75 (8)                                      |                                       |                         |                  |          |          |
|                             | B               | 36                 | -43.683 (2)                              | 16:52:17.681 (5)         | -44:26:55.60 (3)                              | 0.326 (3)                             | 7.40 (6)                |                  |          |          |
|                             |                 |                    | -43.041 (1)                              | 16:52:17.632 (5)         | -44:26:55.98 (3)                              | 0.274 (2)                             | 9.40 (8)                |                  |          |          |
|                             |                 |                    | -41.86 (4)                               | 16:52:17.20 (4)          | -44:26:55.5 (2)                               | 0.4 (1)                               | 0.32 (8)                |                  |          |          |
|                             |                 |                    | -41.0 (1)                                | 16:52:17.0 (1)           | -44:26:57.2 (8)                               | 1.6 (3)                               | 0.30 (3)                |                  |          |          |
| 44                          |                 |                    | -43.892 (1)                              | 16:52:17.683 (3)         | -44:26:55.59 (2)                              | 0.381 (3)                             | 20.8 (2)                |                  |          |          |
|                             |                 |                    | -43.39 (4)                               | 16:52:17.62 (4)          | -44:26:56.0 (3)                               | 1.37 (8)                              | 1.6 (2)                 |                  |          |          |
|                             |                 |                    | -43.298 (1)                              | 16:52:17.642 (5)         | -44:26:55.97 (3)                              | 0.325 (3)                             | 19.6 (2)                |                  |          |          |
|                             |                 |                    | C                                        | 36                       | -44.65 (2)                                    | 16:52:17.85 (6)                       | -44:26:45.9 (4)         | 0.23 (4)         | 0.78 (8) |          |
|                             |                 |                    |                                          |                          | -44.28 (3)                                    | 16:52:17.76 (8)                       | -44:26:46.3 (5)         | 0.3 (1)          | 0.59 (8) |          |
| -43.96 (3)                  |                 |                    |                                          |                          | 16:52:17.90 (8)                               | -44:26:46.5 (5)                       | 0.22 (8)                | 0.51 (9)         |          |          |
| 44                          | -45.55 (8)      | 16:52:17.88 (6)    |                                          |                          | -44:26:46.2 (4)                               | 1.2 (2)                               | 0.56 (4)                |                  |          |          |
|                             | -44.887 (5)     | 16:52:17.88 (2)    |                                          |                          | -44:26:46.2 (2)                               | 0.12 (2)                              | 1.9 (2)                 |                  |          |          |
|                             | -44.652 (9)     | 16:52:17.89 (3)    |                                          | -44:26:46.4 (2)          | 0.38 (3)                                      | 3.6 (1)                               |                         |                  |          |          |
|                             | -44.181 (9)     | 16:52:17.912 (9)   |                                          | -44:26:46.36 (8)         | 0.28 (2)                                      | 4.1 (2)                               |                         |                  |          |          |
|                             | -43.794 (4)     | 16:52:18.045 (9)   |                                          | -44:26:46.81 (8)         | 0.23 (3)                                      | 5 (2)                                 |                         |                  |          |          |
| -43.6 (4)                   | 16:52:18.16 (6) | -44:26:49.4 (6)    |                                          | 0.5 (4)                  | 0.7 (7)                                       |                                       |                         |                  |          |          |
| -42.13 (3)                  | 16:52:17.89 (4) | -44:26:46.8 (3)    |                                          | 0.51 (8)                 | 0.56 (6)                                      |                                       |                         |                  |          |          |

**Table 3** – *continued*

| Source name                 | Location | Frequency<br>(GHz) | LSR<br>velocity<br>(km s <sup>-1</sup> ) | $\alpha_{2000}$<br>(h:m:s) | $\delta_{2000}$<br>(°:arcmin:arcsec) | Line<br>FWHM<br>(km s <sup>-1</sup> ) | Flux<br>density<br>(Jy) |
|-----------------------------|----------|--------------------|------------------------------------------|----------------------------|--------------------------------------|---------------------------------------|-------------------------|
| G341.22-0.21<br>(continued) | D        | 44                 | -42.04 (1)                               | 16:52:16.24 (5)            | -44:27:26.4 (4)                      | 0.39 (3)                              | 3.0 (2)                 |
|                             | E        | 36                 | -44.2 (1)                                | 16:52:18.61 (9)            | -44:26:39.4 (6)                      | 3.1 (2)                               | 0.44 (4)                |
|                             |          |                    | -43.58 (2)                               | 16:52:18.64 (2)            | -44:26:39.6 (1)                      | 0.71 (6)                              | 0.84 (5)                |
|                             |          |                    | -42.42 (2)                               | 16:52:18.67 (5)            | -44:26:39.8 (4)                      | 0.40 (8)                              | 0.46 (6)                |
| G343.12-0.06                | F        | 36                 | -41.54 (2)                               | 16:52:16.22 (9)            | -44:26:53.7 (4)                      | 0.35 (4)                              | 0.71 (8)                |
|                             |          |                    | -33.1 (2)                                | 16:58:16.56 (6)            | -42:52:29.5 (4)                      | 0.8 (1)                               | 2.6 (9)                 |
|                             |          |                    | -32.684 (9)                              | 16:58:16.590 (3)           | -42:52:29.51 (2)                     | 0.671 (8)                             | 23 (1)                  |
|                             | A        | 36                 | -31.693 (5)                              | 16:58:16.49 (3)            | -42:52:27.6 (2)                      | 0.52 (1)                              | 3.24 (5)                |
|                             |          |                    | -33.2 (2)                                | 16:58:16.57 (2)            | -42:52:29.4 (2)                      | 1.1 (1)                               | 12 (3)                  |
|                             |          |                    | -32.906 (3)                              | 16:58:16.586 (2)           | -42:52:29.55 (2)                     | 0.66 (1)                              | 68 (5)                  |
|                             |          | 44                 | -32.433 (4)                              | 16:58:16.57 (1)            | -42:52:29.3 (1)                      | 0.29 (1)                              | 9.6 (9)                 |
|                             |          |                    | -31.91 (1)                               | 16:58:16.48 (3)            | -42:52:27.9 (3)                      | 0.46 (2)                              | 7.4 (5)                 |
|                             |          |                    | -31.513 (2)                              | 16:58:16.460 (9)           | -42:52:25.76 (6)                     | 0.253 (4)                             | 17.6 (4)                |
|                             | B        | 36                 | -31.19 (1)                               | 16:58:16.49 (4)            | -42:52:25.7 (3)                      | 0.58 (2)                              | 3.67 (6)                |
|                             |          |                    | -31.8 (2)                                | 16:58:16.46 (4)            | -42:52:25.3 (3)                      | 2.2 (2)                               | 2.4 (5)                 |
|                             |          |                    | -31.630 (1)                              | 16:58:16.50 (1)            | -42:52:25.4 (1)                      | 0.280 (4)                             | 21.5 (5)                |
|                             | C        | 36                 | -31.616 (2)                              | 16:58:16.46 (2)            | -42:52:26.3 (2)                      | 0.67 (1)                              | 23.6 (5)                |
|                             |          |                    | -31.065 (5)                              | 16:58:16.65 (9)            | -42:52:21.6 (6)                      | 0.27 (1)                              | 2.53 (6)                |
|                             |          |                    | -30.595 (8)                              | 16:58:16.69 (2)            | -42:52:20.9 (1)                      | 0.41 (2)                              | 1.62 (5)                |
|                             |          | 44                 | -31.287 (3)                              | 16:58:16.68 (9)            | -42:52:21.4 (8)                      | 0.258 (8)                             | 6.4 (1)                 |
|                             |          |                    | -30.852 (2)                              | 16:58:16.69 (1)            | -42:52:20.80 (9)                     | 0.273 (3)                             | 12.6 (1)                |
|                             |          |                    | -30.81 (1)                               | 16:58:16.78 (5)            | -42:51:59.2 (3)                      | 0.22 (5)                              | 1.0 (3)                 |
|                             | D        | 36                 | -30.58 (4)                               | 16:58:16.77 (4)            | -42:51:59.2 (2)                      | 0.46 (6)                              | 1.4 (1)                 |
|                             |          |                    | -31.06 (3)                               | 16:58:16.821 (7)           | -42:51:59.23 (8)                     | 0.44 (3)                              | 13 (1)                  |
|                             |          |                    | -30.71 (2)                               | 16:58:16.814 (3)           | -42:51:59.55 (3)                     | 0.39 (5)                              | 14 (3)                  |
|                             | E        | 36                 | -30.37 (6)                               | 16:58:16.82 (1)            | -42:51:59.78 (9)                     | 0.51 (6)                              | 8 (1)                   |
|                             |          |                    | -30.15 (2)                               | 16:58:17.52 (4)            | -42:52:03.5 (3)                      | 0.31 (6)                              | 0.43 (8)                |
|                             |          |                    | -33.399 (9)                              | 16:58:17.51 (3)            | -42:52:05.7 (3)                      | 0.28 (2)                              | 2.1 (1)                 |
|                             |          | 44                 | -31.271 (5)                              | 16:58:17.573 (6)           | -42:52:04.39 (6)                     | 0.28 (1)                              | 4.1 (1)                 |
|                             |          |                    | -30.7 (2)                                | 16:58:17.58 (4)            | -42:52:06.8 (5)                      | 4.7 (4)                               | 0.59 (6)                |
|                             |          |                    | -30.411 (2)                              | 16:58:17.540 (5)           | -42:52:04.12 (4)                     | 0.431 (5)                             | 12.1 (1)                |
|                             | F        | 36                 | -28.905 (6)                              | 16:58:17.888 (8)           | -42:52:05.50 (8)                     | 0.40 (1)                              | 4.0 (1)                 |
|                             |          |                    | -29.025 (5)                              | 16:58:15.981 (6)           | -42:51:58.36 (4)                     | 0.42 (1)                              | 2.49 (6)                |
|                             |          |                    | -27.45 (2)                               | 16:58:16.17 (1)            | -42:52:00.91 (9)                     | 0.34 (3)                              | 8.4 (7)                 |
|                             |          |                    | -27.43 (2)                               | 16:58:16.23 (5)            | -42:52:01.5 (3)                      | 1.07 (5)                              | 2.6 (3)                 |
|                             |          |                    | -27.264 (2)                              | 16:58:16.21 (1)            | -42:52:01.15 (8)                     | 0.214 (5)                             | 25 (2)                  |
|                             |          |                    | -27.039 (4)                              | 16:58:16.146 (7)           | -42:52:00.69 (5)                     | 0.293 (8)                             | 16.9 (3)                |
|                             |          | 44                 | -26.34 (1)                               | 16:58:16.06 (5)            | -42:51:59.7 (3)                      | 0.29 (3)                              | 1.14 (8)                |
|                             |          |                    | -29.233 (4)                              | 16:58:15.993 (6)           | -42:51:58.52 (5)                     | 0.449 (9)                             | 6.5 (1)                 |
|                             |          |                    | -27.70 (1)                               | 16:58:16.140 (3)           | -42:52:00.85 (3)                     | 0.30 (2)                              | 18 (1)                  |
|                             |          |                    | -27.611 (8)                              | 16:58:16.11 (2)            | -42:52:00.7 (2)                      | 0.94 (2)                              | 14.8 (9)                |
|                             |          |                    | -27.481 (2)                              | 16:58:16.191 (3)           | -42:52:01.21 (3)                     | 0.227 (3)                             | 83 (2)                  |
|                             |          |                    | -27.228 (2)                              | 16:58:16.142 (3)           | -42:52:00.92 (2)                     | 0.288 (3)                             | 71.8 (8)                |
|                             | G        | 36                 | -20.80 (2)                               | 16:58:15.71 (8)            | -42:52:36.8 (4)                      | 0.43 (5)                              | 0.46 (5)                |
|                             |          | 44                 | -21.83 (2)                               | 16:58:15.75 (4)            | -42:52:37.2 (3)                      | 0.38 (4)                              | 1.06 (9)                |
|                             | H        | 36                 | -21.07 (1)                               | 16:58:15.86 (3)            | -42:52:36.6 (3)                      | 0.36 (2)                              | 1.7 (1)                 |
|                             |          |                    | -29.94 (2)                               | 16:58:17.31 (4)            | -42:51:51.4 (3)                      | 0.20 (4)                              | 0.7 (1)                 |
|                             |          |                    | -28.40 (6)                               | 16:58:17.26 (4)            | -42:51:51.4 (3)                      | 0.3 (2)                               | 0.19 (9)                |

Table 3 – continued

| Source name                 | Location | Frequency<br>(GHz) | LSR<br>velocity<br>(km s <sup>-1</sup> ) | $\alpha_{2000}$<br>(h:m:s) | $\delta_{2000}$<br>(°:arcmin:arcsec) | Line<br>FWHM<br>(km s <sup>-1</sup> ) | Flux<br>density<br>(Jy) |
|-----------------------------|----------|--------------------|------------------------------------------|----------------------------|--------------------------------------|---------------------------------------|-------------------------|
| G343.12-0.06<br>(continued) | H        | 36                 | -28.15 (8)                               | 16:58:17.38 (6)            | -42:51:51.4 (4)                      | 3.0 (2)                               | 0.51 (3)                |
|                             |          | 44                 | -30.154 (4)                              | 16:58:17.174 (3)           | -42:51:51.38 (3)                     | 0.376 (7)                             | 23.6 (2)                |
|                             |          |                    | -29.82 (1)                               | 16:58:17.16 (2)            | -42:51:51.5 (2)                      | 0.27 (3)                              | 4.4 (4)                 |
|                             |          |                    | -28.47 (2)                               | 16:58:17.17 (1)            | -42:51:51.3 (1)                      | 0.39 (5)                              | 2.0 (2)                 |
|                             |          |                    | -28.20 (8)                               | 16:58:17.25 (5)            | -42:51:51.6 (5)                      | 2.4 (2)                               | 1.3 (1)                 |
|                             | I        | 36                 | -33.56 (1)                               | 16:58:16.3 (1)             | -42:51:53.6 (8)                      | 0.39 (3)                              | 0.89 (8)                |
|                             |          | 44                 | -33.7 (3)                                | 16:58:16.64 (9)            | -42:51:55.4 (6)                      | 2 (1)                                 | 0.3 (3)                 |
|                             |          |                    | -33.743 (9)                              | 16:58:16.39 (2)            | -42:51:55.1 (2)                      | 0.56 (3)                              | 4.6 (3)                 |
|                             | J        | 36                 | -33.56 (8)                               | 16:58:16.12 (8)            | -42:51:41.5 (6)                      | 0.5 (2)                               | 0.41 (9)                |
|                             |          |                    | -33.144 (7)                              | 16:58:15.99 (2)            | -42:51:42.9 (1)                      | 0.19 (2)                              | 2.1 (2)                 |
| G344.23-0.57                | A        | 36                 | -24.73 (8)                               | 17:04:05.51 (8)            | -42:18:51.9 (4)                      | 1.3 (2)                               | 0.30 (3)                |
|                             |          |                    | -20.35 (3)                               | 17:04:05.72 (3)            | -42:18:51.8 (2)                      | 0.52 (8)                              | 0.44 (5)                |
|                             |          | 44                 | -25.179 (9)                              | 17:04:05.56 (1)            | -42:18:51.8 (1)                      | 0.35 (4)                              | 2.6 (4)                 |
|                             | B        |                    | -24.8 (2)                                | 17:04:05.47 (5)            | -42:18:50.8 (5)                      | 0.8 (2)                               | 0.7 (1)                 |
|                             |          | 36                 | -23.965 (2)                              | 17:04:06.415 (8)           | -42:18:58.82 (5)                     | 0.319 (4)                             | 5.35 (6)                |
|                             |          | 44                 | -24.183 (2)                              | 17:04:06.422 (5)           | -42:18:58.79 (5)                     | 0.381 (4)                             | 14.3 (1)                |
|                             | C        |                    | -22.9 (1)                                | 17:04:06.20 (6)            | -42:18:57.2 (5)                      | 2.6 (3)                               | 0.58 (4)                |
|                             |          | 36                 | -23.64 (1)                               | 17:04:08.82 (2)            | -42:18:24.7 (1)                      | 0.41 (3)                              | 1.30 (6)                |
|                             |          |                    | -22.869 (5)                              | 17:04:08.79 (2)            | -42:18:25.9 (2)                      | 0.17 (1)                              | 1.6 (1)                 |
|                             |          |                    | -22.645 (6)                              | 17:04:08.81 (2)            | -42:18:25.2 (1)                      | 0.79 (1)                              | 4.42 (6)                |
|                             |          |                    | -21.37 (4)                               | 17:04:08.75 (4)            | -42:18:27.3 (3)                      | 0.8 (1)                               | 0.46 (5)                |
|                             |          | 44                 | -23.805 (8)                              | 17:04:08.856 (8)           | -42:18:24.59 (8)                     | 0.58 (2)                              | 3.31 (8)                |
|                             |          |                    | -22.891 (2)                              | 17:04:08.842 (5)           | -42:18:24.61 (4)                     | 0.688 (8)                             | 13.2 (1)                |
|                             |          |                    | -21.731 (5)                              | 17:04:08.80 (1)            | -42:18:26.6 (1)                      | 0.29 (1)                              | 3.1 (1)                 |
|                             |          |                    | -21.4 (3)                                | 17:04:08.83 (8)            | -42:18:27.4 (7)                      | 2.2 (5)                               | 0.37 (5)                |
|                             | D        | 36                 | -23.112 (6)                              | 17:04:06.38 (1)            | -42:19:10.31 (9)                     | 0.43 (1)                              | 2.60 (8)                |
|                             |          | 44                 | -23.316 (5)                              | 17:04:06.381 (9)           | -42:19:10.52 (8)                     | 0.38 (1)                              | 4.8 (1)                 |
|                             | E        | 36                 | -22.11 (1)                               | 17:04:08.67 (8)            | -42:18:53.7 (5)                      | 0.27 (3)                              | 0.68 (6)                |
|                             |          | 44                 | -22.265 (2)                              | 17:04:08.808 (7)           | -42:18:53.30 (6)                     | 0.334 (5)                             | 7.55 (9)                |
|                             | F        | 36                 | -21.670 (6)                              | 17:04:05.019 (7)           | -42:18:36.90 (5)                     | 0.31 (1)                              | 5.84 (9)                |
|                             |          |                    | -21.37 (1)                               | 17:04:05.12 (3)            | -42:18:36.8 (2)                      | 0.26 (2)                              | 2.0 (1)                 |
|                             |          | 44                 | -22.5 (1)                                | 17:04:05.01 (8)            | -42:18:38.5 (7)                      | 1.6 (2)                               | 0.70 (8)                |
|                             | G        |                    | -21.956 (5)                              | 17:04:05.04 (1)            | -42:18:37.3 (1)                      | 0.36 (1)                              | 5.2 (1)                 |
|                             |          | 36                 | -20.781 (5)                              | 17:04:07.31 (1)            | -42:18:40.27 (8)                     | 0.51 (1)                              | 5.8 (1)                 |
|                             |          |                    | -20.58 (2)                               | 17:04:07.38 (9)            | -42:18:39.8 (7)                      | 1.95 (9)                              | 1.2 (1)                 |
|                             |          |                    | -20.429 (3)                              | 17:04:07.368 (7)           | -42:18:40.27 (5)                     | 0.14 (1)                              | 2.5 (2)                 |
|                             |          |                    | -20.243 (7)                              | 17:04:07.32 (1)            | -42:18:40.73 (8)                     | 0.39 (1)                              | 6.6 (1)                 |
|                             |          | 44                 | -21.981 (5)                              | 17:04:07.24 (2)            | -42:18:40.4 (2)                      | 0.23 (1)                              | 2.3 (1)                 |
|                             |          |                    | -21.122 (5)                              | 17:04:07.33 (9)            | -42:18:40.7 (8)                      | 0.472 (9)                             | 8.1 (1)                 |
|                             |          |                    | -20.642 (2)                              | 17:04:07.298 (9)           | -42:18:40.64 (8)                     | 0.151 (6)                             | 5.7 (2)                 |
|                             |          |                    | -20.425 (3)                              | 17:04:07.296 (3)           | -42:18:40.95 (3)                     | 0.652 (4)                             | 29.96 (9)               |
|                             |          |                    | -19.57 (2)                               | 17:04:07.29 (5)            | -42:18:41.6 (4)                      | 0.29 (5)                              | 0.66 (9)                |
|                             | H        | 36                 | -21.179 (9)                              | 17:04:07.41 (8)            | -42:18:44.6 (5)                      | 0.25 (2)                              | 1.62 (8)                |
|                             |          | 44                 | -21.396 (2)                              | 17:04:07.44 (1)            | -42:18:44.9 (1)                      | 0.286 (4)                             | 7.66 (8)                |
|                             | I        | 36                 | -18.6 (1)                                | 17:04:07.78 (8)            | -42:18:40.1 (4)                      | 4.8 (2)                               | 0.56 (2)                |
|                             |          |                    | -17.02 (2)                               | 17:04:07.88 (2)            | -42:18:39.3 (1)                      | 0.65 (4)                              | 1.22 (8)                |
|                             |          |                    | -16.20 (2)                               | 17:04:07.87 (2)            | -42:18:39.4 (1)                      | 0.91 (5)                              | 1.76 (4)                |
|                             |          | 44                 | -20.3 (2)                                | 17:04:07.7 (1)             | -42:18:39.7 (6)                      | 8.0 (4)                               | 0.36 (1)                |

**Table 3** – *continued*

| Source name                 | Location | Frequency<br>(GHz) | LSR<br>velocity<br>(km s <sup>-1</sup> ) | $\alpha_{2000}$<br>(h:m:s) | $\delta_{2000}$<br>(°:arcmin:arcsec) | Line<br>FWHM<br>(km s <sup>-1</sup> ) | Flux<br>density<br>(Jy) |
|-----------------------------|----------|--------------------|------------------------------------------|----------------------------|--------------------------------------|---------------------------------------|-------------------------|
| G344.23-0.57<br>(continued) | I        | 44                 | -17.09 (1)                               | 17:04:07.89 (2)            | -42:18:39.2 (2)                      | 0.42 (4)                              | 1.6 (2)                 |
|                             |          |                    | -16.57 (6)                               | 17:04:07.85 (3)            | -42:18:39.0 (3)                      | 1.12 (9)                              | 1.19 (8)                |
|                             | J        | 36                 | -20.296 (5)                              | 17:04:06.527 (8)           | -42:17:40.57 (6)                     | 0.48 (1)                              | 10.5 (3)                |
|                             |          |                    | -20.57 (1)                               | 17:04:06.50 (2)            | -42:17:41.6 (2)                      | 0.51 (2)                              | 18.6 (8)                |
|                             | K        | 44                 | -22.57 (1)                               | 17:04:10.57 (2)            | -42:19:00.9 (2)                      | 0.46 (4)                              | 2.3 (1)                 |
| G345.00-0.22                | L        | 44                 | -22.21 (2)                               | 17:04:08.27 (4)            | -42:18:30.8 (3)                      | 0.51 (4)                              | 0.90 (6)                |
|                             |          |                    | -29.7 (1)                                | 17:05:11.10 (6)            | -41:29:20.4 (4)                      | 1.7 (3)                               | 0.56 (4)                |
|                             | A        | 36                 | -29.075 (7)                              | 17:05:11.01 (5)            | -41:29:20.2 (3)                      | 0.16 (2)                              | 1.7 (2)                 |
|                             |          |                    | -28.744 (6)                              | 17:05:11.062 (3)           | -41:29:20.40 (2)                     | 0.42 (3)                              | 4.2 (1)                 |
|                             |          |                    | -28.28 (1)                               | 17:05:10.92 (3)            | -41:29:21.2 (1)                      | 0.31 (3)                              | 2.5 (1)                 |
|                             |          |                    | -27.877 (1)                              | 17:05:11.113 (2)           | -41:29:19.84 (1)                     | 0.226 (2)                             | 30.5 (3)                |
|                             |          |                    | -27.56 (2)                               | 17:05:11.08 (2)            | -41:29:19.6 (1)                      | 0.42 (5)                              | 2.77 (8)                |
|                             |          |                    | -26.99 (4)                               | 17:05:11.01 (5)            | -41:29:20.5 (3)                      | 0.3 (1)                               | 0.43 (8)                |
|                             |          | 44                 | -30.2 (1)                                | 17:05:11.08 (2)            | -41:29:20.7 (1)                      | 1.2 (2)                               | 1.9 (1)                 |
|                             |          |                    | -29.722 (4)                              | 17:05:11.078 (3)           | -41:29:20.64 (3)                     | 0.37 (2)                              | 7.6 (4)                 |
|                             |          |                    | -29.275 (6)                              | 17:05:10.93 (1)            | -41:29:20.63 (8)                     | 0.28 (1)                              | 11.7 (5)                |
|                             |          |                    | -28.947 (4)                              | 17:05:11.03 (1)            | -41:29:20.5 (1)                      | 0.34 (1)                              | 21.6 (3)                |
|                             |          |                    | -28.469 (3)                              | 17:05:11.01 (6)            | -41:29:21.0 (5)                      | 0.44 (1)                              | 22.9 (1)                |
|                             |          |                    | -28.057 (1)                              | 17:05:11.107 (4)           | -41:29:19.97 (4)                     | 0.254 (2)                             | 69.7 (3)                |
|                             |          |                    | -27.737 (3)                              | 17:05:11.091 (9)           | -41:29:19.56 (8)                     | 0.298 (9)                             | 18.6 (6)                |
|                             |          |                    | -27.36 (4)                               | 17:05:10.85 (3)            | -41:29:21.4 (2)                      | 0.69 (8)                              | 3.8 (2)                 |
|                             | B        | 36                 | -29.28 (1)                               | 17:05:12.45 (3)            | -41:29:29.5 (2)                      | 0.38 (3)                              | 2.3 (1)                 |
|                             |          |                    | -29.47 (1)                               | 17:05:12.45 (2)            | -41:29:29.5 (2)                      | 0.32 (3)                              | 4.1 (3)                 |
|                             | C        | 36                 | -23.69 (1)                               | 17:05:10.71 (2)            | -41:28:58.4 (1)                      | 0.96 (3)                              | 1.53 (4)                |
|                             |          |                    | -27.20 (1)                               | 17:05:10.99 (2)            | -41:28:58.1 (2)                      | 0.83 (3)                              | 2.60 (8)                |
|                             |          | 44                 | -26.25 (3)                               | 17:05:11.01 (3)            | -41:28:57.5 (3)                      | 0.43 (8)                              | 0.8 (1)                 |
|                             |          |                    | -24.347 (4)                              | 17:05:10.681 (6)           | -41:28:57.75 (5)                     | 0.24 (1)                              | 8.9 (5)                 |
|                             |          |                    | -24.13 (8)                               | 17:05:10.60 (3)            | -41:28:56.3 (3)                      | 1.01 (6)                              | 8 (1)                   |
|                             |          |                    | -23.972 (5)                              | 17:05:10.66 (4)            | -41:28:57.7 (3)                      | 0.46 (2)                              | 16 (1)                  |
|                             |          |                    | -23.48 (1)                               | 17:05:10.67 (5)            | -41:28:57.8 (4)                      | 0.47 (3)                              | 10 (1)                  |
|                             |          |                    | -26.39 (1)                               | 17:05:09.32 (4)            | -41:29:21.6 (2)                      | 0.63 (3)                              | 1.40 (6)                |
|                             | D        | 36                 | -17.14 (8)                               | 17:05:09.36 (8)            | -41:29:17.7 (5)                      | 1.2 (2)                               | 0.37 (4)                |
|                             |          |                    | -26.51 (2)                               | 17:05:09.29 (2)            | -41:29:21.0 (1)                      | 0.76 (4)                              | 1.76 (8)                |
|                             | E        | 36                 | -26.38 (1)                               | 17:05:08.99 (3)            | -41:29:08.1 (2)                      | 0.40 (3)                              | 1.06 (6)                |
|                             |          |                    | -25.75 (1)                               | 17:05:09.06 (3)            | -41:29:07.1 (2)                      | 0.47 (3)                              | 1.20 (6)                |
| G345.01+1.79                | A        | 36                 | -15.04 (3)                               | 16:56:47.03 (6)            | -40:14:12.1 (4)                      | 0.73 (5)                              | 1.5 (1)                 |
|                             |          |                    | -14.912 (1)                              | 16:56:47.198 (3)           | -40:14:08.88 (3)                     | 0.218 (2)                             | 16.3 (1)                |
|                             |          |                    | -13.97 (1)                               | 16:56:47.18 (2)            | -40:14:09.6 (2)                      | 0.84 (5)                              | 2.26 (5)                |
|                             |          |                    | -13.243 (5)                              | 16:56:47.07 (2)            | -40:14:10.3 (2)                      | 0.35 (1)                              | 4.0 (1)                 |
|                             |          |                    | -12.896 (3)                              | 16:56:47.00 (1)            | -40:14:10.8 (1)                      | 0.203 (7)                             | 4.7 (1)                 |
|                             |          |                    | -12.42 (6)                               | 16:56:47.33 (3)            | -40:14:09.6 (3)                      | 1.3 (1)                               | 1.05 (4)                |
|                             |          | 44                 | -15.115 (2)                              | 16:56:47.172 (8)           | -40:14:08.69 (6)                     | 0.282 (4)                             | 9.7 (1)                 |
|                             |          |                    | -14.202 (6)                              | 16:56:47.13 (3)            | -40:14:09.6 (2)                      | 0.72 (1)                              | 4.57 (6)                |
|                             |          |                    | -14.01 (2)                               | 16:56:46.85 (6)            | -40:14:10.9 (5)                      | 0.28 (2)                              | 4.5 (2)                 |
|                             |          |                    | -13.764 (7)                              | 16:56:46.77 (2)            | -40:14:11.1 (1)                      | 0.21 (2)                              | 8 (1)                   |
|                             |          |                    | -13.522 (8)                              | 16:56:46.93 (2)            | -40:14:10.6 (2)                      | 0.33 (1)                              | 15.1 (3)                |
|                             |          |                    | -13.103 (2)                              | 16:56:46.947 (4)           | -40:14:10.92 (3)                     | 0.210 (4)                             | 13.3 (2)                |
|                             |          |                    | -12.54 (3)                               | 16:56:47.13 (3)            | -40:14:10.5 (2)                      | 0.79 (5)                              | 2.1 (1)                 |



Table 3 – continued

| Source name                 | Location | Frequency<br>(GHz) | LSR<br>velocity<br>(km s <sup>-1</sup> ) | $\alpha_{2000}$<br>(h:m:s) | $\delta_{2000}$<br>(°:arcmin:arcsec) | Line<br>FWHM<br>(km s <sup>-1</sup> ) | Flux<br>density<br>(Jy) |
|-----------------------------|----------|--------------------|------------------------------------------|----------------------------|--------------------------------------|---------------------------------------|-------------------------|
| G345.01+1.79<br>(continued) | A        | 44                 | -12.245 (8)                              | 16:56:47.18 (2)            | -40:14:10.0 (1)                      | 0.22 (2)                              | 2.2 (2)                 |
|                             | B        | 44                 | -14.916 (2)                              | 16:56:46.735 (6)           | -40:14:02.97 (5)                     | 0.281 (3)                             | 12.9 (1)                |
|                             |          |                    | -14.420 (4)                              | 16:56:46.75 (2)            | -40:14:03.6 (1)                      | 0.27 (1)                              | 4.6 (2)                 |
|                             | C        | 36                 | -13.26 (5)                               | 16:56:46.05 (6)            | -40:14:18.5 (5)                      | 1.8 (1)                               | 0.73 (8)                |
|                             |          |                    | -13.110 (1)                              | 16:56:46.064 (5)           | -40:14:19.53 (4)                     | 0.195 (2)                             | 23.5 (4)                |
|                             |          |                    | -12.991 (5)                              | 16:56:46.096 (7)           | -40:14:19.24 (6)                     | 0.415 (6)                             | 11.6 (3)                |
|                             |          | 44                 | -13.42 (3)                               | 16:56:45.95 (5)            | -40:14:19.8 (4)                      | 1.83 (9)                              | 2.5 (2)                 |
|                             |          |                    | -13.339 (1)                              | 16:56:46.021 (7)           | -40:14:19.41 (5)                     | 0.231 (3)                             | 62 (2)                  |
|                             |          |                    | -13.181 (6)                              | 16:56:46.043 (5)           | -40:14:19.25 (4)                     | 0.417 (6)                             | 43 (1)                  |
|                             | D        | 44                 | -12.555 (9)                              | 16:56:45.13 (3)            | -40:13:51.2 (2)                      | 0.58 (2)                              | 10.2 (3)                |
|                             | E        | 44                 | -15.765 (9)                              | 16:56:44.93 (4)            | -40:14:11.4 (3)                      | 0.20 (2)                              | 4.1 (4)                 |
|                             | F        | 44                 | -17.34 (1)                               | 16:56:46.91 (5)            | -40:14:27.6 (4)                      | 0.29 (3)                              | 0.91 (9)                |
|                             | G        | 36                 | -13.995 (8)                              | 16:56:44.68 (2)            | -40:13:55.7 (2)                      | 0.20 (2)                              | 2.9 (2)                 |
|                             |          |                    | -13.8 (1)                                | 16:56:44.84 (9)            | -40:13:54.7 (8)                      | 3.9 (3)                               | 0.81 (6)                |
| G345.42-0.95                | A        | 44                 | -24.101 (7)                              | 17:09:36.68 (2)            | -41:35:52.5 (1)                      | 0.45 (2)                              | 5.7 (2)                 |
|                             | B        | 36                 | -22.649 (9)                              | 17:09:33.24 (2)            | -41:36:19.0 (2)                      | 0.46 (2)                              | 3.0 (1)                 |
|                             |          | 44                 | -22.982 (5)                              | 17:09:33.22 (1)            | -41:36:18.9 (1)                      | 0.70 (1)                              | 17.1 (2)                |
|                             | C        | 36                 | -17.63 (2)                               | 17:09:37.96 (4)            | -41:35:00.7 (3)                      | 0.52 (5)                              | 2.4 (2)                 |
|                             |          | 44                 | -18.01 (1)                               | 17:09:37.94 (3)            | -41:35:01.5 (2)                      | 0.70 (3)                              | 11.9 (5)                |
| G345.50+0.35                | A        | 36                 | -16.24 (1)                               | 17:04:24.37 (4)            | -40:44:30.2 (3)                      | 0.16 (3)                              | 0.8 (1)                 |
|                             |          | 44                 | -18.16 (1)                               | 17:04:24.51 (1)            | -40:44:31.4 (1)                      | 0.39 (3)                              | 1.8 (1)                 |
|                             |          |                    | -17.33 (2)                               | 17:04:24.51 (3)            | -40:44:31.1 (3)                      | 0.81 (8)                              | 1.41 (8)                |
|                             |          |                    | -16.515 (3)                              | 17:04:24.364 (9)           | -40:44:29.70 (8)                     | 0.214 (6)                             | 5.2 (1)                 |
|                             |          |                    | -15.93 (1)                               | 17:04:24.12 (6)            | -40:44:31.5 (5)                      | 0.17 (3)                              | 0.9 (1)                 |
|                             | B        | 36                 | -16.32 (2)                               | 17:04:21.39 (3)            | -40:44:18.0 (2)                      | 0.59 (4)                              | 0.90 (6)                |
|                             |          | 44                 | -16.679 (3)                              | 17:04:21.360 (4)           | -40:44:17.91 (4)                     | 0.369 (6)                             | 13.3 (1)                |
|                             |          |                    | -16.274 (7)                              | 17:04:21.36 (1)            | -40:44:18.3 (1)                      | 0.34 (1)                              | 5.4 (1)                 |
|                             | C        | 36                 | -15.195 (7)                              | 17:04:25.79 (2)            | -40:43:42.8 (1)                      | 0.66 (2)                              | 3.95 (8)                |
|                             |          |                    | -14.43 (2)                               | 17:04:25.90 (3)            | -40:43:43.5 (2)                      | 0.41 (5)                              | 1.1 (1)                 |
|                             |          | 44                 | -15.45 (1)                               | 17:04:25.74 (2)            | -40:43:42.8 (2)                      | 0.55 (3)                              | 2.5 (1)                 |
|                             | D        | 44                 | -14.73 (2)                               | 17:04:22.59 (3)            | -40:44:24.4 (2)                      | 0.50 (6)                              | 0.64 (6)                |
|                             | E        | 44                 | -16.99 (8)                               | 17:04:26.81 (8)            | -40:44:10.6 (7)                      | 2.0 (2)                               | 1.05 (9)                |
|                             |          |                    | -16.90 (2)                               | 17:04:26.74 (1)            | -40:44:10.8 (1)                      | 0.22 (4)                              | 1.4 (2)                 |
| G348.18+0.48                | A        | 36                 | -7.15 (4)                                | 17:12:08.76 (2)            | -38:30:58.0 (2)                      | 0.64 (3)                              | 8.5 (9)                 |
|                             |          |                    | -7.060 (1)                               | 17:12:08.681 (2)           | -38:30:57.12 (2)                     | 0.253 (3)                             | 40.9 (7)                |
|                             |          |                    | -6.5 (2)                                 | 17:12:08.70 (3)            | -38:30:57.0 (3)                      | 0.7 (2)                               | 1.6 (4)                 |
|                             |          | 44                 | -7.7 (2)                                 | 17:12:08.81 (3)            | -38:30:57.9 (3)                      | 1.0 (2)                               | 8 (2)                   |
|                             |          |                    | -7.38 (2)                                | 17:12:08.72 (1)            | -38:30:57.3 (1)                      | 0.40 (3)                              | 31 (5)                  |
|                             |          |                    | -7.284 (2)                               | 17:12:08.70 (1)            | -38:30:57.0 (1)                      | 0.211 (6)                             | 65 (4)                  |
|                             | B        |                    | -6.6 (2)                                 | 17:12:08.67 (5)            | -38:30:57.1 (4)                      | 0.7 (2)                               | 3 (1)                   |
|                             |          | 36                 | -6.62 (1)                                | 17:12:08.67 (3)            | -38:30:50.0 (3)                      | 0.46 (3)                              | 3.6 (1)                 |
|                             |          |                    | -6.15 (2)                                | 17:12:08.67 (6)            | -38:30:51.0 (5)                      | 0.31 (4)                              | 1.6 (2)                 |
|                             |          | 44                 | -6.875 (5)                               | 17:12:08.70 (2)            | -38:30:48.7 (2)                      | 0.15 (1)                              | 7.7 (5)                 |
|                             |          | 36                 | -6.5 (1)                                 | 17:12:08.6 (1)             | -38:30:47 (1)                        | 0.6 (2)                               | 1.0 (2)                 |
|                             | C        |                    | -6.13 (3)                                | 17:12:08.58 (6)            | -38:30:44.9 (6)                      | 0.33 (5)                              | 2.0 (5)                 |
|                             |          | 44                 | -6.40 (2)                                | 17:12:08.43 (2)            | -38:30:44.6 (2)                      | 0.56 (4)                              | 4.0 (2)                 |
|                             | D        | 44                 | -6.45 (1)                                | 17:12:05.20 (3)            | -38:30:49.3 (2)                      | 0.42 (3)                              | 1.11 (8)                |
|                             | E        | 36                 | -5.719 (7)                               | 17:12:05.22 (2)            | -38:31:11.4 (2)                      | 0.29 (2)                              | 1.9 (1)                 |

**Table 3** – *continued*

| Source name                 | Location | Frequency<br>(GHz) | LSR<br>velocity<br>(km s <sup>-1</sup> ) | $\alpha_{2000}$<br>(h:m:s) | $\delta_{2000}$<br>(°:arcmin:arcsec) | Line<br>FWHM<br>(km s <sup>-1</sup> ) | Flux<br>density<br>(Jy) |
|-----------------------------|----------|--------------------|------------------------------------------|----------------------------|--------------------------------------|---------------------------------------|-------------------------|
| G348.18+0.48<br>(continued) | E        | 44                 | −5.960 (4)                               | 17:12:05.178 (7)           | −38:31:11.37 (6)                     | 0.44 (1)                              | 6.6 (1)                 |
|                             | F        | 44                 | −7.77 (1)                                | 17:12:08.64 (3)            | −38:30:04.8 (2)                      | 0.52 (3)                              | 13.1 (7)                |
|                             | G        | 44                 | −7.66 (3)                                | 17:12:06.08 (3)            | −38:30:36.1 (3)                      | 0.65 (9)                              | 0.77 (8)                |
|                             | H        | 36                 | −5.05 (1)                                | 17:12:06.70 (3)            | −38:30:48.3 (3)                      | 0.49 (2)                              | 1.32 (5)                |
|                             | I        | 36                 | −8.28 (3)                                | 17:12:04.72 (5)            | −38:30:52.5 (5)                      | 0.89 (8)                              | 0.48 (3)                |
| G349.09+0.11                | A        | 36                 | −80.03 (1)                               | 17:16:24.44 (2)            | −37:59:39.3 (2)                      | 0.25 (4)                              | 1.1 (1)                 |
|                             |          |                    | −79.17 (2)                               | 17:16:24.31 (4)            | −37:59:41.4 (3)                      | 0.47 (8)                              | 0.9 (1)                 |
|                             |          |                    | −78.1 (1)                                | 17:16:24.5 (1)             | −37:59:40.6 (8)                      | 3.0 (3)                               | 0.70 (9)                |
|                             |          |                    | −77.925 (2)                              | 17:16:24.534 (7)           | −37:59:37.38 (6)                     | 0.489 (5)                             | 14.2 (1)                |
|                             |          |                    | −77.29 (1)                               | 17:16:24.59 (4)            | −37:59:38.1 (3)                      | 0.24 (3)                              | 1.5 (1)                 |
|                             |          | 44                 | −79.480 (4)                              | 17:16:24.318 (9)           | −37:59:41.49 (8)                     | 0.33 (1)                              | 12.4 (4)                |
|                             |          |                    | −78.9 (1)                                | 17:16:24.31 (5)            | −37:59:41.9 (4)                      | 1.2 (2)                               | 3.1 (2)                 |
|                             | B        | 36                 | −78.129 (2)                              | 17:16:24.534 (7)           | −37:59:37.31 (5)                     | 0.477 (8)                             | 31.4 (6)                |
|                             |          |                    | −77.36 (1)                               | 17:16:24.54 (2)            | −37:59:37.7 (1)                      | 0.34 (3)                              | 4.3 (3)                 |
|                             |          |                    | −76.71 (2)                               | 17:16:24.97 (6)            | −37:59:48.5 (5)                      | 1.42 (6)                              | 1.46 (5)                |
|                             |          | 44                 | −76.390 (7)                              | 17:16:24.94 (3)            | −37:59:47.0 (2)                      | 0.20 (2)                              | 4.8 (4)                 |
|                             |          |                    |                                          |                            |                                      |                                       |                         |
|                             | A        | 36                 | −7.99 (1)                                | 17:19:55.29 (3)            | −35:57:38.6 (3)                      | 0.53 (2)                              | 1.71 (6)                |
|                             |          |                    | −7.849 (1)                               | 17:19:55.31 (2)            | −35:57:38.1 (2)                      | 0.283 (2)                             | 31.0 (1)                |
|                             |          |                    | −7.463 (3)                               | 17:19:55.09 (3)            | −35:57:36.5 (3)                      | 0.279 (5)                             | 25.3 (5)                |
|                             |          |                    | −7.140 (9)                               | 17:19:55.228 (6)           | −35:57:37.21 (6)                     | 0.36 (2)                              | 18.5 (4)                |
|                             |          |                    | −6.956 (3)                               | 17:19:55.28 (1)            | −35:57:38.6 (1)                      | 0.18 (1)                              | 7 (1)                   |
|                             |          |                    | −5.625 (3)                               | 17:19:54.780 (7)           | −35:57:39.45 (8)                     | 0.410 (6)                             | 6.78 (9)                |
|                             |          |                    | −4.56 (3)                                | 17:19:54.28 (4)            | −35:57:38.7 (4)                      | 1.25 (8)                              | 1.31 (5)                |
|                             |          | 44                 | −8.337 (9)                               | 17:19:55.32 (2)            | −35:57:38.1 (1)                      | 0.22 (2)                              | 3.2 (2)                 |
|                             |          |                    | −8.068 (1)                               | 17:19:55.28 (1)            | −35:57:37.89 (8)                     | 0.275 (2)                             | 58.5 (2)                |
|                             |          |                    | −7.662 (2)                               | 17:19:55.07 (1)            | −35:57:36.61 (8)                     | 0.229 (3)                             | 33.1 (3)                |
|                             |          |                    | −7.328 (4)                               | 17:19:55.220 (8)           | −35:57:37.20 (6)                     | 0.337 (7)                             | 33.6 (4)                |
|                             |          |                    | −7.169 (2)                               | 17:19:55.28 (2)            | −35:57:38.1 (1)                      | 0.146 (8)                             | 11.6 (8)                |
|                             |          | 36                 | −6.852 (7)                               | 17:19:54.36 (1)            | −35:57:57.0 (1)                      | 0.42 (1)                              | 10.9 (2)                |
|                             |          |                    | −6.408 (2)                               | 17:19:54.405 (2)           | −35:57:57.20 (2)                     | 0.394 (8)                             | 27.7 (1)                |
|                             |          |                    | −6.091 (4)                               | 17:19:54.395 (7)           | −35:57:57.33 (8)                     | 0.212 (8)                             | 6.5 (3)                 |
|                             | B        | 44                 | −6.800 (8)                               | 17:19:54.392 (7)           | −35:57:57.55 (5)                     | 0.71 (1)                              | 47.1 (5)                |
|                             |          |                    | −6.610 (1)                               | 17:19:54.395 (2)           | −35:57:57.42 (2)                     | 0.210 (4)                             | 34 (1)                  |
|                             |          |                    | −6.272 (2)                               | 17:19:54.405 (3)           | −35:57:57.32 (2)                     | 0.333 (3)                             | 62 (1)                  |
|                             |          |                    | −5.992 (2)                               | 17:19:54.023 (5)           | −35:57:48.87 (6)                     | 0.255 (9)                             | 9.2 (5)                 |
|                             |          | 36                 | −5.73 (2)                                | 17:19:54.19 (2)            | −35:57:48.0 (2)                      | 0.59 (3)                              | 6.5 (2)                 |
|                             |          |                    | −5.12 (2)                                | 17:19:54.23 (3)            | −35:57:47.8 (3)                      | 0.28 (5)                              | 0.8 (1)                 |
|                             |          |                    | −4.36 (1)                                | 17:19:54.70 (1)            | −35:57:47.7 (1)                      | 0.36 (2)                              | 1.72 (9)                |
|                             |          | 44                 | −5.759 (5)                               | 17:19:54.23 (1)            | −35:57:47.65 (9)                     | 0.43 (1)                              | 6.9 (1)                 |
|                             |          |                    | −5.830 (2)                               | 17:19:58.692 (4)           | −35:57:46.89 (3)                     | 0.295 (3)                             | 12.6 (1)                |
|                             |          |                    | −5.012 (1)                               | 17:19:57.275 (1)           | −35:57:58.49 (1)                     | 0.315 (1)                             | 27.6 (1)                |
|                             | F        | 36                 | −6.739 (7)                               | 17:19:55.20 (2)            | −35:58:11.7 (3)                      | 0.16 (2)                              | 1.4 (1)                 |
|                             |          |                    | −6.140 (3)                               | 17:19:55.256 (7)           | −35:58:10.49 (8)                     | 0.227 (8)                             | 5.0 (1)                 |
| G351.24+0.67                | A        | 44                 | −4.785 (3)                               | 17:20:17.624 (6)           | −35:54:48.44 (8)                     | 0.251 (8)                             | 5.9 (2)                 |
|                             |          |                    | −4.45 (1)                                | 17:20:17.67 (5)            | −35:54:48.0 (6)                      | 0.12 (3)                              | 1.1 (2)                 |
|                             | B        | 36                 | −3.62 (2)                                | 17:20:17.77 (3)            | −35:54:42.2 (2)                      | 0.83 (2)                              | 2.5 (1)                 |
|                             |          |                    | −3.418 (7)                               | 17:20:17.748 (9)           | −35:54:41.89 (8)                     | 0.32 (2)                              | 2.2 (2)                 |
|                             |          |                    | −5.3 (1)                                 | 17:20:17.73 (6)            | −35:54:41.5 (7)                      | 0.8 (3)                               | 0.6 (1)                 |

Table 3 – continued

| Source name                 | Location | Frequency<br>(GHz) | LSR<br>velocity<br>(km s <sup>-1</sup> ) | $\alpha_{2000}$<br>(h:m:s) | $\delta_{2000}$<br>(°:arcmin:arcsec) | Line<br>FWHM<br>(km s <sup>-1</sup> ) | Flux<br>density<br>(Jy) |
|-----------------------------|----------|--------------------|------------------------------------------|----------------------------|--------------------------------------|---------------------------------------|-------------------------|
| G351.24+0.67<br>(continued) | B        | 44                 | -4.616 (6)                               | 17:20:17.69 (2)            | -35:54:42.2 (2)                      | 0.30 (1)                              | 9.4 (3)                 |
|                             |          |                    | -4.179 (3)                               | 17:20:17.742 (4)           | -35:54:42.03 (4)                     | 0.402 (8)                             | 25.3 (2)                |
|                             |          |                    | -3.610 (1)                               | 17:20:17.742 (2)           | -35:54:42.14 (2)                     | 0.412 (2)                             | 70.3 (2)                |
|                             | C        | 36                 | -2.43 (1)                                | 17:20:18.35 (2)            | -35:54:41.0 (2)                      | 0.33 (2)                              | 1.51 (9)                |
|                             |          | 44                 | -2.632 (1)                               | 17:20:18.346 (2)           | -35:54:40.83 (2)                     | 0.316 (3)                             | 29.6 (2)                |
| G351.42+0.65                | A        | 36                 | -9.92 (3)                                | 17:20:52.72 (3)            | -35:47:05.9 (3)                      | 1.07 (5)                              | 2.12 (4)                |
|                             |          |                    | -9.41 (3)                                | 17:20:52.66 (3)            | -35:47:06.5 (3)                      | 0.33 (8)                              | 0.9 (4)                 |
|                             |          |                    | -9.08 (6)                                | 17:20:52.75 (4)            | -35:47:05.4 (4)                      | 0.56 (8)                              | 1.6 (2)                 |
|                             |          |                    | -7.1 (2)                                 | 17:20:53.1 (1)             | -35:46:59 (1)                        | 2.7 (4)                               | 0.20 (3)                |
|                             |          |                    | -6.14 (2)                                | 17:20:52.93 (8)            | -35:46:59.4 (8)                      | 0.64 (6)                              | 0.56 (5)                |
|                             |          | 44                 | -10.28 (3)                               | 17:20:52.82 (2)            | -35:47:06.5 (2)                      | 1.54 (6)                              | 1.18 (5)                |
|                             |          |                    | -9.995 (4)                               | 17:20:52.91 (1)            | -35:47:00.7 (1)                      | 0.27 (1)                              | 2.85 (9)                |
|                             |          |                    | -9.037 (3)                               | 17:20:52.972 (6)           | -35:47:01.50 (6)                     | 0.256 (6)                             | 4.44 (9)                |
|                             |          |                    | -6.63 (1)                                | 17:20:52.745 (2)           | -35:47:00.58 (2)                     | 0.32 (1)                              | 6.3 (4)                 |
|                             |          |                    | -6.319 (8)                               | 17:20:52.748 (5)           | -35:47:00.37 (4)                     | 0.40 (1)                              | 10.3 (2)                |
|                             | B        | 36                 | -8.56 (1)                                | 17:20:49.828 (7)           | -35:46:49.03 (8)                     | 0.33 (2)                              | 11.6 (4)                |
|                             |          |                    | -8.264 (7)                               | 17:20:49.833 (3)           | -35:46:48.88 (3)                     | 0.28 (2)                              | 13.2 (7)                |
|                             |          |                    | -7.870 (3)                               | 17:20:49.87 (2)            | -35:46:48.5 (2)                      | 0.473 (6)                             | 32.9 (2)                |
|                             |          |                    | -6.953 (6)                               | 17:20:50.197 (6)           | -35:46:48.00 (8)                     | 0.49 (1)                              | 5.8 (1)                 |
|                             |          |                    | -8.656 (6)                               | 17:20:49.805 (5)           | -35:46:49.25 (4)                     | 0.69 (1)                              | 59.2 (7)                |
|                             |          | 44                 | -8.071 (2)                               | 17:20:49.86 (2)            | -35:46:48.7 (2)                      | 0.185 (6)                             | 22.8 (7)                |
|                             |          |                    | -8.018 (6)                               | 17:20:49.806 (6)           | -35:46:48.99 (6)                     | 0.612 (9)                             | 53 (1)                  |
|                             |          |                    | -7.152 (3)                               | 17:20:50.195 (5)           | -35:46:48.09 (5)                     | 0.249 (7)                             | 14.8 (4)                |
|                             |          | 36                 | -5.18 (2)                                | 17:20:54.54 (2)            | -35:46:46.3 (2)                      | 0.37 (6)                              | 0.58 (8)                |
|                             |          |                    | -6.989 (2)                               | 17:20:54.648 (2)           | -35:46:45.11 (2)                     | 0.510 (4)                             | 21.11 (8)               |
|                             | C        | 44                 | -6.429 (3)                               | 17:20:54.646 (4)           | -35:46:45.03 (4)                     | 0.449 (5)                             | 15.1 (1)                |
|                             |          |                    | -5.829 (3)                               | 17:20:54.88 (1)            | -35:46:47.5 (1)                      | 0.184 (6)                             | 5.0 (1)                 |
|                             |          |                    | -5.341 (2)                               | 17:20:54.607 (5)           | -35:46:45.69 (4)                     | 0.388 (4)                             | 10.72 (9)               |
|                             |          |                    | -3.085 (8)                               | 17:20:54.55 (2)            | -35:46:43.5 (2)                      | 0.42 (2)                              | 2.35 (9)                |
|                             |          |                    | -9.273 (4)                               | 17:20:50.75 (1)            | -35:46:18.1 (1)                      | 0.322 (8)                             | 25.7 (6)                |
|                             |          | 36                 | -10.9 (1)                                | 17:20:53.24 (4)            | -35:46:59.6 (5)                      | 1.6 (2)                               | 0.43 (3)                |
|                             |          |                    | -9.1 (1)                                 | 17:20:53.21 (9)            | -35:46:59.5 (9)                      | 1.6 (3)                               | 0.33 (3)                |
|                             |          |                    | -7.33 (2)                                | 17:20:53.30 (3)            | -35:46:57.7 (3)                      | 0.50 (6)                              | 0.54 (6)                |
|                             |          |                    | -6.30 (3)                                | 17:20:53.35 (2)            | -35:46:57.6 (2)                      | 1.66 (8)                              | 1.07 (2)                |
|                             |          |                    | -16.332 (1)                              | 17:29:18.372 (1)           | -36:40:24.18 (1)                     | 0.333 (2)                             | 14.15 (9)               |
| G351.63-1.26                | A        | 44                 | -15.2 (1)                                | 17:29:18.25 (8)            | -36:40:24.4 (6)                      | 3.2 (2)                               | 0.45 (3)                |
|                             |          |                    | -14.65 (1)                               | 17:29:18.26 (1)            | -36:40:23.0 (1)                      | 0.18 (3)                              | 0.9 (1)                 |
|                             |          |                    | -13.89 (1)                               | 17:29:18.28 (3)            | -36:40:22.2 (2)                      | 0.52 (3)                              | 1.56 (8)                |
|                             | B        | 36                 | -12.81 (1)                               | 17:29:17.397 (4)           | -36:40:35.69 (3)                     | 0.74 (2)                              | 10.0 (2)                |
|                             |          |                    | -12.457 (2)                              | 17:29:17.408 (4)           | -36:40:35.77 (4)                     | 0.41 (1)                              | 10.4 (5)                |
|                             |          | 44                 | -13.206 (7)                              | 17:29:17.393 (5)           | -36:40:35.51 (4)                     | 0.81 (1)                              | 21.9 (1)                |
| G351.77-0.54                | A        | 36                 | -12.668 (2)                              | 17:29:17.395 (5)           | -36:40:35.61 (5)                     | 0.462 (4)                             | 28.4 (4)                |
|                             |          |                    | -8.17 (3)                                | 17:26:42.90 (4)            | -36:09:03.5 (3)                      | 0.66 (6)                              | 0.74 (6)                |
|                             |          |                    | -7.192 (6)                               | 17:26:42.888 (4)           | -36:09:03.16 (3)                     | 0.41 (1)                              | 7.22 (8)                |
|                             |          | 44                 | -6.801 (1)                               | 17:26:42.885 (1)           | -36:09:03.158 (5)                    | 0.322 (2)                             | 29.3 (1)                |
|                             |          |                    | -9.378 (5)                               | 17:26:42.841 (4)           | -36:09:03.76 (3)                     | 0.33 (1)                              | 9.1 (2)                 |
|                             |          |                    | -8.5 (1)                                 | 17:26:42.877 (5)           | -36:09:03.75 (4)                     | 0.6 (1)                               | 22 (1)                  |
|                             |          |                    | -8.25 (2)                                | 17:26:42.863 (2)           | -36:09:03.73 (2)                     | 0.45 (8)                              | 18 (3)                  |

**Table 3** – *continued*

| Source name                 | Location | Frequency<br>(GHz) | LSR<br>velocity<br>(km s <sup>-1</sup> ) | $\alpha_{2000}$<br>(h:m:s) | $\delta_{2000}$<br>(°:arcmin:arcsec) | Line<br>FWHM<br>(km s <sup>-1</sup> ) | Flux<br>density<br>(Jy) |
|-----------------------------|----------|--------------------|------------------------------------------|----------------------------|--------------------------------------|---------------------------------------|-------------------------|
| G351.77-0.54<br>(continued) | A        | 44                 | -7.486 (3)                               | 17:26:42.843 (1)           | -36:09:03.37 (1)                     | 0.521 (5)                             | 74.3 (3)                |
|                             |          |                    | -7.009 (1)                               | 17:26:42.842 (1)           | -36:09:03.28 (1)                     | 0.421 (2)                             | 140.6 (5)               |
|                             |          |                    | -6.41 (1)                                | 17:26:42.85 (1)            | -36:09:03.3 (1)                      | 0.19 (3)                              | 2.4 (3)                 |
|                             | B        | 36                 | -8.62 (1)                                | 17:26:42.43 (2)            | -36:09:16.6 (2)                      | 0.37 (4)                              | 0.82 (8)                |
|                             |          |                    | -7.5 (1)                                 | 17:26:42.66 (3)            | -36:09:17.1 (2)                      | 1.1 (3)                               | 0.6 (2)                 |
|                             |          |                    | -7.3 (8)                                 | 17:26:42.62 (8)            | -36:09:16.8 (7)                      | 4.1 (7)                               | 0.8 (3)                 |
|                             |          |                    | -6.29 (3)                                | 17:26:42.58 (2)            | -36:09:16.6 (2)                      | 0.6 (2)                               | 0.6 (4)                 |
|                             |          |                    | -5.46 (3)                                | 17:26:42.53 (2)            | -36:09:17.3 (1)                      | 0.6 (2)                               | 0.6 (4)                 |
|                             |          |                    | -4.35 (8)                                | 17:26:42.56 (3)            | -36:09:17.4 (2)                      | 0.9 (2)                               | 1.0 (3)                 |
|                             |          |                    | -3.09 (4)                                | 17:26:42.54 (2)            | -36:09:18.1 (2)                      | 1.5 (2)                               | 2.0 (2)                 |
|                             |          |                    | -2.391 (5)                               | 17:26:42.51 (2)            | -36:09:17.2 (1)                      | 0.36 (2)                              | 2.5 (2)                 |
|                             |          |                    | -1.62 (2)                                | 17:26:42.52 (3)            | -36:09:16.6 (3)                      | 0.44 (8)                              | 0.8 (1)                 |
|                             |          |                    | -1.0 (2)                                 | 17:26:42.47 (3)            | -36:09:17.4 (3)                      | 3.0 (3)                               | 0.79 (4)                |
|                             |          | 44                 | -8.888 (9)                               | 17:26:42.31 (1)            | -36:09:16.1 (1)                      | 0.48 (2)                              | 2.00 (8)                |
|                             |          |                    | -6.12 (6)                                | 17:26:42.63 (5)            | -36:09:16.5 (4)                      | 2.0 (2)                               | 0.72 (4)                |
|                             |          |                    | -4.25 (2)                                | 17:26:42.46 (1)            | -36:09:17.5 (1)                      | 0.82 (8)                              | 1.76 (6)                |
|                             |          |                    | -3.630 (6)                               | 17:26:42.566 (6)           | -36:09:17.46 (5)                     | 0.34 (2)                              | 4.7 (3)                 |
|                             |          |                    | -3.08 (3)                                | 17:26:42.53 (1)            | -36:09:16.9 (1)                      | 0.72 (5)                              | 3.2 (1)                 |
|                             |          |                    | -2.659 (5)                               | 17:26:42.50 (1)            | -36:09:17.06 (9)                     | 0.442 (8)                             | 8.45 (6)                |
|                             |          |                    | -1.998 (7)                               | 17:26:42.70 (2)            | -36:09:15.9 (2)                      | 0.23 (2)                              | 2.6 (2)                 |
|                             |          |                    | -1.606 (8)                               | 17:26:42.40 (2)            | -36:09:15.8 (2)                      | 0.44 (3)                              | 3.54 (8)                |
|                             |          |                    | -0.835 (5)                               | 17:26:42.483 (8)           | -36:09:17.04 (8)                     | 0.70 (2)                              | 6.79 (8)                |
|                             |          |                    | +0.07 (1)                                | 17:26:42.473 (4)           | -36:09:17.15 (4)                     | 0.73 (2)                              | 4.28 (6)                |
|                             | C        | 36                 | -6.77 (2)                                | 17:26:44.228 (6)           | -36:09:03.47 (5)                     | 0.41 (6)                              | 1.5 (4)                 |
|                             |          |                    | -6.343 (9)                               | 17:26:44.25 (1)            | -36:09:04.95 (9)                     | 0.28 (4)                              | 2.2 (5)                 |
|                             |          |                    | -5.79 (2)                                | 17:26:44.23 (1)            | -36:09:05.6 (1)                      | 0.41 (4)                              | 2.6 (3)                 |
|                             |          | 44                 | -6.572 (3)                               | 17:26:44.200 (7)           | -36:09:05.09 (8)                     | 0.257 (7)                             | 5.9 (1)                 |
|                             |          |                    | -6.000 (2)                               | 17:26:44.170 (8)           | -36:09:05.66 (8)                     | 0.425 (4)                             | 12.7 (1)                |
|                             |          |                    | -4.954 (5)                               | 17:26:42.21 (2)            | -36:09:06.6 (2)                      | 0.32 (1)                              | 2.22 (8)                |
|                             | D        | 36                 | -3.75 (1)                                | 17:26:42.20 (2)            | -36:09:07.6 (1)                      | 0.33 (3)                              | 1.03 (8)                |
|                             |          |                    | -2.170 (1)                               | 17:26:42.253 (2)           | -36:09:10.31 (1)                     | 0.3132 (9)                            | 31.54 (8)               |
|                             |          |                    | -1.67 (1)                                | 17:26:42.33 (5)            | -36:09:13.2 (6)                      | 0.18 (3)                              | 0.7 (1)                 |
|                             |          |                    | -5.134 (2)                               | 17:26:42.186 (1)           | -36:09:06.86 (1)                     | 0.427 (4)                             | 26.6 (2)                |
|                             |          | 44                 | -4.50 (1)                                | 17:26:42.148 (4)           | -36:09:08.60 (4)                     | 0.34 (2)                              | 6.0 (2)                 |
|                             |          |                    | -4.005 (6)                               | 17:26:42.152 (3)           | -36:09:07.59 (3)                     | 0.44 (2)                              | 11.3 (2)                |
|                             |          |                    | -2.87 (8)                                | 17:26:42.19 (4)            | -36:09:12.7 (4)                      | 0.9 (2)                               | 3.2 (1)                 |
|                             |          |                    | -2.399 (1)                               | 17:26:42.213 (1)           | -36:09:10.507 (6)                    | 0.351 (2)                             | 113.0 (7)               |
|                             |          |                    | -1.933 (2)                               | 17:26:42.215 (5)           | -36:09:11.15 (4)                     | 0.184 (5)                             | 17.1 (4)                |
|                             |          |                    | -1.44 (1)                                | 17:26:42.24 (5)            | -36:09:12.8 (5)                      | 0.71 (3)                              | 10.3 (4)                |
|                             |          |                    | -0.8 (2)                                 | 17:26:42.3 (1)             | -36:09:14 (1)                        | 1.18 (9)                              | 1.4 (4)                 |
|                             |          |                    | -5.910 (5)                               | 17:26:44.39 (1)            | -36:08:51.8 (1)                      | 0.45 (1)                              | 3.22 (8)                |
|                             |          |                    | -6.169 (3)                               | 17:26:44.319 (6)           | -36:08:52.30 (6)                     | 0.475 (8)                             | 9.2 (1)                 |
|                             | F        | 36                 | -2.976 (6)                               | 17:26:39.63 (1)            | -36:09:36.1 (1)                      | 0.52 (2)                              | 4.1 (1)                 |
|                             |          | 44                 | -3.126 (4)                               | 17:26:39.63 (1)            | -36:09:36.5 (1)                      | 0.552 (8)                             | 13.5 (2)                |
|                             | G        | 36                 | -4.143 (4)                               | 17:26:40.86 (1)            | -36:09:34.66 (9)                     | 0.400 (9)                             | 3.54 (8)                |
|                             |          | 44                 | +0.35 (4)                                | 17:26:40.83 (1)            | -36:09:35.0 (1)                      | 1.21 (9)                              | 0.74 (5)                |
|                             | H        | 36                 | -5.672 (6)                               | 17:26:45.07 (3)            | -36:09:18.2 (2)                      | 0.31 (1)                              | 3.00 (8)                |
|                             |          |                    | -5.35 (1)                                | 17:26:45.11 (8)            | -36:09:18.7 (6)                      | 0.21 (3)                              | 1.1 (1)                 |
